# Supplementary material for: Analytical computation of moderate-degree fully-symmetric cubature rules on the triangle
Source: arXiv:1111.3827 ancillary file (2011-11-16)
Supplement: Supplementary file 1 [file allrules.pdf]

# List of zero-dimensional fully symmetric cubature rules on the triangle

Stefanos-Aldo Papanicolopulos*

November 16, 2011

This list is provided as *supplemental material* for the article "Analytical computation of moderate-degree fully-symmetric cubature rules on the triangle" by S.-A. Papanicolopulos. We list here all the cubature rules computed in that paper. For each rule we first list the degree $d$, the number of points $n_p$, the rule type and the rule quality. We then provide a list of the orbits, where the first column is the number of points in the orbit, the second is the weight for each integration point and the last three columns are the areal coordinates defining a point in the orbit.

$d = 1$, $n_p = 1$, type $[1, 0, 0]$, quality PI

| | | | | |
|---|---|---|---|---|
| 1 | 1.000000000000000e+00 | 3.333333333333333e-01 | 3.333333333333333e-01 | 3.333333333333333e-01 |

$d = 2$, $n_p = 3$, type $[0, 1, 0]$, quality PI

| | | | | |
|---|---|---|---|---|
| 3 | 3.333333333333333e-01 | 6.666666666666667e-01 | 1.666666666666667e-01 | 1.666666666666667e-01 |

$d = 2$, $n_p = 3$, type $[0, 1, 0]$, quality PB

| | | | | |
|---|---|---|---|---|
| 3 | 3.333333333333333e-01 | 0.000000000000000e+00 | 5.000000000000000e-01 | 5.000000000000000e-01 |

$d = 3$, $n_p = 4$, type $[1, 1, 0]$, quality NI

| | | | | |
|---|---|---|---|---|
| 1 | -5.625000000000000e-01 | 3.333333333333333e-01 | 3.333333333333333e-01 | 3.333333333333333e-01 |
| 3 | 5.208333333333333e-01 | 6.000000000000000e-01 | 2.000000000000000e-01 | 2.000000000000000e-01 |

$d = 3$, $n_p = 6$, type $[0, 0, 1]$, quality PI

| | | | | |
|---|---|---|---|---|
| 6 | 1.666666666666667e-01 | 1.090390090728772e-01 | 2.319333685530306e-01 | 6.590276223740922e-01 |

$d = 4$, $n_p = 6$, type $[0, 2, 0]$, quality PI

| | | | | |
|---|---|---|---|---|
| 3 | 2.233815896504443e-01 | 1.081030181575240e-01 | 4.459484909212380e-01 | 4.459484909212380e-01 |
| 3 | 1.099517436588788e-01 | 8.168475729758093e-01 | 9.157621351209534e-02 | 9.157621351209534e-02 |

$d = 4$, $n_p = 6$, type $[0, 2, 0]$, quality PO

| | | | | |
|---|---|---|---|---|
| 3 | 3.327551636583892e-01 | 6.612411828395935e-01 | 1.693794085802032e-01 | 1.693794085802032e-01 |
| 3 | 5.781696719470309e-04 | -1.141747329506260e+00 | 1.070873664753130e+00 | 1.070873664753130e+00 |

$d = 5$, $n_p = 7$, type $[1, 2, 0]$, quality PI

| | | | | |
|---|---|---|---|---|
| 1 | 2.250000000000000e-01 | 3.333333333333333e-01 | 3.333333333333333e-01 | 3.333333333333333e-01 |
| 3 | 1.323941527885062e-01 | 5.971587178976982e-02 | 4.701420641051151e-01 | 4.701420641051151e-01 |
| 3 | 1.259391805448272e-01 | 7.974269853530873e-01 | 1.012865073234563e-01 | 1.012865073234563e-01 |

$d = 6$, $n_p = 12$, type $[0, 2, 1]$, quality PI

| | | | | |
|---|---|---|---|---|
| 3 | 1.713331241529810e-01 | 5.611400349004341e-01 | 2.194299825497830e-01 | 2.194299825497830e-01 |
| 3 | 8.073108959303098e-02 | 3.972407177556991e-02 | 4.801379641122150e-01 | 4.801379641122150e-01 |
| 6 | 4.063455979366066e-02 | 1.937172436124079e-02 | 1.416190159239682e-01 | 8.390092597147911e-01 |

$d = 6$, $n_p = 12$, type $[0, 2, 1]$, quality PI

| | | | | |
|---|---|---|---|---|
| 3 | 1.167862757263794e-01 | 5.014265096581792e-01 | 2.492867451709104e-01 | 2.492867451709104e-01 |
| 3 | 5.084490637020682e-02 | 8.738219710169955e-01 | 6.308901449150223e-02 | 6.308901449150223e-02 |
| 6 | 8.285107561837358e-02 | 5.314504984481695e-02 | 3.103524510337844e-01 | 6.365024991213986e-01 |

*Department of Mechanics, National Technical University of Athens, Zografou 15773, Greece, email: stefanos@mechan.ntua.gr

$d = 6$, $n_p = 12$, type $[0, 2, 1]$, quality PO

| | | | | |
|---|---|---|---|---|
| 3 | 2.127201350144858e-01 | 1.131404479298898e-01 | 4.434297760350551e-01 | 4.434297760350551e-01 |
| 3 | 1.197593020220355e-01 | 8.007239089385513e-01 | 9.963804553072436e-02 | 9.963804553072436e-02 |
| 6 | 4.269481484059911e-04 | -3.916056607505046e-01 | 3.812153080251857e-01 | 1.010390352725319e+00 |

$d = 6$, $n_p = 12$, type $[0, 2, 1]$, quality PO

| | | | | |
|---|---|---|---|---|
| 3 | 2.089592162197666e-01 | 1.214772766832564e-01 | 4.392613616583718e-01 | 4.392613616583718e-01 |
| 3 | 1.435864594002268e-07 | -2.772879527844379e+00 | 1.886439763922189e+00 | 1.886439763922189e+00 |
| 6 | 6.218698676355368e-02 | 4.193543030528293e-02 | 1.579523486480328e-01 | 8.001122210466843e-01 |

$d = 6$, $n_p = 12$, type $[0, 2, 1]$, quality CC

| | | | | |
|---|---|---|---|---|
| 3 | 4.935e-02+i*8.655e-03 | 2.903e-01-i*1.251e-01 | 3.549e-01+i*6.254e-02 | 3.549e-01+i*6.254e-02 |
| 3 | 4.135e-02+i*2.321e-03 | 8.915e-01-i*4.861e-03 | 5.425e-02+i*2.430e-03 | 5.425e-02+i*2.430e-03 |
| 6 | 1.213e-01-i*5.488e-03 | 7.521e-02-i*2.885e-03 | 2.980e-01+i*2.812e-03 | 6.268e-01+i*7.318e-05 |

$d = 6$, $n_p = 12$, type $[0, 2, 1]$, quality CC

| | | | | |
|---|---|---|---|---|
| 3 | 4.935e-02-i*8.655e-03 | 2.903e-01+i*1.251e-01 | 3.549e-01-i*6.254e-02 | 3.549e-01-i*6.254e-02 |
| 3 | 4.135e-02-i*2.321e-03 | 8.915e-01+i*4.861e-03 | 5.425e-02-i*2.430e-03 | 5.425e-02-i*2.430e-03 |
| 6 | 1.213e-01+i*5.488e-03 | 7.521e-02+i*2.885e-03 | 2.980e-01-i*2.812e-03 | 6.268e-01-i*7.318e-05 |

$d = 7$, $n_p = 13$, type $[1, 2, 1]$, quality NI

| | | | | |
|---|---|---|---|---|
| 1 | -1.495700444676818e-01 | 3.333333333333333e-01 | 3.333333333333333e-01 | 3.333333333333333e-01 |
| 3 | 1.756152574332078e-01 | 4.793080678419203e-01 | 2.603459660790398e-01 | 2.603459660790398e-01 |
| 3 | 5.334723560883849e-02 | 8.697397941955684e-01 | 6.513010290221581e-02 | 6.513010290221581e-02 |
| 6 | 7.711376089025714e-02 | 4.869031542531641e-02 | 3.128654960048739e-01 | 6.384441885698097e-01 |

$d = 7$, $n_p = 13$, type $[1, 2, 1]$, quality PO

| | | | | |
|---|---|---|---|---|
| 1 | 1.972707495121721e-01 | 3.333333333333333e-01 | 3.333333333333333e-01 | 3.333333333333333e-01 |
| 3 | 4.449484431009920e-02 | 8.842157156244530e-01 | 5.789214218777349e-02 | 5.789214218777349e-02 |
| 3 | 7.546437878461855e-07 | -1.205952855704503e+00 | 1.102976427852252e+00 | 1.102976427852252e+00 |
| 6 | 1.115404089376945e-01 | 7.126755844224918e-02 | 2.982123657195186e-01 | 6.305200758382323e-01 |

$d = 7$, $n_p = 13$, type $[1, 2, 1]$, quality CC

| | | | | |
|---|---|---|---|---|
| 1 | 2.047e-01+i*5.977e-03 | 3.333333333333333e-01 | 3.333333333333333e-01 | 3.333333333333333e-01 |
| 3 | 1.238e-01+i*1.614e-02 | 6.404e-02+i*3.796e-03 | 4.680e-01-i*1.898e-03 | 4.680e-01-i*1.898e-03 |
| 3 | 1.534e-01-i*1.157e-02 | 7.787e-01+i*4.230e-02 | 1.107e-01-i*2.115e-02 | 1.107e-01-i*2.115e-02 |
| 6 | -6.083e-03-i*3.278e-03 | -2.921e-02-i*1.531e-01 | 1.131e-01-i*7.177e-04 | 9.161e-01+i*1.538e-01 |

$d = 7$, $n_p = 13$, type $[1, 2, 1]$, quality CC

| | | | | |
|---|---|---|---|---|
| 1 | 2.047e-01-i*5.977e-03 | 3.333333333333333e-01 | 3.333333333333333e-01 | 3.333333333333333e-01 |
| 3 | 1.238e-01-i*1.614e-02 | 6.404e-02-i*3.796e-03 | 4.680e-01+i*1.898e-03 | 4.680e-01+i*1.898e-03 |
| 3 | 1.534e-01+i*1.157e-02 | 7.787e-01-i*4.230e-02 | 1.107e-01+i*2.115e-02 | 1.107e-01+i*2.115e-02 |
| 6 | -6.083e-03+i*3.278e-03 | -2.921e-02+i*1.531e-01 | 1.131e-01+i*7.177e-04 | 9.161e-01-i*1.538e-01 |

$d = 7$, $n_p = 15$, type $[0, 1, 2]$, quality PI

| | | | | |
|---|---|---|---|---|
| 3 | 1.253936074493031e-01 | 5.134817203287849e-01 | 2.432591398356075e-01 | 2.432591398356075e-01 |
| 6 | 7.630633834054171e-02 | 5.071438430720704e-02 | 3.186441898475371e-01 | 6.306414258452559e-01 |
| 6 | 2.766352460147343e-02 | 4.572082984632032e-02 | 8.663663134174900e-02 | 8.676425388119307e-01 |

$d = 7$, $n_p = 15$, type $[0, 1, 2]$, quality PI

| | | | | |
|---|---|---|---|---|
| 3 | 5.307780179023241e-02 | 8.701389736816703e-01 | 6.493051315916486e-02 | 6.493051315916486e-02 |
| 6 | 7.085308369213357e-02 | 1.983844766815067e-01 | 2.845755842491703e-01 | 5.170399390693229e-01 |
| 6 | 6.927468207941689e-02 | 4.386347179237247e-02 | 3.135591843849315e-01 | 6.425773438226960e-01 |

$d = 7$, $n_p = 15$, type $[0, 1, 2]$, quality CC

| | | | | |
|---|---|---|---|---|
| 3 | -3.235e-02-i*9.561e-02 | 1.230e-01+i*1.118e-01 | 4.385e-01-i*5.590e-02 | 4.385e-01-i*5.590e-02 |
| 6 | 1.509e-01+i*4.372e-02 | 8.963e-02+i*3.420e-02 | 3.402e-01+i*2.931e-03 | 5.702e-01-i*3.713e-02 |
| 6 | 3.195e-02+i*4.087e-03 | 2.415e-02-i*1.046e-02 | 1.175e-01+i*1.911e-02 | 8.584e-01-i*8.653e-03 |

$d = 7$, $n_p = 15$, type $[0, 1, 2]$, quality CC

| | | | | |
|---|---|---|---|---|
| 3 | -3.235e-02+i*9.561e-02 | 1.230e-01-i*1.118e-01 | 4.385e-01+i*5.590e-02 | 4.385e-01+i*5.590e-02 |
| 6 | 1.509e-01-i*4.372e-02 | 8.963e-02-i*3.420e-02 | 3.402e-01-i*2.931e-03 | 5.702e-01+i*3.713e-02 |
| 6 | 3.195e-02-i*4.087e-03 | 2.415e-02+i*1.046e-02 | 1.175e-01-i*1.911e-02 | 8.584e-01+i*8.653e-03 |

$d = 8$, $n_p = 16$, type $[1, 3, 1]$, quality PI

| | | | | |
|---|---|---|---|---|
| 1 | 1.443156076777872e-01 | 3.333333333333333e-01 | 3.333333333333333e-01 | 3.333333333333333e-01 |
| 3 | 9.509163426728462e-02 | 8.141482341455369e-02 | 4.592925882927232e-01 | 4.592925882927232e-01 |
| 3 | 1.032173705347183e-01 | 6.588613844964796e-01 | 1.705693077517602e-01 | 1.705693077517602e-01 |
| 3 | 3.245849762319808e-02 | 8.989055433659380e-01 | 5.054722831703098e-02 | 5.054722831703098e-02 |
| 6 | 2.723031417443499e-02 | 8.394777409957605e-03 | 2.631128296346381e-01 | 7.284923929554043e-01 |

$d = 8$, $n_p = 16$, type $[1, 3, 1]$, quality NI

| | | | | |
|---|---|---|---|---|
| 1 | -2.834183851113882e-01 | 3.333333333333333e-01 | 3.333333333333333e-01 | 3.333333333333333e-01 |
| 3 | 2.188298823304475e-01 | 4.593042216691928e-01 | 2.703478891654036e-01 | 2.703478891654036e-01 |
| 3 | 6.990696193265258e-02 | 4.666912123569525e-02 | 4.766654393821524e-01 | 4.766654393821524e-01 |
| 3 | 1.709091267160089e-02 | 9.324563118910393e-01 | 3.377184405448034e-02 | 3.377184405448034e-02 |
| 6 | 6.098918571788089e-02 | 5.146433548666153e-02 | 2.027061737460871e-01 | 7.458294907672514e-01 |

$d = 9$, $n_p = 19$, type $[1, 4, 1]$, quality PI

| | | | | |
|---|---|---|---|---|
| 1 | 9.713579628279883e-02 | 3.333333333333333e-01 | 3.333333333333333e-01 | 3.333333333333333e-01 |
| 3 | 7.782754100477428e-02 | 1.258208170141267e-01 | 4.370895914929366e-01 | 4.370895914929366e-01 |
| 3 | 7.964773892721025e-02 | 6.235929287619345e-01 | 1.882035356190327e-01 | 1.882035356190327e-01 |
| 3 | 3.133470022713907e-02 | 2.063496160252474e-02 | 4.896825191987376e-01 | 4.896825191987376e-01 |
| 3 | 2.557767565869803e-02 | 9.105409732110946e-01 | 4.472951339445271e-02 | 4.472951339445271e-02 |
| 6 | 4.328353937728938e-02 | 3.683841205473628e-02 | 2.219629891607657e-01 | 7.411985987844980e-01 |

$d = 10$, $n_p = 24$, type $[0, 4, 2]$, quality PO

| | | | | |
|---|---|---|---|---|
| 3 | 1.113071865209842e-01 | 5.026978114122357e-01 | 2.486510942938821e-01 | 2.486510942938821e-01 |
| 3 | 7.119670534950083e-02 | 6.635907288263227e-02 | 4.668204635586839e-01 | 4.668204635586839e-01 |
| 3 | 4.696616474360448e-02 | 7.632938936578346e-01 | 1.183530531710827e-01 | 1.183530531710827e-01 |
| 3 | 1.902393645152547e-04 | -1.657729732417002e-01 | 5.828864866208501e-01 | 5.828864866208501e-01 |
| 6 | 4.030080154318636e-02 | 3.781022557738019e-02 | 2.621569284355658e-01 | 7.000328459870540e-01 |
| 6 | 1.153571713417794e-02 | 1.001549024788887e-02 | 7.456459853916804e-02 | 9.154199112129431e-01 |

$d = 10$, $n_p = 24$, type $[0, 4, 2]$, quality PO

| | | | | |
|---|---|---|---|---|
| 3 | 9.692507712273318e-02 | 5.074226937435643e-01 | 2.462886531282178e-01 | 2.462886531282178e-01 |
| 3 | 4.781839996017734e-02 | 1.286004654386225e-01 | 4.356997672806888e-01 | 4.356997672806888e-01 |
| 3 | 4.109023634840217e-02 | 2.964218664317674e-02 | 4.851789066784116e-01 | 4.851789066784116e-01 |
| 3 | 2.538936153411637e-02 | 9.108895849984749e-01 | 4.455520750076253e-02 | 4.455520750076253e-02 |
| 6 | 6.096913196191074e-02 | 5.556920568166035e-02 | 2.198980596698902e-01 | 7.245327346484495e-01 |
| 6 | 8.599722204139380e-05 | -1.912103965528146e-01 | 2.318226334220659e-01 | 9.593877631307487e-01 |

$d = 10$, $n_p = 24$, type $[0, 4, 2]$, quality PO

| | | | | |
|---|---|---|---|---|
| 3 | 1.021164310556899e-01 | 1.873741894559398e-01 | 4.063129052720301e-01 | 4.063129052720301e-01 |
| 3 | 3.753243062934215e-02 | 3.550780182651719e-02 | 4.822460990867414e-01 | 4.822460990867414e-01 |
| 3 | 7.567429430158421e-02 | 6.585688050844513e-01 | 1.707155974577743e-01 | 1.707155974577743e-01 |
| 3 | 4.563222214322113e-05 | 1.176975579059068e+00 | -8.848778952953401e-02 | -8.848778952953401e-02 |
| 6 | 3.894085372377458e-02 | 3.780824829131215e-02 | 2.746261024563111e-01 | 6.875656492523768e-01 |
| 6 | 2.004141883851233e-02 | 2.426288797438504e-02 | 9.052562960335602e-02 | 8.852114824222589e-01 |

$d = 10$, $n_p = 24$, type $[0, 4, 2]$, quality PO

| | | | | |
|---|---|---|---|---|
| 3 | 9.599741042888876e-02 | 1.898400810314716e-01 | 4.050799594842642e-01 | 4.050799594842642e-01 |
| 3 | 7.513135885458828e-02 | 6.421617272601987e-01 | 1.789191363699007e-01 | 1.789191363699007e-01 |
| 3 | 9.867483567666925e-03 | 9.460415689037733e-01 | 2.697921554811336e-02 | 2.697921554811336e-02 |
| 3 | 8.760199500273730e-10 | -1.260342691863928e+00 | 1.130171345931964e+00 | 1.130171345931964e+00 |
| 6 | 4.640707470960211e-02 | 3.827649052610617e-02 | 3.574456156027844e-01 | 6.042778938711095e-01 |
| 6 | 2.976146509348259e-02 | 3.421894955482090e-02 | 1.480202526474223e-01 | 8.177607977977568e-01 |

$d = 10$, $n_p = 24$, type $[0, 4, 2]$, quality NO

| | | | | |
|---|---|---|---|---|
| 3 | 1.236684309825885e-01 | 5.119016025712940e-01 | 2.440491987143530e-01 | 2.440491987143530e-01 |
| 3 | 7.443013227349203e-02 | 5.269598579799418e-02 | 4.736520071010029e-01 | 4.736520071010029e-01 |
| 3 | 2.104077630330353e-02 | 9.205479385373168e-01 | 3.972603073134159e-02 | 3.972603073134159e-02 |
| 3 | -8.033172144993467e-09 | -1.511429765803512e+00 | 1.255714882901756e+00 | 1.255714882901756e+00 |
| 6 | 5.709685101130022e-02 | 4.935376022874730e-02 | 2.094009006809330e-01 | 7.412453390903197e-01 |
| 6 | 1.498922604922153e-07 | -9.426332499824509e-01 | 7.533148446910445e-01 | 1.189318405291406e+00 |

$d = 10$, $n_p = 24$, type $[0, 4, 2]$, quality CC

| | | | | |
|---|---|---|---|---|
| 3 | 5.277106485193921e-02 | 3.732125752386770e-02 | 4.813393712380661e-01 | 4.813393712380661e-01 |
| 3 | 2.492198600544332e-02 | 9.118099151434606e-01 | 4.409504242826971e-02 | 4.409504242826971e-02 |
| 3 | -9.824e-02+i*2.109e-01 | 5.933e-01+i*5.695e-02 | 2.033e-01-i*2.848e-02 | 2.033e-01-i*2.848e-02 |
| 3 | -9.824e-02-i*2.109e-01 | 5.933e-01-i*5.695e-02 | 2.033e-01+i*2.848e-02 | 2.033e-01+i*2.848e-02 |
| 6 | 2.176973842142864e-01 | 1.297928977055975e-01 | 2.185542631560071e-01 | 6.516528391383955e-01 |
| 6 | 8.365369419937155e-03 | -2.116915828170165e-02 | 2.227246551358855e-01 | 7.984445031458161e-01 |

$d = 10$, $n_p = 24$, type $[0, 4, 2]$, quality CC

| | | | | |
|---|---|---|---|---|
| 3 | 1.271e-01+i*1.946e-02 | 1.776e-01-i*7.046e-03 | 4.112e-01+i*3.523e-03 | 4.112e-01+i*3.523e-03 |
| 3 | 7.268e-02+i*1.323e-02 | 4.475e-02+i*4.403e-03 | 4.776e-01-i*2.201e-03 | 4.776e-01-i*2.201e-03 |
| 3 | 7.103e-02-i*4.153e-03 | 7.075e-01+i*1.477e-02 | 1.462e-01-i*7.386e-03 | 1.462e-01-i*7.386e-03 |
| 3 | 1.976e-02-i*5.432e-04 | 9.221e-01+i*1.079e-03 | 3.894e-02-i*5.393e-04 | 3.894e-02-i*5.393e-04 |
| 6 | -4.937e-03-i*1.099e-02 | 1.043e-01+i*1.731e-03 | 3.943e-01-i*1.642e-01 | 5.015e-01+i*1.624e-01 |
| 6 | 2.632e-02-i*3.014e-03 | 1.948e-02-i*3.739e-03 | 2.081e-01-i*1.422e-04 | 7.725e-01+i*3.881e-03 |

$d = 10$, $n_p = 24$, type $[0, 4, 2]$, quality CC

| | | | | |
|---|---|---|---|---|
| 3 | 1.271e-01-i*1.946e-02 | 1.776e-01+i*7.046e-03 | 4.112e-01-i*3.523e-03 | 4.112e-01-i*3.523e-03 |
| 3 | 7.268e-02-i*1.323e-02 | 4.475e-02-i*4.403e-03 | 4.776e-01+i*2.201e-03 | 4.776e-01+i*2.201e-03 |
| 3 | 7.103e-02+i*4.153e-03 | 7.075e-01-i*1.477e-02 | 1.462e-01+i*7.386e-03 | 1.462e-01+i*7.386e-03 |
| 3 | 1.976e-02+i*5.432e-04 | 9.221e-01-i*1.079e-03 | 3.894e-02+i*5.393e-04 | 3.894e-02+i*5.393e-04 |
| 6 | -4.937e-03+i*1.099e-02 | 1.043e-01-i*1.731e-03 | 3.943e-01+i*1.642e-01 | 5.015e-01-i*1.624e-01 |
| 6 | 2.632e-02+i*3.014e-03 | 1.948e-02+i*3.739e-03 | 2.081e-01+i*1.422e-04 | 7.725e-01-i*3.881e-03 |

$d = 10$, $n_p = 24$, type $[0, 4, 2]$, quality CC

| | | | | |
|---|---|---|---|---|
| 3 | 9.551e-02+i*1.282e-02 | 4.865e-01+i*7.661e-03 | 2.568e-01-i*3.831e-03 | 2.568e-01-i*3.831e-03 |
| 3 | -2.450e-02-i*4.859e-03 | 2.672e-02-i*6.493e-02 | 4.866e-01+i*3.246e-02 | 4.866e-01+i*3.246e-02 |
| 3 | 5.921e-02-i*1.086e-03 | 7.388e-01-i*1.405e-02 | 1.306e-01+i*7.023e-03 | 1.306e-01+i*7.023e-03 |
| 3 | 1.780e-02-i*1.118e-03 | 9.256e-01+i*1.878e-03 | 3.718e-02-i*9.389e-04 | 3.718e-02-i*9.389e-04 |
| 6 | 7.447e-02-i*5.338e-03 | 6.088e-02-i*2.409e-02 | 3.771e-01+i*1.910e-02 | 5.621e-01+i*4.997e-03 |
| 6 | 1.818e-02+i*2.460e-03 | 1.315e-02+i*9.144e-03 | 1.917e-01-i*1.883e-02 | 7.951e-01+i*9.688e-03 |

$d = 10$, $n_p = 24$, type $[0, 4, 2]$, quality CC

| | | | | |
|---|---|---|---|---|
| 3 | 9.551e-02-i*1.282e-02 | 4.865e-01-i*7.661e-03 | 2.568e-01+i*3.831e-03 | 2.568e-01+i*3.831e-03 |
| 3 | -2.450e-02+i*4.859e-03 | 2.672e-02+i*6.493e-02 | 4.866e-01-i*3.246e-02 | 4.866e-01-i*3.246e-02 |
| 3 | 5.921e-02+i*1.086e-03 | 7.388e-01+i*1.405e-02 | 1.306e-01-i*7.023e-03 | 1.306e-01-i*7.023e-03 |
| 3 | 1.780e-02+i*1.118e-03 | 9.256e-01-i*1.878e-03 | 3.718e-02+i*9.389e-04 | 3.718e-02+i*9.389e-04 |
| 6 | 7.447e-02+i*5.338e-03 | 6.088e-02+i*2.409e-02 | 3.771e-01-i*1.910e-02 | 5.621e-01-i*4.997e-03 |
| 6 | 1.818e-02-i*2.460e-03 | 1.315e-02-i*9.144e-03 | 1.917e-01+i*1.883e-02 | 7.951e-01-i*9.688e-03 |

$d = 10$, $n_p = 24$, type $[0, 4, 2]$, quality CC

| | | | | |
|---|---|---|---|---|
| 3 | 1.358719435989953e-01 | 2.004054461442247e-01 | 3.997972769278876e-01 | 3.997972769278876e-01 |
| 3 | 6.814440284306941e-03 | 9.616949078730796e-01 | 1.915254606346019e-02 | 1.915254606346019e-02 |
| 3 | 1.586e-02-i*6.597e-02 | 5.635e-01+i*6.684e-02 | 2.183e-01-i*3.342e-02 | 2.183e-01-i*3.342e-02 |
| 3 | 1.586e-02+i*6.597e-02 | 5.635e-01-i*6.684e-02 | 2.183e-01+i*3.342e-02 | 2.183e-01+i*3.342e-02 |
| 6 | 4.521993542833537e-02 | 3.622531754605337e-02 | 3.567498979156279e-01 | 6.070247845383188e-01 |
| 6 | 3.424108623694124e-02 | 3.808365017663759e-02 | 1.417605854191583e-01 | 8.201557644042041e-01 |

$d = 10$, $n_p = 24$, type $[0, 4, 2]$, quality CC

| | | | | |
|---|---|---|---|---|
| 3 | 1.177794118402790e-01 | 1.925503067708375e-01 | 4.037248466145812e-01 | 4.037248466145812e-01 |
| 3 | 6.298057687297120e-03 | 9.648657254494669e-01 | 1.756713727526654e-02 | 1.756713727526654e-02 |
| 3 | 2.449e-02-i*2.110e-02 | 6.062e-01+i*9.350e-02 | 1.969e-01-i*4.675e-02 | 1.969e-01-i*4.675e-02 |
| 3 | 2.449e-02+i*2.110e-02 | 6.062e-01-i*9.350e-02 | 1.969e-01+i*4.675e-02 | 1.969e-01+i*4.675e-02 |
| 6 | 4.490881803412202e-02 | 3.588453312863029e-02 | 3.563028765141633e-01 | 6.078125903572064e-01 |
| 6 | 3.523291234224051e-02 | 3.882168421406334e-02 | 1.404951124558004e-01 | 8.206832033301363e-01 |

$d = 10$, $n_p = 24$, type $[0, 4, 2]$, quality CC

| | | | | |
|---|---|---|---|---|
| 3 | 7.999e-02+i*7.502e-03 | 1.898e-01+i*1.483e-03 | 4.051e-01-i*7.413e-04 | 4.051e-01-i*7.413e-04 |
| 3 | 6.816e-02-i*6.033e-04 | 5.803e-01+i*2.274e-02 | 2.098e-01-i*1.137e-02 | 2.098e-01-i*1.137e-02 |
| 3 | 5.233e-02+i*9.819e-06 | 3.714e-02+i*2.384e-05 | 4.814e-01-i*1.192e-05 | 4.814e-01-i*1.192e-05 |
| 3 | 2.517e-02+i*4.582e-05 | 9.113e-01-i*9.331e-05 | 4.435e-02+i*4.666e-05 | 4.435e-02+i*4.666e-05 |
| 6 | 5.384e-02-i*3.469e-03 | 4.804e-02-i*3.531e-03 | 2.192e-01+i*3.309e-04 | 7.328e-01+i*3.200e-03 |
| 6 | 9.485e-07-i*8.585e-06 | -3.140e-01-i*9.245e-02 | 2.494e-01+i*9.077e-03 | 1.065e+00+i*8.337e-02 |

$d = 10$, $n_p = 24$, type $[0, 4, 2]$, quality CC

| | | | | |
|---|---|---|---|---|
| 3 | 7.999e-02-i*7.502e-03 | 1.898e-01-i*1.483e-03 | 4.051e-01+i*7.413e-04 | 4.051e-01+i*7.413e-04 |
| 3 | 6.816e-02+i*6.033e-04 | 5.803e-01-i*2.274e-02 | 2.098e-01+i*1.137e-02 | 2.098e-01+i*1.137e-02 |
| 3 | 5.233e-02-i*9.819e-06 | 3.714e-02-i*2.384e-05 | 4.814e-01+i*1.192e-05 | 4.814e-01+i*1.192e-05 |
| 3 | 2.517e-02-i*4.582e-05 | 9.113e-01+i*9.331e-05 | 4.435e-02-i*4.666e-05 | 4.435e-02-i*4.666e-05 |
| 6 | 5.384e-02+i*3.469e-03 | 4.804e-02+i*3.531e-03 | 2.192e-01-i*3.309e-04 | 7.328e-01-i*3.200e-03 |
| 6 | 9.485e-07+i*8.585e-06 | -3.140e-01+i*9.245e-02 | 2.494e-01-i*9.077e-03 | 1.065e+00-i*8.337e-02 |

$d = 10$, $n_p = 25$, type $[1, 2, 3]$, quality PI

| | | | | |
|---|---|---|---|---|
| 1 | 9.081799038275358e-02 | 3.333333333333333e-01 | 3.333333333333333e-01 | 3.333333333333333e-01 |
| 3 | 3.672595775646670e-02 | 2.884473323268525e-02 | 4.855776333836574e-01 | 4.855776333836574e-01 |
| 3 | 4.532105943552793e-02 | 7.810368490299259e-01 | 1.094815754850371e-01 | 1.094815754850371e-01 |
| 6 | 7.275791684542011e-02 | 1.417072194148800e-01 | 3.079398387641210e-01 | 5.503529418209991e-01 |
| 6 | 2.832724253105748e-02 | 2.500353476268639e-02 | 2.466725606399027e-01 | 7.283239045974109e-01 |
| 6 | 9.421666963732823e-03 | 9.540815400299458e-03 | 6.680325101220027e-02 | 9.236559335875003e-01 |

$d = 10$, $n_p = 25$, type $[1, 2, 3]$, quality PI

| | | | | |
|---|---|---|---|---|
| 1 | 8.174332914628597e-02 | 3.333333333333333e-01 | 3.333333333333333e-01 | 3.333333333333333e-01 |
| 3 | 4.595796360474473e-02 | 7.156777978868712e-01 | 1.421611010565644e-01 | 1.421611010565644e-01 |
| 3 | 1.335296881314957e-02 | 9.358892535661130e-01 | 3.205537321694351e-02 | 3.205537321694351e-02 |
| 6 | 6.390490639642405e-02 | 1.481328857838206e-01 | 3.218129952888354e-01 | 5.300541189273440e-01 |
| 6 | 3.418464816295943e-02 | 2.961988948872977e-02 | 3.691467818278110e-01 | 6.012333286834592e-01 |
| 6 | 2.529775770728838e-02 | 2.836766533993844e-02 | 1.637017337371825e-01 | 8.079306009228791e-01 |

$d = 10$, $n_p = 25$, type $[1, 2, 3]$, quality PI

| | | | | |
|---|---|---|---|---|
| 1 | 8.321973698645014e-02 | 3.333333333333333e-01 | 3.333333333333333e-01 | 3.333333333333333e-01 |
| 3 | 5.265194946824459e-02 | 6.741737642518105e-01 | 1.629131178740948e-01 | 1.629131178740948e-01 |
| 3 | 1.095128834026841e-02 | 9.429929994232243e-01 | 2.850350028838784e-02 | 2.850350028838784e-02 |
| 6 | 5.627727971081118e-02 | 1.468115053939304e-01 | 3.366958752782316e-01 | 5.164926193278379e-01 |
| 6 | 3.539494779153839e-02 | 2.930760450457947e-02 | 3.633626169945705e-01 | 6.073297785008500e-01 |
| 6 | 2.932286409565224e-02 | 3.368569868061029e-02 | 1.533030551695614e-01 | 8.130112461498283e-01 |

$d = 10$, $n_p = 25$, type $[1, 2, 3]$, quality PI

| | | | | |
|---|---|---|---|---|
| 1 | 7.989450474123971e-02 | 3.333333333333333e-01 | 3.333333333333333e-01 | 3.333333333333333e-01 |
| 3 | 7.112380223237733e-02 | 1.498275787958189e-01 | 4.250862106020906e-01 | 4.250862106020906e-01 |
| 3 | 8.223818690464196e-03 | 9.533822649799996e-01 | 2.330886751000019e-02 | 2.330886751000019e-02 |
| 6 | 4.543059229617002e-02 | 1.479256262095344e-01 | 2.237669735769730e-01 | 6.283074002134926e-01 |
| 6 | 3.735985623430528e-02 | 2.994603195417089e-02 | 3.587401418644315e-01 | 6.113138261813976e-01 |
| 6 | 3.088665688456399e-02 | 3.563255958750348e-02 | 1.432953704268671e-01 | 8.210720699856294e-01 |

$d = 10$, $n_p = 25$, type $[1, 2, 3]$, quality NO

| | | | | |
|---|---|---|---|---|
| 1 | -7.666796298141887e-01 | 3.333333333333333e-01 | 3.333333333333333e-01 | 3.333333333333333e-01 |
| 3 | 3.655803798514184e-01 | 4.140154126757789e-01 | 2.929922936621106e-01 | 2.929922936621106e-01 |
| 3 | 6.337005059321771e-02 | 4.684710061961884e-02 | 4.765764496901906e-01 | 4.765764496901906e-01 |
| 6 | 6.645630425322236e-02 | 6.266902949201206e-02 | 2.226110814683924e-01 | 7.147198890395955e-01 |
| 6 | 1.338735065782750e-02 | 2.548944056926703e-02 | 6.532703235568311e-02 | 9.091835270750499e-01 |
| 6 | 1.277348356635279e-04 | -1.832474681550071e-01 | 2.997648596468021e-01 | 8.834826085082051e-01 |

$d = 10$, $n_p = 25$, type $[1, 2, 3]$, quality NO

| | | | | |
|---|---|---|---|---|
| 1 | -2.234216242442501e-02 | 3.333333333333333e-01 | 3.333333333333333e-01 | 3.333333333333333e-01 |
| 3 | 5.375883299230817e-02 | 3.804427929524181e-02 | 4.809778603523791e-01 | 4.809778603523791e-01 |
| 3 | 2.501687033787517e-02 | 9.116086878088240e-01 | 4.419565609558801e-02 | 4.419565609558801e-02 |
| 6 | 6.989538046094846e-02 | 1.993064436135549e-01 | 3.086120750851603e-01 | 4.920814813012848e-01 |
| 6 | 6.097151293906329e-02 | 5.667196507579838e-02 | 2.180515720339544e-01 | 7.252764628902472e-01 |
| 6 | 1.356153389674141e-04 | -1.710229492405390e-01 | 2.375089404721930e-01 | 9.335140087683460e-01 |

$d = 10$, $n_p = 25$, type $[1, 2, 3]$, quality NC

| | | | | |
|---|---|---|---|---|
| 1 | -3.511785671433198e-01 | 3.333333333333333e-01 | 3.333333333333333e-01 | 3.333333333333333e-01 |
| 3 | 1.537094275889405e-01 | 5.637143317945119e-01 | 2.181428341027440e-01 | 2.181428341027440e-01 |
| 3 | 6.003406955064882e-03 | 9.669178906831611e-01 | 1.654105465841945e-02 | 1.654105465841945e-02 |
| 6 | 4.919918345098354e-02 | 3.912778429794670e-02 | 3.552925314380801e-01 | 6.055796842639732e-01 |
| 6 | 3.427224787652705e-02 | 3.792917298073304e-02 | 1.394007651993403e-01 | 8.226700618199267e-01 |
| 6 | 6.186857925770666e-02 | 2.462039460059490e-01 | 3.769e-01-i*1.012e-01 | 3.769e-01+i*1.012e-01 |

$d = 10$, $n_p = 25$, type $[1, 2, 3]$, quality NC

| | | | | |
|---|---|---|---|---|
| 1 | -1.178115856087280e+00 | 3.333333333333333e-01 | 3.333333333333333e-01 | 3.333333333333333e-01 |
| 3 | 5.042597587897799e-01 | 4.023008730495049e-01 | 2.988495634752475e-01 | 2.988495634752475e-01 |
| 3 | 2.951176304210135e-02 | 9.043663027590406e-01 | 4.781684862047970e-02 | 4.781684862047970e-02 |
| 6 | 7.834616921901520e-02 | 5.922133371721720e-02 | 2.437311397226710e-01 | 6.970475265601118e-01 |
| 6 | 8.045535211715699e-05 | -2.179472732472314e-01 | 2.595600030669780e-01 | 9.583872701802534e-01 |
| 6 | 1.770692386080701e-02 | 4.117912010327615e-02 | 4.794e-01-i*1.117e-01 | 4.794e-01+i*1.117e-01 |

$d = 10$, $n_p = 25$, type $[1, 2, 3]$, quality NC

| | | | | |
|---|---|---|---|---|
| 1 | -3.903434917845503e+00 | 3.333333333333333e-01 | 3.333333333333333e-01 | 3.333333333333333e-01 |
| 3 | 1.416543958510859e+00 | 3.752929553388003e-01 | 3.123535223305999e-01 | 3.123535223305999e-01 |
| 3 | 7.094452544803134e-02 | 7.806524006060786e-01 | 1.096737996969607e-01 | 1.096737996969607e-01 |
| 6 | 6.487379159300377e-02 | 4.575157470896738e-02 | 3.352454655310191e-01 | 6.190029597600135e-01 |
| 6 | 8.621119400999336e-03 | -1.381314513364574e-02 | 8.683887903239943e-02 | 9.269742661012463e-01 |
| 6 | 8.023434348787957e-13 | -1.305e-01-i*3.418e+00 | -1.305e-01+i*3.418e+00 | 1.261075255225183e+00 |

$d = 10$, $n_p = 25$, type $[1, 2, 3]$, quality CC

| | | | | |
|---|---|---|---|---|
| 1 | 1.755e-01-i*5.424e-04 | 3.333333333333333e-01 | 3.333333333333333e-01 | 3.333333333333333e-01 |
| 3 | 1.008e-01-i*8.355e-03 | 7.841e-02-i*4.431e-02 | 4.608e-01+i*2.216e-02 | 4.608e-01+i*2.216e-02 |
| 3 | 1.836e-03-i*1.074e-02 | 6.413e-01-i*2.246e-01 | 1.793e-01+i*1.123e-01 | 1.793e-01+i*1.123e-01 |
| 6 | -1.893e-03-i*2.225e-02 | 1.358e-02-i*4.814e-02 | 3.719e-01-i*8.853e-03 | 6.146e-01+i*5.699e-02 |
| 6 | 7.304e-02+i*2.800e-02 | 9.385e-02+i*9.164e-03 | 2.178e-01+i*4.218e-02 | 6.883e-01-i*5.134e-02 |
| 6 | 1.495e-02+i*3.894e-03 | 1.328e-02+i*6.281e-03 | 8.245e-02+i*5.555e-03 | 9.043e-01-i*1.184e-02 |

$d = 10$, $n_p = 25$, type $[1, 2, 3]$, quality CC

| | | | | |
|---|---|---|---|---|
| 1 | 1.755e-01+i*5.424e-04 | 3.333333333333333e-01 | 3.333333333333333e-01 | 3.333333333333333e-01 |
| 3 | 1.008e-01+i*8.355e-03 | 7.841e-02+i*4.431e-02 | 4.608e-01-i*2.216e-02 | 4.608e-01-i*2.216e-02 |
| 3 | 1.836e-03+i*1.074e-02 | 6.413e-01+i*2.246e-01 | 1.793e-01-i*1.123e-01 | 1.793e-01-i*1.123e-01 |
| 6 | -1.893e-03+i*2.225e-02 | 1.358e-02+i*4.814e-02 | 3.719e-01+i*8.853e-03 | 6.146e-01-i*5.699e-02 |
| 6 | 7.304e-02-i*2.800e-02 | 9.385e-02-i*9.164e-03 | 2.178e-01-i*4.218e-02 | 6.883e-01+i*5.134e-02 |
| 6 | 1.495e-02-i*3.894e-03 | 1.328e-02-i*6.281e-03 | 8.245e-02-i*5.555e-03 | 9.043e-01+i*1.184e-02 |

$d = 10$, $n_p = 25$, type $[1, 2, 3]$, quality CC

| | | | | |
|---|---|---|---|---|
| 1 | 1.624e-01+i*5.573e-02 | 3.333333333333333e-01 | 3.333333333333333e-01 | 3.333333333333333e-01 |
| 3 | 3.713e-02-i*1.597e-02 | 1.527e-01-i*9.266e-02 | 4.237e-01+i*4.633e-02 | 4.237e-01+i*4.633e-02 |
| 3 | 7.943e-02+i*3.921e-03 | 6.431e-01-i*5.377e-02 | 1.784e-01+i*2.689e-02 | 1.784e-01+i*2.689e-02 |
| 6 | 5.000e-02-i*1.441e-02 | 4.074e-02-i*1.015e-02 | 3.580e-01+i*4.518e-03 | 6.012e-01+i*5.636e-03 |
| 6 | 2.964e-02+i*4.415e-03 | 2.841e-02+i*2.256e-02 | 1.363e-01+i*3.044e-02 | 8.353e-01-i*5.299e-02 |
| 6 | 1.671e-03+i*6.732e-03 | -3.738e-03+i*4.328e-03 | 6.620e-02+i*4.044e-02 | 9.375e-01-i*4.477e-02 |

$d = 10$, $n_p = 25$, type $[1, 2, 3]$, quality CC

| | | | | |
|---|---|---|---|---|
| 1 | 1.624e-01-i*5.573e-02 | 3.333333333333333e-01 | 3.333333333333333e-01 | 3.333333333333333e-01 |
| 3 | 3.713e-02+i*1.597e-02 | 1.527e-01+i*9.266e-02 | 4.237e-01-i*4.633e-02 | 4.237e-01-i*4.633e-02 |
| 3 | 7.943e-02-i*3.921e-03 | 6.431e-01+i*5.377e-02 | 1.784e-01-i*2.689e-02 | 1.784e-01-i*2.689e-02 |
| 6 | 5.000e-02+i*1.441e-02 | 4.074e-02+i*1.015e-02 | 3.580e-01-i*4.518e-03 | 6.012e-01-i*5.636e-03 |
| 6 | 2.964e-02-i*4.415e-03 | 2.841e-02-i*2.256e-02 | 1.363e-01-i*3.044e-02 | 8.353e-01+i*5.299e-02 |
| 6 | 1.671e-03-i*6.732e-03 | -3.738e-03-i*4.328e-03 | 6.620e-02-i*4.044e-02 | 9.375e-01+i*4.477e-02 |

$d = 10$, $n_p = 25$, type $[1, 2, 3]$, quality CC

| | | | | |
|---|---|---|---|---|
| 1 | 1.188e-01+i*6.118e-03 | 3.333333333333333e-01 | 3.333333333333333e-01 | 3.333333333333333e-01 |
| 3 | 1.639e-02-i*9.198e-03 | -8.224e-03-i*2.346e-02 | 5.041e-01+i*1.173e-02 | 5.041e-01+i*1.173e-02 |
| 3 | 1.403e-02-i*1.465e-03 | 9.355e-01+i*3.852e-03 | 3.223e-02-i*1.926e-03 | 3.223e-02-i*1.926e-03 |
| 6 | 9.069e-02+i*6.139e-03 | 1.122e-01-i*8.763e-03 | 3.166e-01+i*4.914e-03 | 5.712e-01+i*3.849e-03 |
| 6 | 4.096e-02-i*1.819e-03 | 4.065e-02+i*3.315e-04 | 1.751e-01-i*7.957e-03 | 7.842e-01+i*7.626e-03 |
| 6 | 5.618e-06-i*8.462e-06 | -7.407e-02+i*4.155e-01 | 1.844e-01-i*3.578e-01 | 8.896e-01-i*5.767e-02 |

$d = 10$, $n_p = 25$, type $[1, 2, 3]$, quality CC

| | | | | |
|---|---|---|---|---|
| 1 | 1.188e-01-i*6.118e-03 | 3.333333333333333e-01 | 3.333333333333333e-01 | 3.333333333333333e-01 |
| 3 | 1.639e-02+i*9.198e-03 | -8.224e-03+i*2.346e-02 | 5.041e-01-i*1.173e-02 | 5.041e-01-i*1.173e-02 |
| 3 | 1.403e-02+i*1.465e-03 | 9.355e-01-i*3.852e-03 | 3.223e-02+i*1.926e-03 | 3.223e-02+i*1.926e-03 |
| 6 | 9.069e-02-i*6.139e-03 | 1.122e-01+i*8.763e-03 | 3.166e-01-i*4.914e-03 | 5.712e-01-i*3.849e-03 |
| 6 | 4.096e-02+i*1.819e-03 | 4.065e-02-i*3.315e-04 | 1.751e-01+i*7.957e-03 | 7.842e-01-i*7.626e-03 |
| 6 | 5.618e-06+i*8.462e-06 | -7.407e-02-i*4.155e-01 | 1.844e-01+i*3.578e-01 | 8.896e-01+i*5.767e-02 |

$d = 11$, $n_p = 27$, type $[0, 5, 2]$, quality PO

| | | | | |
|---|---|---|---|---|
| 3 | 7.714953491481312e-02 | 2.020613940682896e-01 | 3.989693029658552e-01 | 3.989693029658552e-01 |
| 3 | 5.932297738077407e-02 | 5.933801991374351e-01 | 2.033099004312825e-01 | 2.033099004312825e-01 |
| 3 | 3.618454050341808e-02 | 7.612981754348374e-01 | 1.193509122825813e-01 | 1.193509122825813e-01 |
| 3 | 1.365973100267786e-02 | 9.352701037774482e-01 | 3.236494811127589e-02 | 3.236494811127589e-02 |
| 3 | 9.270063289606761e-04 | -6.922209654151662e-02 | 5.346110482707583e-01 | 5.346110482707583e-01 |
| 6 | 5.233711196220407e-02 | 5.017813831049467e-02 | 3.566206482612926e-01 | 5.932012134282128e-01 |
| 6 | 2.070765963914069e-02 | 2.102201653616630e-02 | 1.714889803040415e-01 | 8.074890031597922e-01 |

$d = 11$, $n_p = 27$, type $[0, 5, 2]$, quality NC

| | | | | |
|---|---|---|---|---|
| 3 | 7.644300834509658e-02 | 4.706185952289155e-01 | 2.646907023855423e-01 | 2.646907023855423e-01 |
| 3 | 1.040872057724585e-01 | 8.893210086075351e-02 | 4.555339495696232e-01 | 4.555339495696232e-01 |
| 3 | 3.530652386121065e-02 | 1.706341992134396e-02 | 4.914682900393280e-01 | 4.914682900393280e-01 |
| 3 | 6.073140434513309e-02 | 6.937428295265409e-01 | 1.531285852367296e-01 | 1.531285852367296e-01 |
| 3 | 1.722544639682646e-02 | 9.272358258964896e-01 | 3.638208705175521e-02 | 3.638208705175521e-02 |
| 6 | 3.059283412711725e-02 | 2.818723450614946e-02 | 1.892188429265186e-01 | 7.825939225673319e-01 |
| 6 | -1.082296182081321e-02 | 5.543638942985082e-02 | 4.723e-01-i*1.531e-01 | 4.723e-01+i*1.531e-01 |

$d = 11$, $n_p = 27$, type $[0, 5, 2]$, quality NC

| | | | | |
|---|---|---|---|---|
| 3 | 9.663724160075700e-02 | 1.913310167160145e-01 | 4.043344916419927e-01 | 4.043344916419927e-01 |
| 3 | 6.285321562569496e-02 | 4.114729090275807e-02 | 4.794263545486210e-01 | 4.794263545486210e-01 |
| 3 | 7.626764489668001e-02 | 6.504168117467320e-01 | 1.747915941266340e-01 | 1.747915941266340e-01 |
| 3 | 2.052202227942507e-02 | 9.206714153502984e-01 | 3.966429232485082e-02 | 3.966429232485082e-02 |
| 3 | 2.332563153290277e-06 | -3.379910139345642e-01 | 6.689955069672821e-01 | 6.689955069672821e-01 |
| 6 | 3.872464464456317e-02 | 3.315615705868087e-02 | 2.059317554331134e-01 | 7.609120875082057e-01 |
| 6 | -1.992064607516610e-04 | 6.359994807231937e-02 | 4.682e-01-i*3.698e-01 | 4.682e-01+i*3.698e-01 |

$d = 11$, $n_p = 27$, type $[0, 5, 2]$, quality CC

| | | | | |
|---|---|---|---|---|
| 3 | 1.022065736188831e-01 | 4.834171422209986e-01 | 2.582914288895007e-01 | 2.582914288895007e-01 |
| 3 | 5.384660137394204e-02 | 7.257198349279758e-01 | 1.371400825360121e-01 | 1.371400825360121e-01 |
| 3 | 1.513362471683927e-02 | 9.312942343491043e-01 | 3.435288282544783e-02 | 3.435288282544783e-02 |
| 3 | 9.927e-04-i*9.604e-04 | 4.326e-02+i*1.706e-01 | 4.784e-01-i*8.529e-02 | 4.784e-01-i*8.529e-02 |
| 3 | 9.927e-04+i*9.604e-04 | 4.326e-02-i*1.706e-01 | 4.784e-01+i*8.529e-02 | 4.784e-01+i*8.529e-02 |
| 6 | 5.847406364512098e-02 | 5.057524053642106e-02 | 3.667390810093398e-01 | 5.826856784542392e-01 |
| 6 | 2.160645956192909e-02 | 2.180035340551002e-02 | 1.731448656570703e-01 | 8.050547809374197e-01 |

$d = 11$, $n_p = 27$, type $[0, 5, 2]$, quality CC

| | | | | |
|---|---|---|---|---|
| 3 | 2.551e-02-i*2.010e-03 | 3.433e-01-i*6.023e-02 | 3.284e-01+i*3.011e-02 | 3.284e-01+i*3.011e-02 |
| 3 | 7.920e-02+i*1.689e-03 | 1.365e-01+i*2.418e-03 | 4.317e-01-i*1.209e-03 | 4.317e-01-i*1.209e-03 |
| 3 | 8.032e-02-i*2.762e-04 | 6.215e-01+i*1.767e-04 | 1.893e-01-i*8.833e-05 | 1.893e-01-i*8.833e-05 |
| 3 | 3.532e-02+i*5.537e-04 | 2.439e-02+i*4.319e-04 | 4.878e-01-i*2.160e-04 | 4.878e-01-i*2.160e-04 |
| 3 | 2.606e-02+i*2.301e-05 | 9.095e-01-i*4.793e-05 | 4.523e-02+i*2.397e-05 | 4.523e-02+i*2.397e-05 |
| 6 | 4.346e-02+i*1.025e-05 | 3.706e-02+i*1.345e-05 | 2.231e-01+i*6.707e-05 | 7.399e-01-i*8.053e-05 |
| 6 | 2.736e-10+i*8.647e-11 | -1.392e+00+i*5.518e-02 | 7.809e-02+i*7.298e-05 | 2.314e+00-i*5.525e-02 |

$d = 11$, $n_p = 27$, type $[0, 5, 2]$, quality CC

| | | | | |
|---|---|---|---|---|
| 3 | 2.551e-02+i*2.010e-03 | 3.433e-01+i*6.023e-02 | 3.284e-01-i*3.011e-02 | 3.284e-01-i*3.011e-02 |
| 3 | 7.920e-02-i*1.689e-03 | 1.365e-01-i*2.418e-03 | 4.317e-01+i*1.209e-03 | 4.317e-01+i*1.209e-03 |
| 3 | 8.032e-02+i*2.762e-04 | 6.215e-01-i*1.767e-04 | 1.893e-01+i*8.833e-05 | 1.893e-01+i*8.833e-05 |
| 3 | 3.532e-02-i*5.537e-04 | 2.439e-02-i*4.319e-04 | 4.878e-01+i*2.160e-04 | 4.878e-01+i*2.160e-04 |
| 3 | 2.606e-02-i*2.301e-05 | 9.095e-01+i*4.793e-05 | 4.523e-02-i*2.397e-05 | 4.523e-02-i*2.397e-05 |
| 6 | 4.346e-02-i*1.025e-05 | 3.706e-02-i*1.345e-05 | 2.231e-01-i*6.707e-05 | 7.399e-01+i*8.053e-05 |
| 6 | 2.736e-10-i*8.647e-11 | -1.392e+00-i*5.518e-02 | 7.809e-02-i*7.298e-05 | 2.314e+00+i*5.525e-02 |

$d = 11$, $n_p = 28$, type $[1, 3, 3]$, quality NI

| | | | | |
|---|---|---|---|---|
| 1 | 1.918874890144834e-01 | 3.333333333333333e-01 | 3.333333333333333e-01 | 3.333333333333333e-01 |
| 3 | 4.494673641886435e-02 | 3.618633512713571e-02 | 4.819068324364321e-01 | 4.819068324364321e-01 |
| 3 | 4.110012887519764e-02 | 8.110470430369368e-01 | 9.447647848153162e-02 | 9.447647848153162e-02 |
| 3 | -3.968990834546128e+00 | 5.167437799769402e-01 | 2.416281100115299e-01 | 2.416281100115299e-01 |
| 6 | 2.034937507030261e+00 | 2.273118971929394e-01 | 2.539744293918833e-01 | 5.187136734151773e-01 |
| 6 | 3.401519357474532e-02 | 3.065503892384041e-02 | 2.512520556604245e-01 | 7.180929054157351e-01 |
| 6 | 7.204702518612579e-03 | 1.500937328757639e-03 | 6.561155330342952e-02 | 9.328875093678128e-01 |

$d = 11$, $n_p = 28$, type $[1, 3, 3]$, quality NI

| | | | | |
|---|---|---|---|---|
| 1 | -6.240162943348243e-02 | 3.333333333333333e-01 | 3.333333333333333e-01 | 3.333333333333333e-01 |
| 3 | 8.172717083864956e-02 | 4.327128944999808e-01 | 2.836435527500096e-01 | 2.836435527500096e-01 |
| 3 | 4.896465250586733e-02 | 7.112097470078995e-01 | 1.443951264960502e-01 | 1.443951264960502e-01 |
| 3 | 1.380135388627025e-02 | 9.345387060670882e-01 | 3.273064696645591e-02 | 3.273064696645591e-02 |
| 6 | 5.340235179593824e-02 | 1.163964134004934e-01 | 3.353500785250607e-01 | 5.482535080744460e-01 |
| 6 | 2.632505873531205e-02 | 2.261151330038821e-02 | 3.724949218910710e-01 | 6.048935648085408e-01 |
| 6 | 2.509293909226987e-02 | 2.799022568208098e-02 | 1.649013104719147e-01 | 8.071084638460043e-01 |

$d = 11$, $n_p = 28$, type $[1, 3, 3]$, quality PO

| | | | | |
|---|---|---|---|---|
| 1 | 8.103415654031123e-02 | 3.333333333333333e-01 | 3.333333333333333e-01 | 3.333333333333333e-01 |
| 3 | 5.521245711458991e-02 | 1.549403633935724e-01 | 4.225298183032138e-01 | 4.225298183032138e-01 |
| 3 | 3.819386598277898e-02 | 3.039920045395750e-02 | 4.848003997730212e-01 | 4.848003997730212e-01 |
| 3 | 3.814130708154661e-02 | 8.420439220789682e-01 | 7.897803896051590e-02 | 7.897803896051590e-02 |
| 6 | 5.281491834213239e-02 | 1.385997646250211e-01 | 2.550244945506976e-01 | 6.063757408242813e-01 |
| 6 | 3.022529791222147e-02 | 2.722512260765257e-02 | 2.478462753334077e-01 | 7.249286020589398e-01 |
| 6 | 4.346942566136523e-03 | -9.893227433531385e-03 | 6.170038756899856e-02 | 9.481928398645328e-01 |

$d = 11$, $n_p = 28$, type $[1, 3, 3]$, quality PO

| | | | | |
|---|---|---|---|---|
| 1 | 7.062089909913476e-02 | 3.333333333333333e-01 | 3.333333333333333e-01 | 3.333333333333333e-01 |
| 3 | 4.863840089306735e-02 | 7.225524909428175e-01 | 1.387237545285912e-01 | 1.387237545285912e-01 |
| 3 | 1.417899528374483e-02 | 9.336554312678324e-01 | 3.317228436608382e-02 | 3.317228436608382e-02 |
| 3 | 1.611710280602759e-04 | -9.702074100173288e-02 | 5.485103705008664e-01 | 5.485103705008664e-01 |
| 6 | 6.093530657379762e-02 | 1.584316224642345e-01 | 3.188956515582766e-01 | 5.226727259774889e-01 |
| 6 | 3.901504738453730e-02 | 3.614003928518986e-02 | 3.664078219490362e-01 | 5.974521387657739e-01 |
| 6 | 2.345687925603972e-02 | 2.551684875520769e-02 | 1.676620435625215e-01 | 8.068211076822708e-01 |

$d = 11$, $n_p = 28$, type $[1, 3, 3]$, quality PO

| | | | | |
|---|---|---|---|---|
| 1 | 8.680578199654031e-02 | 3.333333333333333e-01 | 3.333333333333333e-01 | 3.333333333333333e-01 |
| 3 | 3.649067572499776e-02 | 2.794971816836728e-02 | 4.860251409158164e-01 | 4.860251409158164e-01 |
| 3 | 4.613089159837884e-02 | 6.731620552412965e-01 | 1.634189723793518e-01 | 1.634189723793518e-01 |
| 3 | 3.306625186475146e-02 | 8.807270043513695e-01 | 5.963649782431526e-02 | 5.963649782431526e-02 |
| 6 | 5.879312726288114e-02 | 1.442167060180959e-01 | 3.307971938668732e-01 | 5.249861001150308e-01 |
| 6 | 3.453369249871182e-02 | 3.061750461832727e-02 | 2.403310260162528e-01 | 7.290514693654199e-01 |
| 6 | 1.028306978252956e-03 | -4.573087904223890e-02 | 5.838008973998508e-02 | 9.873507893022538e-01 |

$d = 11$, $n_p = 28$, type $[1, 3, 3]$, quality PO

| | | | | |
|---|---|---|---|---|
| 1 | 9.240141465707048e-02 | 3.333333333333333e-01 | 3.333333333333333e-01 | 3.333333333333333e-01 |
| 3 | 7.705315964304812e-02 | 6.268855781508001e-01 | 1.865572109246000e-01 | 1.865572109246000e-01 |
| 3 | 3.423997592723243e-02 | 2.355377133819504e-02 | 4.882231143309025e-01 | 4.882231143309025e-01 |
| 3 | 2.607378457164280e-02 | 9.094728357504813e-01 | 4.526358212475937e-02 | 4.526358212475937e-02 |
| 6 | 3.986296177031882e-02 | 1.324157313898656e-01 | 4.052954525294021e-01 | 4.622888160807323e-01 |
| 6 | 4.272000825772866e-02 | 3.648097880233658e-02 | 2.230840809720972e-01 | 7.404349402255663e-01 |
| 6 | 7.914790950004850e-10 | -1.214856339121183e+00 | 7.583681845129545e-02 | 2.139019520669888e+00 |

$d = 11$, $n_p = 28$, type $[1, 3, 3]$, quality PO

| | | | | |
|---|---|---|---|---|
| 1 | 9.242953343240852e-02 | 3.333333333333333e-01 | 3.333333333333333e-01 | 3.333333333333333e-01 |
| 3 | 7.624780409334145e-02 | 1.320056867999758e-01 | 4.339971566000121e-01 | 4.339971566000121e-01 |
| 3 | 3.423455884054410e-02 | 2.352966108624836e-02 | 4.882351694568758e-01 | 4.882351694568758e-01 |
| 3 | 2.601823672030473e-02 | 9.096179053541431e-01 | 4.519104732292844e-02 | 4.519104732292844e-02 |
| 6 | 4.025049886116545e-02 | 1.745916351287411e-01 | 2.008024476276966e-01 | 6.246059172435623e-01 |
| 6 | 4.276094558689746e-02 | 3.650887742847141e-02 | 2.229527117670237e-01 | 7.405384108045049e-01 |
| 6 | 1.527738657225798e-10 | -1.508114349834959e+00 | 7.639709072931050e-02 | 2.431717259105649e+00 |

$d = 11$, $n_p = 28$, type $[1, 3, 3]$, quality NO

| | | | | |
|---|---|---|---|---|
| 1 | -6.444064673948750e+01 | 3.333333333333333e-01 | 3.333333333333333e-01 | 3.333333333333333e-01 |
| 3 | 2.156337120324032e+01 | 3.407573267582806e-01 | 3.296213366208597e-01 | 3.296213366208597e-01 |
| 3 | 5.669231145203291e-02 | 5.963799008013352e-02 | 4.701810049599332e-01 | 4.701810049599332e-01 |
| 3 | 4.546992103790541e-03 | 9.693310269601193e-01 | 1.533448651994037e-02 | 1.533448651994037e-02 |
| 6 | 6.070205221830118e-02 | 9.807995682321420e-02 | 2.414720687554708e-01 | 6.604479744213150e-01 |
| 6 | 2.349124822717670e-02 | 3.141246279449187e-02 | 1.172809636961076e-01 | 8.513065735094005e-01 |
| 6 | 1.027590273770016e-02 | -5.316879596835041e-03 | 3.252872681432797e-01 | 6.800296114535553e-01 |

$d = 11$, $n_p = 28$, type $[1, 3, 3]$, quality NO

| | | | | |
|---|---|---|---|---|
| 1 | -8.948351437781234e-01 | 3.333333333333333e-01 | 3.333333333333333e-01 | 3.333333333333333e-01 |
| 3 | 3.913863805758886e-01 | 3.980306287487377e-01 | 3.009846856256311e-01 | 3.009846856256311e-01 |
| 3 | 6.546964133644136e-02 | 6.070907188370493e-02 | 4.696454640581475e-01 | 4.696454640581475e-01 |
| 3 | 4.215746322206285e-05 | 1.153013345359738e+00 | -7.650667267986909e-02 | -7.650667267986909e-02 |
| 6 | 6.431023941129274e-02 | 8.019195896449298e-02 | 2.264314401310975e-01 | 6.933766009044095e-01 |
| 6 | 1.731525662828238e-02 | 2.123385630685585e-02 | 8.502804733618706e-02 | 8.937380963569571e-01 |
| 6 | 5.731271569002774e-03 | -2.379835572015993e-02 | 3.257464511193175e-01 | 6.980519046008424e-01 |

$d = 11$, $n_p = 28$, type $[1, 3, 3]$, quality NO

| | | | | |
|---|---|---|---|---|
| 1 | 8.354763139989195e-02 | 3.333333333333333e-01 | 3.333333333333333e-01 | 3.333333333333333e-01 |
| 3 | 4.495332896089251e-02 | 7.230980522480803e-01 | 1.384509738759599e-01 | 1.384509738759599e-01 |
| 3 | 1.353305805665459e-02 | 9.356473114080119e-01 | 3.217634429599407e-02 | 3.217634429599407e-02 |
| 3 | -6.321870234628512e-10 | 1.880542883110225e+00 | -4.402714415551123e-01 | -4.402714415551123e-01 |
| 6 | 6.526976410004706e-02 | 1.469395909908931e-01 | 3.195263706661379e-01 | 5.335340383429690e-01 |
| 6 | 3.352448040192583e-02 | 2.930313290561486e-02 | 3.706046615353776e-01 | 6.000922055590076e-01 |
| 6 | 2.470462373869841e-02 | 2.738509137240040e-02 | 1.657249099689410e-01 | 8.068899986586586e-01 |

$d = 11$, $n_p = 28$, type $[1, 3, 3]$, quality PC

| | | | | |
|---|---|---|---|---|
| 1 | 9.478443713754539e-02 | 3.333333333333333e-01 | 3.333333333333333e-01 | 3.333333333333333e-01 |
| 3 | 7.590352594328159e-02 | 1.271497159701983e-01 | 4.364251420149008e-01 | 4.364251420149008e-01 |
| 3 | 7.980773833602824e-02 | 6.195730792606873e-01 | 1.902134603696564e-01 | 1.902134603696564e-01 |
| 3 | 3.912133430343436e-02 | 8.827741580093834e-01 | 5.861292099530830e-02 | 5.861292099530830e-02 |
| 6 | 4.900043116370720e-02 | 3.303896594662877e-02 | 2.720257596836592e-01 | 6.949352743697120e-01 |
| 6 | 1.911454022421450e-04 | -1.169317494817391e-01 | 6.201337625583373e-02 | 1.054918373225905e+00 |
| 6 | 4.261384619754331e-03 | 1.320184903531028e-02 | 4.934e-01-i*1.612e-01 | 4.934e-01+i*1.612e-01 |

$d = 11$, $n_p = 28$, type $[1, 3, 3]$, quality PC

| | | | | |
|---|---|---|---|---|
| 1 | 9.305576179070473e-02 | 3.333333333333333e-01 | 3.333333333333333e-01 | 3.333333333333333e-01 |
| 3 | 7.709254161203404e-02 | 1.306722702826980e-01 | 4.346638648586510e-01 | 4.346638648586510e-01 |
| 3 | 7.928194390695918e-02 | 6.244472452136583e-01 | 1.877763773931708e-01 | 1.877763773931708e-01 |
| 3 | 2.742985946166169e-02 | 9.071742507368462e-01 | 4.641287463157690e-02 | 4.641287463157690e-02 |
| 6 | 4.460740119610785e-02 | 3.626551349751969e-02 | 2.303436064349877e-01 | 7.333908800674926e-01 |
| 6 | 5.365983785329571e-09 | -9.439742238020671e-01 | 7.339537766957268e-02 | 1.870578846132494e+00 |
| 6 | 1.464779398246346e-02 | 2.224193675320249e-02 | 4.889e-01-i*5.414e-02 | 4.889e-01+i*5.414e-02 |

$d = 11$, $n_p = 28$, type $[1, 3, 3]$, quality NC

| | | | | |
|---|---|---|---|---|
| 1 | -3.674274101368846e+01 | 3.333333333333333e-01 | 3.333333333333333e-01 | 3.333333333333333e-01 |
| 3 | 1.232484706321282e+01 | 3.424388466658519e-01 | 3.287805766670741e-01 | 3.287805766670741e-01 |
| 3 | 1.417909837688303e-02 | 9.341088821264392e-01 | 3.294555893678042e-02 | 3.294555893678042e-02 |
| 3 | 6.517356262212764e-03 | -2.704838309560608e-02 | 5.135241915478030e-01 | 5.135241915478030e-01 |
| 6 | 7.606758279474378e-02 | 7.681589092113013e-02 | 3.312733825935125e-01 | 5.919107264853574e-01 |
| 6 | 3.295089418010134e-02 | 3.281200000608670e-02 | 1.723012378575729e-01 | 7.948867621363404e-01 |
| 6 | 8.666599713941777e-03 | 1.488e-01-i*9.999e-02 | 1.488e-01+i*9.999e-02 | 7.023195304157000e-01 |

$d = 11$, $n_p = 28$, type $[1, 3, 3]$, quality NC

| | | | | |
|---|---|---|---|---|
| 1 | -7.607523089092928e-01 | 3.333333333333333e-01 | 3.333333333333333e-01 | 3.333333333333333e-01 |
| 3 | 3.486211976284935e-01 | 2.656218698530042e-01 | 3.671890650734979e-01 | 3.671890650734979e-01 |
| 3 | 7.170969293832582e-02 | 6.773689956288715e-01 | 1.613155021855642e-01 | 1.613155021855642e-01 |
| 3 | 4.297937116875782e-06 | -3.406995465193188e-01 | 6.703497732596594e-01 | 6.703497732596594e-01 |
| 6 | 5.492614158081669e-02 | 4.543538983856531e-02 | 3.549951581281783e-01 | 5.995694520332564e-01 |
| 6 | 2.554099958173523e-02 | 2.190562910172119e-02 | 1.365778401540281e-01 | 8.415165307442508e-01 |
| 6 | 2.823982737028783e-03 | 1.800e-02-i*3.383e-02 | 1.800e-02+i*3.383e-02 | 9.640011518693551e-01 |

$d = 11$, $n_p = 28$, type $[1,3,3]$, quality NC

| | | | | |
|---|---|---|---|---|
| 1 | -9.512480050039531e-01 | 3.333333333333333e-01 | 3.333333333333333e-01 | 3.333333333333333e-01 |
| 3 | 4.417571301837738e-01 | 4.194317600711132e-01 | 2.902841199644434e-01 | 2.902841199644434e-01 |
| 3 | 5.677555976154027e-02 | 4.026040311033344e-02 | 4.798697984448333e-01 | 4.798697984448333e-01 |
| 3 | 2.610125926163343e-02 | 9.093837522498476e-01 | 4.530812387507621e-02 | 4.530812387507621e-02 |
| 6 | 6.286961568044845e-02 | 5.467935011581393e-02 | 2.227366850207297e-01 | 7.225839648634564e-01 |
| 6 | 2.483448212852227e-06 | -4.167140858855286e-01 | 1.793605604421121e-01 | 1.237353525443417e+00 |
| 6 | 1.892710185712507e-05 | 3.095336690761896e-01 | 3.452e-01-i*5.535e-01 | 3.452e-01+i*5.535e-01 |

$d = 11$, $n_p = 28$, type $[1,3,3]$, quality NC

| | | | | |
|---|---|---|---|---|
| 1 | 9.264637658838440e-02 | 3.333333333333333e-01 | 3.333333333333333e-01 | 3.333333333333333e-01 |
| 3 | 7.743417731355679e-02 | 1.314654464357271e-01 | 4.342672767821364e-01 | 4.342672767821364e-01 |
| 3 | 7.915366179805717e-02 | 6.256762477497286e-01 | 1.871618761251357e-01 | 1.871618761251357e-01 |
| 3 | 3.410168858734214e-02 | 2.330443909781449e-02 | 4.883477804510928e-01 | 4.883477804510928e-01 |
| 6 | 4.306766448079726e-02 | 3.675368301491709e-02 | 2.222743353435667e-01 | 7.409719816415162e-01 |
| 6 | 1.281317557376122e-02 | 4.007426735729309e-02 | 4.941666840158073e-02 | 9.105090642411262e-01 |
| 6 | -2.100604345745184e-12 | 7.721729807245186e-02 | 4.614e-01-i*2.970e+00 | 4.614e-01+i*2.970e+00 |

$d = 11$, $n_p = 28$, type $[1,3,3]$, quality CC

| | | | | |
|---|---|---|---|---|
| 1 | 1.075668899454949e-01 | 3.333333333333333e-01 | 3.333333333333333e-01 | 3.333333333333333e-01 |
| 3 | 5.050399943119756e-02 | -2.709145207309484e-02 | 5.135457260365474e-01 | 5.135457260365474e-01 |
| 3 | -1.371e-03-i*9.267e-03 | 9.172e-01+i*5.606e-02 | 4.138e-02-i*2.803e-02 | 4.138e-02-i*2.803e-02 |
| 3 | -1.371e-03+i*9.267e-03 | 9.172e-01-i*5.606e-02 | 4.138e-02+i*2.803e-02 | 4.138e-02+i*2.803e-02 |
| 6 | 8.873469422811158e-02 | 1.206804036158372e-01 | 3.134956497358211e-01 | 5.658239466483417e-01 |
| 6 | 4.793305768488000e-02 | 4.631198717699563e-02 | 1.496020472075786e-01 | 8.040859656154257e-01 |
| 6 | -1.180968234395948e-02 | -4.497570515678598e-02 | 5.225e-01-i*7.808e-02 | 5.225e-01+i*7.808e-02 |

$d = 11$, $n_p = 28$, type $[1,3,3]$, quality CC

| | | | | |
|---|---|---|---|---|
| 1 | 8.880e-02-i*1.151e-03 | 3.333333333333333e-01 | 3.333333333333333e-01 | 3.333333333333333e-01 |
| 3 | 7.906e-02-i*3.018e-02 | 1.440e-01-i*4.649e-03 | 4.280e-01+i*2.325e-03 | 4.280e-01+i*2.325e-03 |
| 3 | 6.638e-02+i*2.199e-02 | 6.800e-01-i*4.230e-02 | 1.600e-01+i*2.115e-02 | 1.600e-01+i*2.115e-02 |
| 3 | 1.413e-02+i*1.438e-05 | 9.335e-01-i*3.902e-05 | 3.323e-02+i*1.951e-05 | 3.323e-02+i*1.951e-05 |
| 6 | 1.235e-02+i*6.436e-04 | 1.578e-01+i*1.029e-03 | 2.820e-01+i*1.318e-01 | 5.602e-01-i*1.328e-01 |
| 6 | 3.261e-02-i*1.318e-04 | 2.810e-02-i*1.026e-04 | 3.695e-01-i*1.056e-05 | 6.024e-01+i*1.131e-04 |
| 6 | 2.712e-02+i*3.770e-03 | 3.054e-02+i*4.159e-03 | 1.646e-01+i*1.211e-04 | 8.049e-01-i*4.280e-03 |

$d = 11$, $n_p = 28$, type $[1,3,3]$, quality CC

| | | | | |
|---|---|---|---|---|
| 1 | 8.880e-02+i*1.151e-03 | 3.333333333333333e-01 | 3.333333333333333e-01 | 3.333333333333333e-01 |
| 3 | 7.906e-02+i*3.018e-02 | 1.440e-01+i*4.649e-03 | 4.280e-01-i*2.325e-03 | 4.280e-01-i*2.325e-03 |
| 3 | 6.638e-02-i*2.199e-02 | 6.800e-01+i*4.230e-02 | 1.600e-01-i*2.115e-02 | 1.600e-01-i*2.115e-02 |
| 3 | 1.413e-02-i*1.438e-05 | 9.335e-01+i*3.902e-05 | 3.323e-02-i*1.951e-05 | 3.323e-02-i*1.951e-05 |
| 6 | 1.235e-02-i*6.436e-04 | 1.578e-01-i*1.029e-03 | 2.820e-01-i*1.318e-01 | 5.602e-01+i*1.328e-01 |
| 6 | 3.261e-02+i*1.318e-04 | 2.810e-02+i*1.026e-04 | 3.695e-01+i*1.056e-05 | 6.024e-01-i*1.131e-04 |
| 6 | 2.712e-02-i*3.770e-03 | 3.054e-02-i*4.159e-03 | 1.646e-01-i*1.211e-04 | 8.049e-01+i*4.280e-03 |

$d = 11$, $n_p = 28$, type $[1,3,3]$, quality CC

| | | | | |
|---|---|---|---|---|
| 1 | 8.534e-02+i*4.496e-05 | 3.333333333333333e-01 | 3.333333333333333e-01 | 3.333333333333333e-01 |
| 3 | 3.536e-02-i*3.277e-03 | 2.964e-02+i*3.739e-04 | 4.852e-01-i*1.869e-04 | 4.852e-01-i*1.869e-04 |
| 3 | 4.265e-02+i*2.024e-04 | 7.327e-01+i*3.659e-03 | 1.337e-01-i*1.830e-03 | 1.337e-01-i*1.830e-03 |
| 3 | 1.033e-02+i*1.102e-02 | 9.350e-01-i*2.213e-02 | 3.251e-02+i*1.106e-02 | 3.251e-02+i*1.106e-02 |
| 6 | 6.716e-02+i*3.782e-04 | 1.457e-01-i*3.959e-05 | 3.163e-01-i*6.316e-04 | 5.381e-01+i*6.712e-04 |
| 6 | 2.897e-02-i*4.058e-03 | 2.728e-02-i*3.405e-04 | 2.597e-01+i*2.512e-02 | 7.130e-01-i*2.478e-02 |
| 6 | 1.215e-02-i*2.994e-04 | 2.905e-02-i*1.361e-03 | 1.059e-01+i*5.365e-02 | 8.651e-01-i*5.229e-02 |

$d = 11$, $n_p = 28$, type $[1,3,3]$, quality CC

| | | | | |
|---|---|---|---|---|
| 1 | 8.534e-02-i*4.496e-05 | 3.333333333333333e-01 | 3.333333333333333e-01 | 3.333333333333333e-01 |
| 3 | 3.536e-02+i*3.277e-03 | 2.964e-02-i*3.739e-04 | 4.852e-01+i*1.869e-04 | 4.852e-01+i*1.869e-04 |
| 3 | 4.265e-02-i*2.024e-04 | 7.327e-01-i*3.659e-03 | 1.337e-01+i*1.830e-03 | 1.337e-01+i*1.830e-03 |
| 3 | 1.033e-02-i*1.102e-02 | 9.350e-01+i*2.213e-02 | 3.251e-02-i*1.106e-02 | 3.251e-02-i*1.106e-02 |
| 6 | 6.716e-02-i*3.782e-04 | 1.457e-01+i*3.959e-05 | 3.163e-01+i*6.316e-04 | 5.381e-01-i*6.712e-04 |
| 6 | 2.897e-02+i*4.058e-03 | 2.728e-02+i*3.405e-04 | 2.597e-01-i*2.512e-02 | 7.130e-01+i*2.478e-02 |
| 6 | 1.215e-02+i*2.994e-04 | 2.905e-02+i*1.361e-03 | 1.059e-01-i*5.365e-02 | 8.651e-01+i*5.229e-02 |

$d = 11$, $n_p = 28$, type $[1,3,3]$, quality CC

| | | | | |
|---|---|---|---|---|
| 1 | -3.460e-03+i*1.971e-01 | 3.333333333333333e-01 | 3.333333333333333e-01 | 3.333333333333333e-01 |
| 3 | 8.828e-02-i*6.184e-02 | 2.278e-01-i*4.623e-02 | 3.861e-01+i*2.312e-02 | 3.861e-01+i*2.312e-02 |
| 3 | 6.892e-02+i*5.717e-03 | 6.388e-01-i*9.408e-03 | 1.806e-01+i*4.704e-03 | 1.806e-01+i*4.704e-03 |
| 3 | 1.118e-02-i*3.389e-04 | 9.422e-01+i*1.150e-03 | 2.888e-02-i*5.749e-04 | 2.888e-02-i*5.749e-04 |
| 6 | 5.162e-02-i*5.031e-03 | 4.495e-02-i*6.607e-03 | 3.616e-01+i*1.640e-04 | 5.934e-01+i*6.443e-03 |
| 6 | 3.155e-02+i*4.779e-04 | 3.606e-02+i*4.906e-04 | 1.545e-01-i*1.029e-03 | 8.094e-01+i*5.387e-04 |
| 6 | -1.168e-04-i*6.521e-05 | -1.151e-01-i*9.873e-02 | 3.800e-01+i*1.382e-02 | 7.351e-01+i*8.490e-02 |

$d = 11$, $n_p = 28$, type $[1,3,3]$, quality CC

| | | | | |
|---|---|---|---|---|
| 1 | -3.460e-03-i*1.971e-01 | 3.333333333333333e-01 | 3.333333333333333e-01 | 3.333333333333333e-01 |
| 3 | 8.828e-02+i*6.184e-02 | 2.278e-01+i*4.623e-02 | 3.861e-01-i*2.312e-02 | 3.861e-01-i*2.312e-02 |
| 3 | 6.892e-02-i*5.717e-03 | 6.388e-01+i*9.408e-03 | 1.806e-01-i*4.704e-03 | 1.806e-01-i*4.704e-03 |
| 3 | 1.118e-02+i*3.389e-04 | 9.422e-01-i*1.150e-03 | 2.888e-02+i*5.749e-04 | 2.888e-02+i*5.749e-04 |
| 6 | 5.162e-02+i*5.031e-03 | 4.495e-02+i*6.607e-03 | 3.616e-01-i*1.640e-04 | 5.934e-01-i*6.443e-03 |
| 6 | 3.155e-02-i*4.779e-04 | 3.606e-02-i*4.906e-04 | 1.545e-01+i*1.029e-03 | 8.094e-01-i*5.387e-04 |
| 6 | -1.168e-04+i*6.521e-05 | -1.151e-01+i*9.873e-02 | 3.800e-01-i*1.382e-02 | 7.351e-01-i*8.490e-02 |

$d = 11$, $n_p = 30$, type $[0,2,4]$, quality PI

| | | | | |
|---|---|---|---|---|
| 3 | 5.623165917468111e-02 | 4.470587017120257e-01 | 2.764706491439872e-01 | 2.764706491439872e-01 |
| 3 | 4.776140553308587e-02 | 7.160355004191862e-01 | 1.419822497904069e-01 | 1.419822497904069e-01 |
| 6 | 5.473425616511274e-02 | 1.230230372259886e-01 | 3.322412718141577e-01 | 5.447356909598537e-01 |
| 6 | 2.801405891803870e-02 | 2.440399719079145e-02 | 3.726974607915782e-01 | 6.028985420176303e-01 |
| 6 | 2.479873781819909e-02 | 2.785386480846610e-02 | 1.671151632795214e-01 | 8.050309719120125e-01 |
| 6 | 7.123081411432649e-03 | 2.715094170950369e-02 | 3.934509469602969e-02 | 9.335039635944666e-01 |

$d = 11$, $n_p = 30$, type $[0,2,4]$, quality PI

| | | | | |
|---|---|---|---|---|
| 3 | 7.217804239720927e-02 | 2.128984074010406e-01 | 3.935507962994797e-01 | 3.935507962994797e-01 |
| 3 | 4.321543561536084e-02 | 4.041868382205103e-02 | 4.797906580889745e-01 | 4.797906580889745e-01 |
| 6 | 5.817371032216302e-02 | 1.253995635366209e-01 | 2.659762019033016e-01 | 6.086242345600775e-01 |
| 6 | 1.697584832298340e-02 | 1.240997015369853e-02 | 2.853641853869646e-01 | 7.022258444593369e-01 |
| 6 | 2.759146415644959e-02 | 5.279205798821771e-02 | 1.372353674781709e-01 | 8.099725745336114e-01 |
| 6 | 6.228904858785596e-03 | 5.100344564582806e-03 | 5.681715578857245e-02 | 9.380824996468447e-01 |

$d = 11$, $n_p = 30$, type $[0,2,4]$, quality PI

| | | | | |
|---|---|---|---|---|
| 3 | 5.832566212744962e-02 | 4.504543641757660e-01 | 2.747728179121170e-01 | 2.747728179121170e-01 |
| 3 | 1.387599563149455e-02 | 9.343162547117883e-01 | 3.284187264410585e-02 | 3.284187264410585e-02 |
| 6 | 5.336354239334048e-02 | 1.214249938587573e-01 | 3.347953592492709e-01 | 5.437796468919718e-01 |
| 6 | 2.781232090455112e-02 | 2.400046762583091e-02 | 3.718599950903680e-01 | 6.041395372838011e-01 |
| 6 | 2.525341262993140e-02 | 1.270006888757827e-01 | 1.580400095523586e-01 | 7.149593015718587e-01 |
| 6 | 2.413656185937158e-02 | 2.703971256481997e-02 | 1.649223432616415e-01 | 8.080379441735386e-01 |

$d = 11$, $n_p = 30$, type $[0,2,4]$, quality PI

| | | | | |
|---|---|---|---|---|
| 3 | 4.888313586239229e-02 | 7.118787020151916e-01 | 1.440606489924042e-01 | 1.440606489924042e-01 |
| 3 | 1.381436845965494e-02 | 9.345094686995734e-01 | 3.274526565021330e-02 | 3.274526565021330e-02 |
| 6 | 3.511195082989262e-02 | 2.404698682473196e-01 | 3.020758710955400e-01 | 4.574542606571404e-01 |
| 6 | 5.015309687490970e-02 | 1.100051862098844e-01 | 3.372221080172993e-01 | 5.527727057728163e-01 |
| 6 | 2.503977132164279e-02 | 2.152075977107619e-02 | 3.731132768172773e-01 | 6.053659634116466e-01 |
| 6 | 2.501309547919794e-02 | 2.787575641695829e-02 | 1.650070701309573e-01 | 8.071171734520844e-01 |

$d = 11$, $n_p = 30$, type $[0,2,4]$, quality PO

| | | | | |
|---|---|---|---|---|
| 3 | 9.146460925792323e-02 | 1.932811803214623e-01 | 4.033594098392688e-01 | 4.033594098392688e-01 |
| 3 | 1.077652485656911e-02 | 9.435389719586807e-01 | 2.823051402065965e-02 | 2.823051402065965e-02 |
| 6 | 3.858935164239617e-02 | 1.609441871369630e-01 | 2.056034975881083e-01 | 6.334523152749287e-01 |
| 6 | 4.548838170586973e-02 | 3.916227679633498e-02 | 3.619822445159721e-01 | 5.988554786876929e-01 |
| 6 | 3.146386578675350e-02 | 3.617454811634562e-02 | 1.527247315066171e-01 | 8.111007203770372e-01 |
| 6 | 4.500474401094019e-06 | -2.839704914959607e-01 | 3.953703085041258e-01 | 8.886001829918350e-01 |

$d = 11$, $n_p = 30$, type $[0,2,4]$, quality NO

| | | | | |
|---|---|---|---|---|
| 3 | 1.046552374072418e-01 | 4.953618249513159e-01 | 2.523190875243421e-01 | 2.523190875243421e-01 |
| 3 | -4.201657598214284e-13 | -2.874039728765704e+00 | 1.937019864382852e+00 | 1.937019864382852e+00 |
| 6 | 5.124013901471287e-02 | 6.499863400131213e-02 | 3.835251966747101e-01 | 5.514761693239778e-01 |
| 6 | 5.001030269100911e-02 | 6.242508241686238e-02 | 1.909211148225356e-01 | 7.466538027606020e-01 |
| 6 | 1.088659988221991e-02 | 1.348647350462758e-02 | 6.829338874047763e-02 | 9.182201377548948e-01 |
| 6 | 2.202006375313941e-03 | -5.655605450014434e-02 | 3.581899684755242e-01 | 6.983660860246201e-01 |

$d = 11$, $n_p = 30$, type $[0,2,4]$, quality PC

| | | | | |
|---|---|---|---|---|
| 3 | 4.813139868863970e-02 | 4.187881615097658e-01 | 2.906059192451171e-01 | 2.906059192451171e-01 |
| 3 | 2.024210178662841e-02 | -6.766677156498676e-03 | 5.033833385782493e-01 | 5.033833385782493e-01 |
| 6 | 7.962748197508636e-02 | 1.141071609684337e-01 | 3.196119608257670e-01 | 5.662808782057993e-01 |
| 6 | 4.407477594691577e-02 | 4.666371038032501e-02 | 1.846304040067430e-01 | 7.687058856129320e-01 |
| 6 | 8.775867751393290e-03 | 1.519450616593240e-02 | 5.803390335651477e-02 | 9.267715904775528e-01 |
| 6 | 1.790755637190237e-06 | -4.451e-03-i*4.883e-01 | -4.451e-03+i*4.883e-01 | 1.008901313363203e+00 |

$d = 11$, $n_p = 30$, type $[0,2,4]$, quality PC

| | | | | |
|---|---|---|---|---|
| 3 | 4.152085508334644e-02 | 3.342412178729761e-02 | 4.832879391063512e-01 | 4.832879391063512e-01 |
| 3 | 4.179160980924176e-02 | 8.095645415795505e-01 | 9.521772921022473e-02 | 9.521772921022473e-02 |
| 6 | 7.769934744753965e-02 | 1.578202665605547e-01 | 2.912912988429158e-01 | 5.508884345965295e-01 |
| 6 | 3.183884425444742e-02 | 2.888018532713458e-02 | 2.497858858191612e-01 | 7.213339288537042e-01 |
| 6 | 7.222761138498196e-03 | 1.786107839349653e-03 | 6.529508252404634e-02 | 9.329188096366040e-01 |
| 6 | 8.249481379887305e-03 | 2.511500535455142e-01 | 3.744e-01-i*1.348e-01 | 3.744e-01+i*1.348e-01 |

$d = 11$, $n_p = 30$, type $[0,2,4]$, quality PC

| | | | | |
|---|---|---|---|---|
| 3 | 5.950795085979763e-02 | 7.016306524513449e-01 | 1.491846737743276e-01 | 1.491846737743276e-01 |
| 3 | 1.157288317062918e-04 | -1.448265050823015e-01 | 5.724132525411507e-01 | 5.724132525411507e-01 |
| 6 | 5.770462374303046e-02 | 1.957117321488564e-01 | 3.288267453960641e-01 | 4.754615224550794e-01 |
| 6 | 5.047201153812862e-02 | 4.434172288616122e-02 | 3.571861455046850e-01 | 5.984721316091538e-01 |
| 6 | 2.366397889251860e-02 | 2.233566593019009e-02 | 1.506515502460172e-01 | 8.270127838237927e-01 |
| 6 | 5.014212647237021e-03 | 2.764e-02-i*2.224e-02 | 2.764e-02+i*2.224e-02 | 9.447130224184685e-01 |

$d = 11$, $n_p = 30$, type $[0,2,4]$, quality PC

| | | | | |
|---|---|---|---|---|
| 3 | 1.422463935651383e-02 | 9.338481576932990e-01 | 3.307592115335049e-02 | 3.307592115335049e-02 |
| 3 | 4.623750003909563e-03 | -3.054757387024414e-02 | 5.152737869351221e-01 | 5.152737869351221e-01 |
| 6 | 5.018785346248799e-02 | 2.080871590250023e-01 | 3.227984515431529e-01 | 4.691143894318447e-01 |
| 6 | 6.285533119845694e-02 | 6.422980026053753e-02 | 3.399267106021509e-01 | 5.958434891373115e-01 |
| 6 | 3.030272389034122e-02 | 3.069068302710457e-02 | 1.714121195537683e-01 | 7.978971974191271e-01 |
| 6 | 1.389656343516883e-02 | 1.467e-01-i*7.243e-02 | 1.467e-01+i*7.243e-02 | 7.065288644742932e-01 |

$d = 11$, $n_p = 30$, type $[0,2,4]$, quality NC

| | | | | |
|---|---|---|---|---|
| 3 | 9.898681848451233e-02 | 1.908151662677124e-01 | 4.045924168661438e-01 | 4.045924168661438e-01 |
| 3 | -3.982563183797605e-12 | 3.207079107298070e+00 | -1.103539553649035e+00 | -1.103539553649035e+00 |
| 6 | 4.572817987670809e-02 | 1.324104070457752e-01 | 2.086461363392200e-01 | 6.589434566150048e-01 |
| 6 | 4.394919210980262e-02 | 3.502054609135649e-02 | 3.570053553874323e-01 | 6.079740985212112e-01 |
| 6 | 2.668109429825323e-02 | 2.294491738641314e-02 | 1.213165401247856e-01 | 8.557385424888013e-01 |
| 6 | 8.147911416378308e-04 | -6.951e-03-i*4.539e-02 | -6.951e-03+i*4.539e-02 | 1.013901550610228e+00 |

$d = 11$, $n_p = 30$, type $[0,2,4]$, quality NC

| | | | | |
|---|---|---|---|---|
| 3 | 5.310896597712391e-02 | 3.751478729962652e-02 | 4.812426063501867e-01 | 4.812426063501867e-01 |
| 3 | 2.473228822923786e-02 | 9.121918678936203e-01 | 4.390406605318983e-02 | 4.390406605318983e-02 |
| 6 | 6.708071324597394e-02 | 1.923151040105270e-01 | 3.094309776450466e-01 | 4.982539183444265e-01 |
| 6 | 6.040125803758637e-02 | 5.722160192248993e-02 | 2.168190288925455e-01 | 7.259593691849645e-01 |
| 6 | 2.640682799276180e-04 | -1.352447942367976e-01 | 2.392445766821049e-01 | 8.960002175546927e-01 |
| 6 | -2.144326813939148e-15 | -6.177083728221061e-01 | 8.089e-01-i*4.991e+00 | 8.089e-01+i*4.991e+00 |

$d = 11$, $n_p = 30$, type $[0,2,4]$, quality CC

| | | | | |
|---|---|---|---|---|
| 3 | 9.406e-02-i*1.448e-02 | 4.913e-01-i*1.087e-02 | 2.543e-01+i*5.437e-03 | 2.543e-01+i*5.437e-03 |
| 3 | 6.793e-02-i*1.483e-02 | 8.911e-02+i*2.425e-02 | 4.554e-01-i*1.212e-02 | 4.554e-01-i*1.212e-02 |
| 6 | 1.959e-02+i*1.505e-02 | 1.593e-02+i*1.886e-02 | 3.553e-01+i*9.909e-03 | 6.288e-01-i*2.877e-02 |
| 6 | 5.555e-02-i*5.407e-03 | 7.222e-02+i*1.659e-02 | 2.011e-01+i*3.972e-03 | 7.267e-01-i*2.056e-02 |
| 6 | -5.465e-04+i*1.089e-03 | -3.944e-03+i*5.613e-02 | 1.765e-01+i*1.432e-01 | 8.274e-01-i*1.994e-01 |
| 6 | 1.108e-02+i*3.919e-03 | 1.243e-02-i*2.707e-03 | 6.965e-02+i*1.710e-02 | 9.179e-01-i*1.440e-02 |

$d = 11$, $n_p = 30$, type $[0, 2, 4]$, quality CC

| | | | | |
|---|---|---|---|---|
| 3 | 9.406e-02+i*1.448e-02 | 4.913e-01+i*1.087e-02 | 2.543e-01-i*5.437e-03 | 2.543e-01-i*5.437e-03 |
| 3 | 6.793e-02+i*1.483e-02 | 8.911e-02-i*2.425e-02 | 4.554e-01+i*1.212e-02 | 4.554e-01+i*1.212e-02 |
| 6 | 1.959e-02-i*1.505e-02 | 1.593e-02-i*1.886e-02 | 3.553e-01-i*9.909e-03 | 6.288e-01+i*2.877e-02 |
| 6 | 5.555e-02+i*5.407e-03 | 7.222e-02-i*1.659e-02 | 2.011e-01-i*3.972e-03 | 7.267e-01+i*2.056e-02 |
| 6 | -5.465e-04-i*1.089e-03 | -3.944e-03-i*5.613e-02 | 1.765e-01-i*1.432e-01 | 8.274e-01+i*1.994e-01 |
| 6 | 1.108e-02-i*3.919e-03 | 1.243e-02+i*2.707e-03 | 6.965e-02-i*1.710e-02 | 9.179e-01+i*1.440e-02 |

$d = 11$, $n_p = 30$, type $[0, 2, 4]$, quality CC

| | | | | |
|---|---|---|---|---|
| 3 | 3.318e-02-i*1.709e-02 | 2.554e-01+i*6.131e-02 | 3.723e-01-i*3.066e-02 | 3.723e-01-i*3.066e-02 |
| 3 | 2.195e-02+i*1.313e-03 | -7.026e-03-i*8.332e-03 | 5.035e-01+i*4.166e-03 | 5.035e-01+i*4.166e-03 |
| 6 | 8.402e-02+i*5.956e-03 | 1.240e-01+i*9.216e-03 | 3.205e-01+i*4.760e-03 | 5.555e-01-i*1.398e-02 |
| 6 | 3.558e-04+i*1.084e-04 | -7.378e-02+i*8.736e-02 | 3.844e-01-i*2.318e-01 | 6.894e-01+i*1.444e-01 |
| 6 | 4.575e-02+i*1.523e-03 | 4.943e-02+i*3.615e-03 | 1.850e-01+i*1.463e-04 | 7.656e-01-i*3.762e-03 |
| 6 | 8.978e-03+i*2.999e-04 | 1.400e-02-i*1.185e-03 | 6.007e-02+i*2.427e-03 | 9.259e-01-i*1.242e-03 |

$d = 11$, $n_p = 30$, type $[0, 2, 4]$, quality CC

| | | | | |
|---|---|---|---|---|
| 3 | 3.318e-02+i*1.709e-02 | 2.554e-01-i*6.131e-02 | 3.723e-01+i*3.066e-02 | 3.723e-01+i*3.066e-02 |
| 3 | 2.195e-02-i*1.313e-03 | -7.026e-03+i*8.332e-03 | 5.035e-01-i*4.166e-03 | 5.035e-01-i*4.166e-03 |
| 6 | 8.402e-02-i*5.956e-03 | 1.240e-01-i*9.216e-03 | 3.205e-01-i*4.760e-03 | 5.555e-01+i*1.398e-02 |
| 6 | 3.558e-04-i*1.084e-04 | -7.378e-02-i*8.736e-02 | 3.844e-01+i*2.318e-01 | 6.894e-01-i*1.444e-01 |
| 6 | 4.575e-02-i*1.523e-03 | 4.943e-02-i*3.615e-03 | 1.850e-01-i*1.463e-04 | 7.656e-01+i*3.762e-03 |
| 6 | 8.978e-03-i*2.999e-04 | 1.400e-02+i*1.185e-03 | 6.007e-02-i*2.427e-03 | 9.259e-01+i*1.242e-03 |

$d = 11$, $n_p = 30$, type $[0, 2, 4]$, quality CC

| | | | | |
|---|---|---|---|---|
| 3 | 2.125e-02-i*2.241e-03 | 3.176e-01+i*7.184e-02 | 3.412e-01-i*3.592e-02 | 3.412e-01-i*3.592e-02 |
| 3 | 4.400e-02-i*4.476e-04 | 7.343e-01+i*2.734e-03 | 1.329e-01-i*1.367e-03 | 1.329e-01-i*1.367e-03 |
| 6 | 6.960e-02+i*1.132e-03 | 1.505e-01+i*1.876e-03 | 3.180e-01-i*1.529e-03 | 5.315e-01-i*3.470e-04 |
| 6 | 3.255e-02+i*2.070e-04 | 2.942e-02+i*3.740e-04 | 3.747e-01+i*5.617e-04 | 5.959e-01-i*9.357e-04 |
| 6 | 2.393e-02-i*1.056e-04 | 2.762e-02-i*3.434e-05 | 1.774e-01+i*1.709e-03 | 7.950e-01-i*1.674e-03 |
| 6 | 7.961e-03+i*1.111e-04 | 2.102e-02-i*6.377e-04 | 4.908e-02+i*1.086e-03 | 9.299e-01-i*4.481e-04 |

$d = 11$, $n_p = 30$, type $[0, 2, 4]$, quality CC

| | | | | |
|---|---|---|---|---|
| 3 | 2.125e-02+i*2.241e-03 | 3.176e-01-i*7.184e-02 | 3.412e-01+i*3.592e-02 | 3.412e-01+i*3.592e-02 |
| 3 | 4.400e-02+i*4.476e-04 | 7.343e-01-i*2.734e-03 | 1.329e-01+i*1.367e-03 | 1.329e-01+i*1.367e-03 |
| 6 | 6.960e-02-i*1.132e-03 | 1.505e-01-i*1.876e-03 | 3.180e-01+i*1.529e-03 | 5.315e-01+i*3.470e-04 |
| 6 | 3.255e-02-i*2.070e-04 | 2.942e-02-i*3.740e-04 | 3.747e-01-i*5.617e-04 | 5.959e-01+i*9.357e-04 |
| 6 | 2.393e-02+i*1.056e-04 | 2.762e-02+i*3.434e-05 | 1.774e-01-i*1.709e-03 | 7.950e-01+i*1.674e-03 |
| 6 | 7.961e-03-i*1.111e-04 | 2.102e-02+i*6.377e-04 | 4.908e-02-i*1.086e-03 | 9.299e-01+i*4.481e-04 |

$d = 11$, $n_p = 30$, type $[0, 2, 4]$, quality CC

| | | | | |
|---|---|---|---|---|
| 3 | -7.494e-03+i*2.841e-02 | 4.705e-01+i*1.332e-01 | 2.647e-01-i*6.660e-02 | 2.647e-01-i*6.660e-02 |
| 3 | 3.998e-02-i*1.050e-03 | 3.138e-02+i*3.221e-03 | 4.843e-01-i*1.610e-03 | 4.843e-01-i*1.610e-03 |
| 6 | 8.981e-02-i*8.641e-03 | 1.626e-01-i*1.977e-02 | 2.960e-01-i*1.288e-02 | 5.413e-01+i*3.265e-02 |
| 6 | 2.774e-02-i*2.077e-02 | 3.009e-02-i*1.448e-02 | 2.444e-01+i*3.197e-02 | 7.255e-01-i*1.749e-02 |
| 6 | 2.510e-02+i*1.584e-02 | 5.966e-02-i*2.186e-02 | 1.486e-01+i*3.771e-02 | 7.917e-01-i*1.586e-02 |
| 6 | 7.769e-03-i*1.116e-04 | 4.896e-03+i*4.772e-03 | 6.428e-02-i*5.652e-03 | 9.308e-01+i*8.796e-04 |

$d = 11$, $n_p = 30$, type $[0, 2, 4]$, quality CC

| | | | | |
|---|---|---|---|---|
| 3 | -7.494e-03-i*2.841e-02 | 4.705e-01-i*1.332e-01 | 2.647e-01+i*6.660e-02 | 2.647e-01+i*6.660e-02 |
| 3 | 3.998e-02+i*1.050e-03 | 3.138e-02-i*3.221e-03 | 4.843e-01+i*1.610e-03 | 4.843e-01+i*1.610e-03 |
| 6 | 8.981e-02+i*8.641e-03 | 1.626e-01+i*1.977e-02 | 2.960e-01+i*1.288e-02 | 5.413e-01-i*3.265e-02 |
| 6 | 2.774e-02+i*2.077e-02 | 3.009e-02+i*1.448e-02 | 2.444e-01-i*3.197e-02 | 7.255e-01+i*1.749e-02 |
| 6 | 2.510e-02-i*1.584e-02 | 5.966e-02+i*2.186e-02 | 1.486e-01-i*3.771e-02 | 7.917e-01+i*1.586e-02 |
| 6 | 7.769e-03+i*1.116e-04 | 4.896e-03-i*4.772e-03 | 6.428e-02+i*5.652e-03 | 9.308e-01-i*8.796e-04 |

$d = 11$, $n_p = 30$, type $[0, 2, 4]$, quality CC

| | | | | |
|---|---|---|---|---|
| 3 | 9.241e-02-i*5.968e-03 | 1.920e-01+i*3.600e-03 | 4.040e-01-i*1.800e-03 | 4.040e-01-i*1.800e-03 |
| 3 | 7.421e-02-i*3.623e-03 | 6.336e-01-i*1.528e-02 | 1.832e-01+i*7.639e-03 | 1.832e-01+i*7.639e-03 |
| 6 | 4.617e-02+i*4.804e-04 | 3.915e-02+i*2.371e-03 | 3.609e-01+i*3.365e-03 | 5.999e-01-i*5.735e-03 |
| 6 | 3.148e-02+i*2.973e-03 | 3.648e-02+i*5.872e-03 | 1.550e-01+i*9.091e-03 | 8.085e-01-i*1.496e-02 |
| 6 | -4.373e-06-i*1.828e-05 | -1.529e-01+i*2.119e-01 | 3.463e-01-i*7.933e-02 | 8.066e-01-i*1.325e-01 |
| 6 | 5.710e-03+i*1.361e-03 | 1.637e-02-i*5.921e-03 | 4.292e-02+i*1.375e-02 | 9.407e-01-i*7.833e-03 |

$d = 11$, $n_p = 30$, type $[0, 2, 4]$, quality CC

| | | | | |
|---|---|---|---|---|
| 3 | 9.241e-02+i*5.968e-03 | 1.920e-01-i*3.600e-03 | 4.040e-01+i*1.800e-03 | 4.040e-01+i*1.800e-03 |
| 3 | 7.421e-02+i*3.623e-03 | 6.336e-01+i*1.528e-02 | 1.832e-01-i*7.639e-03 | 1.832e-01-i*7.639e-03 |
| 6 | 4.617e-02-i*4.804e-04 | 3.915e-02-i*2.371e-03 | 3.609e-01-i*3.365e-03 | 5.999e-01+i*5.735e-03 |
| 6 | 3.148e-02-i*2.973e-03 | 3.648e-02-i*5.872e-03 | 1.550e-01-i*9.091e-03 | 8.085e-01+i*1.496e-02 |
| 6 | -4.373e-06+i*1.828e-05 | -1.529e-01-i*2.119e-01 | 3.463e-01+i*7.933e-02 | 8.066e-01+i*1.325e-01 |
| 6 | 5.710e-03-i*1.361e-03 | 1.637e-02+i*5.921e-03 | 4.292e-02-i*1.375e-02 | 9.407e-01+i*7.833e-03 |

$d = 11$, $n_p = 30$, type $[0, 2, 4]$, quality CC

| | | | | |
|---|---|---|---|---|
| 3 | 7.369e-02-i*8.283e-04 | 2.127e-01+i*4.700e-04 | 3.936e-01-i*2.350e-04 | 3.936e-01-i*2.350e-04 |
| 3 | 5.287e-02+i*1.343e-02 | 8.880e-01-i*3.015e-02 | 5.598e-02+i*1.507e-02 | 5.598e-02+i*1.507e-02 |
| 6 | 2.358e-03+i*5.774e-03 | 4.299e-02-i*2.913e-03 | 3.846e-01-i*1.740e-01 | 5.724e-01+i*1.769e-01 |
| 6 | 6.529e-02-i*2.021e-03 | 1.189e-01+i*1.722e-03 | 2.633e-01+i*1.813e-03 | 6.177e-01-i*3.535e-03 |
| 6 | 3.972e-02-i*7.390e-03 | 2.482e-02-i*2.441e-03 | 3.000e-01-i*7.217e-03 | 6.752e-01+i*9.658e-03 |
| 6 | -3.979e-03-i*2.664e-03 | 2.222e-02+i*8.805e-02 | 5.538e-02+i*3.338e-03 | 9.224e-01-i*9.139e-02 |

$d = 11$, $n_p = 30$, type $[0, 2, 4]$, quality CC

| | | | | |
|---|---|---|---|---|
| 3 | 7.369e-02+i*8.283e-04 | 2.127e-01-i*4.700e-04 | 3.936e-01+i*2.350e-04 | 3.936e-01+i*2.350e-04 |
| 3 | 5.287e-02-i*1.343e-02 | 8.880e-01+i*3.015e-02 | 5.598e-02-i*1.507e-02 | 5.598e-02-i*1.507e-02 |
| 6 | 2.358e-03-i*5.774e-03 | 4.299e-02+i*2.913e-03 | 3.846e-01+i*1.740e-01 | 5.724e-01-i*1.769e-01 |
| 6 | 6.529e-02+i*2.021e-03 | 1.189e-01-i*1.722e-03 | 2.633e-01-i*1.813e-03 | 6.177e-01+i*3.535e-03 |
| 6 | 3.972e-02+i*7.390e-03 | 2.482e-02+i*2.441e-03 | 3.000e-01+i*7.217e-03 | 6.752e-01-i*9.658e-03 |
| 6 | -3.979e-03+i*2.664e-03 | 2.222e-02-i*8.805e-02 | 5.538e-02-i*3.338e-03 | 9.224e-01+i*9.139e-02 |

$d = 11$, $n_p = 30$, type $[0, 2, 4]$, quality CC

| | | | | |
|---|---|---|---|---|
| 3 | -1.309e-01+i*5.891e-02 | 5.278e-01+i*1.092e-01 | 2.361e-01-i*5.458e-02 | 2.361e-01-i*5.458e-02 |
| 3 | 1.315e-03-i*7.013e-02 | 8.981e-01+i*5.548e-02 | 5.095e-02-i*2.774e-02 | 5.095e-02-i*2.774e-02 |
| 6 | 1.518e-01-i*1.871e-02 | 1.829e-01-i*3.617e-02 | 2.738e-01-i*2.861e-02 | 5.433e-01+i*6.478e-02 |
| 6 | 5.047e-02-i*1.236e-03 | 3.357e-02-i*3.486e-03 | 3.320e-01-i*9.768e-03 | 6.344e-01+i*1.325e-02 |
| 6 | 2.916e-02+i*2.557e-02 | 4.925e-02-i*1.400e-02 | 8.488e-02-i*6.333e-02 | 8.659e-01+i*7.733e-02 |
| 6 | 1.669e-05-i*1.845e-05 | 5.718e-02+i*2.471e-02 | 3.404e-01+i*4.933e-01 | 6.024e-01-i*5.180e-01 |

$d = 11$, $n_p = 30$, type $[0, 2, 4]$, quality CC

| | | | | |
|---|---|---|---|---|
| 3 | -1.309e-01-i*5.891e-02 | 5.278e-01-i*1.092e-01 | 2.361e-01+i*5.458e-02 | 2.361e-01+i*5.458e-02 |
| 3 | 1.315e-03+i*7.013e-02 | 8.981e-01-i*5.548e-02 | 5.095e-02+i*2.774e-02 | 5.095e-02+i*2.774e-02 |
| 6 | 1.518e-01+i*1.871e-02 | 1.829e-01+i*3.617e-02 | 2.738e-01+i*2.861e-02 | 5.433e-01-i*6.478e-02 |
| 6 | 5.047e-02+i*1.236e-03 | 3.357e-02+i*3.486e-03 | 3.320e-01+i*9.768e-03 | 6.344e-01-i*1.325e-02 |
| 6 | 2.916e-02-i*2.557e-02 | 4.925e-02+i*1.400e-02 | 8.488e-02+i*6.333e-02 | 8.659e-01-i*7.733e-02 |
| 6 | 1.669e-05+i*1.845e-05 | 5.718e-02-i*2.471e-02 | 3.404e-01-i*4.933e-01 | 6.024e-01+i*5.180e-01 |

$d = 11$, $n_p = 30$, type $[0, 2, 4]$, quality CC

| | | | | |
|---|---|---|---|---|
| 3 | 9.838e-03+i*1.081e-02 | 2.641e-01-i*1.128e-01 | 3.680e-01+i*5.642e-02 | 3.680e-01+i*5.642e-02 |
| 3 | 1.424e-02-i*2.201e-04 | 9.333e-01+i*6.005e-04 | 3.336e-02-i*3.003e-04 | 3.336e-02-i*3.003e-04 |
| 6 | 7.154e-02-i*4.001e-03 | 1.585e-01-i*1.024e-02 | 3.251e-01+i*3.708e-03 | 5.164e-01+i*6.527e-03 |
| 6 | 3.437e-02-i*1.691e-03 | 2.973e-02-i*1.572e-03 | 3.701e-01+i*4.522e-05 | 6.002e-01+i*1.527e-03 |
| 6 | 2.868e-02-i*2.032e-03 | 1.032e-01+i*8.680e-03 | 1.684e-01-i*2.035e-03 | 7.284e-01-i*6.646e-03 |
| 6 | 2.004e-02+i*2.430e-03 | 2.269e-02+i*2.918e-03 | 1.653e-01-i*3.859e-04 | 8.120e-01-i*2.532e-03 |

$d = 11$, $n_p = 30$, type $[0, 2, 4]$, quality CC

| | | | | |
|---|---|---|---|---|
| 3 | 9.838e-03-i*1.081e-02 | 2.641e-01+i*1.128e-01 | 3.680e-01-i*5.642e-02 | 3.680e-01-i*5.642e-02 |
| 3 | 1.424e-02+i*2.201e-04 | 9.333e-01-i*6.005e-04 | 3.336e-02+i*3.003e-04 | 3.336e-02+i*3.003e-04 |
| 6 | 7.154e-02+i*4.001e-03 | 1.585e-01+i*1.024e-02 | 3.251e-01-i*3.708e-03 | 5.164e-01-i*6.527e-03 |
| 6 | 3.437e-02+i*1.691e-03 | 2.973e-02+i*1.572e-03 | 3.701e-01-i*4.522e-05 | 6.002e-01-i*1.527e-03 |
| 6 | 2.868e-02+i*2.032e-03 | 1.032e-01-i*8.680e-03 | 1.684e-01+i*2.035e-03 | 7.284e-01+i*6.646e-03 |
| 6 | 2.004e-02-i*2.430e-03 | 2.269e-02-i*2.918e-03 | 1.653e-01+i*3.859e-04 | 8.120e-01+i*2.532e-03 |

$d = 11$, $n_p = 30$, type $[0, 2, 4]$, quality CC

| | | | | |
|---|---|---|---|---|
| 3 | 6.182e-02-i*2.492e-02 | 6.368e-01+i*4.111e-02 | 1.816e-01-i*2.055e-02 | 1.816e-01-i*2.055e-02 |
| 3 | 1.117e-02+i*1.317e-03 | 9.420e-01-i*4.469e-03 | 2.902e-02+i*2.235e-03 | 2.902e-02+i*2.235e-03 |
| 6 | 5.314e-02+i*1.294e-02 | 1.911e-01+i*1.749e-03 | 3.386e-01-i*4.082e-02 | 4.703e-01+i*3.907e-02 |
| 6 | 4.501e-02+i*8.196e-04 | 3.827e-02+i*2.185e-03 | 3.622e-01+i*2.248e-03 | 5.995e-01-i*4.434e-03 |
| 6 | 3.203e-02-i*1.949e-03 | 3.665e-02-i*1.944e-03 | 1.543e-01+i*3.836e-03 | 8.091e-01-i*1.892e-03 |
| 6 | -2.417e-06-i*8.823e-06 | -1.795e-01+i*2.362e-01 | 3.730e-01-i*4.376e-02 | 8.065e-01-i*1.924e-01 |

$d = 11$, $n_p = 30$, type $[0, 2, 4]$, quality CC

| | | | | |
|---|---|---|---|---|
| 3 | 6.182e-02+i*2.492e-02 | 6.368e-01-i*4.111e-02 | 1.816e-01+i*2.055e-02 | 1.816e-01+i*2.055e-02 |
| 3 | 1.117e-02-i*1.317e-03 | 9.420e-01+i*4.469e-03 | 2.902e-02-i*2.235e-03 | 2.902e-02-i*2.235e-03 |
| 6 | 5.314e-02-i*1.294e-02 | 1.911e-01-i*1.749e-03 | 3.386e-01+i*4.082e-02 | 4.703e-01-i*3.907e-02 |
| 6 | 4.501e-02-i*8.196e-04 | 3.827e-02-i*2.185e-03 | 3.622e-01-i*2.248e-03 | 5.995e-01+i*4.434e-03 |
| 6 | 3.203e-02+i*1.949e-03 | 3.665e-02+i*1.944e-03 | 1.543e-01-i*3.836e-03 | 8.091e-01+i*1.892e-03 |
| 6 | -2.417e-06+i*8.823e-06 | -1.795e-01-i*2.362e-01 | 3.730e-01+i*4.376e-02 | 8.065e-01+i*1.924e-01 |

$d = 11$, $n_p = 30$, type $[0, 2, 4]$, quality CC

| | | | | |
|---|---|---|---|---|
| 3 | 5.235e-02-i*2.868e-03 | 4.958e-02-i*3.967e-04 | 4.752e-01+i*1.983e-04 | 4.752e-01+i*1.983e-04 |
| 3 | -5.579e-04+i*2.566e-03 | 9.799e-01-i*5.266e-02 | 1.003e-02+i*2.633e-02 | 1.003e-02+i*2.633e-02 |
| 6 | 5.547e-02-i*2.339e-03 | 2.017e-01+i*7.021e-04 | 3.212e-01+i*5.460e-03 | 4.771e-01-i*6.162e-03 |
| 6 | 5.610e-02-i*2.273e-03 | 8.422e-02+i*7.937e-03 | 2.273e-01+i*6.822e-03 | 6.884e-01-i*1.476e-02 |
| 6 | 9.134e-03+i*2.186e-03 | -5.607e-03+i*6.786e-03 | 3.048e-01+i*1.419e-03 | 7.008e-01-i*8.205e-03 |
| 6 | 2.006e-02+i*2.577e-03 | 2.704e-02+i*5.454e-03 | 9.309e-02+i*1.700e-02 | 8.799e-01-i*2.245e-02 |

$d = 11$, $n_p = 30$, type $[0, 2, 4]$, quality CC

| | | | | |
|---|---|---|---|---|
| 3 | 5.235e-02+i*2.868e-03 | 4.958e-02+i*3.967e-04 | 4.752e-01-i*1.983e-04 | 4.752e-01-i*1.983e-04 |
| 3 | -5.579e-04-i*2.566e-03 | 9.799e-01+i*5.266e-02 | 1.003e-02-i*2.633e-02 | 1.003e-02-i*2.633e-02 |
| 6 | 5.547e-02+i*2.339e-03 | 2.017e-01-i*7.021e-04 | 3.212e-01-i*5.460e-03 | 4.771e-01+i*6.162e-03 |
| 6 | 5.610e-02+i*2.273e-03 | 8.422e-02-i*7.937e-03 | 2.273e-01-i*6.822e-03 | 6.884e-01+i*1.476e-02 |
| 6 | 9.134e-03-i*2.186e-03 | -5.607e-03-i*6.786e-03 | 3.048e-01-i*1.419e-03 | 7.008e-01+i*8.205e-03 |
| 6 | 2.006e-02-i*2.577e-03 | 2.704e-02-i*5.454e-03 | 9.309e-02-i*1.700e-02 | 8.799e-01+i*2.245e-02 |

$d = 11$, $n_p = 30$, type $[0, 2, 4]$, quality CC

| | | | | |
|---|---|---|---|---|
| 3 | -4.592e-02-i*6.340e-02 | 5.071e-01-i*1.126e-01 | 2.464e-01+i*5.628e-02 | 2.464e-01+i*5.628e-02 |
| 3 | 4.767e-02+i*6.666e-03 | 8.699e-01-i*5.428e-03 | 6.504e-02+i*2.714e-03 | 6.504e-02+i*2.714e-03 |
| 6 | 1.102e-01+i*2.215e-02 | 1.708e-01+i*3.405e-02 | 2.810e-01+i*1.810e-02 | 5.482e-01-i*5.215e-02 |
| 6 | -2.485e-03-i*1.916e-03 | 4.141e-02-i*3.025e-03 | 3.298e-01+i*2.272e-01 | 6.288e-01-i*2.241e-01 |
| 6 | 5.783e-02+i*8.324e-03 | 3.366e-02+i*4.781e-03 | 3.067e-01+i*1.906e-02 | 6.596e-01-i*2.384e-02 |
| 6 | 2.881e-04-i*1.961e-04 | -1.015e-01-i*3.824e-02 | 6.563e-02+i*4.798e-03 | 1.036e+00+i*3.344e-02 |

$d = 11$, $n_p = 30$, type $[0, 2, 4]$, quality CC

| | | | | |
|---|---|---|---|---|
| 3 | -4.592e-02+i*6.340e-02 | 5.071e-01+i*1.126e-01 | 2.464e-01-i*5.628e-02 | 2.464e-01-i*5.628e-02 |
| 3 | 4.767e-02-i*6.666e-03 | 8.699e-01+i*5.428e-03 | 6.504e-02-i*2.714e-03 | 6.504e-02-i*2.714e-03 |
| 6 | 1.102e-01-i*2.215e-02 | 1.708e-01-i*3.405e-02 | 2.810e-01-i*1.810e-02 | 5.482e-01+i*5.215e-02 |
| 6 | -2.485e-03+i*1.916e-03 | 4.141e-02+i*3.025e-03 | 3.298e-01-i*2.272e-01 | 6.288e-01+i*2.241e-01 |
| 6 | 5.783e-02-i*8.324e-03 | 3.366e-02-i*4.781e-03 | 3.067e-01-i*1.906e-02 | 6.596e-01+i*2.384e-02 |
| 6 | 2.881e-04+i*1.961e-04 | -1.015e-01+i*3.824e-02 | 6.563e-02-i*4.798e-03 | 1.036e+00-i*3.344e-02 |

$d = 12$, $n_p = 33$, type $[0, 5, 3]$, quality PI

| | | | | |
|---|---|---|---|---|
| 3 | 6.254121319590276e-02 | 4.570749859701478e-01 | 2.714625070149261e-01 | 2.714625070149261e-01 |
| 3 | 4.991833492806094e-02 | 1.197767026828138e-01 | 4.401116486585931e-01 | 4.401116486585931e-01 |
| 3 | 2.426683808145203e-02 | 2.359249810891690e-02 | 4.882037509455416e-01 | 4.882037509455416e-01 |
| 3 | 2.848605206887754e-02 | 7.814843446812914e-01 | 1.092578276593543e-01 | 1.092578276593543e-01 |
| 3 | 7.931642509973638e-03 | 9.507072731273288e-01 | 2.464636343633559e-02 | 2.464636343633559e-02 |
| 6 | 4.322736365941421e-02 | 1.162960196779266e-01 | 2.554542286385173e-01 | 6.282497516835561e-01 |
| 6 | 2.178358503860756e-02 | 2.303415635526714e-02 | 2.916556797383410e-01 | 6.853101639063919e-01 |
| 6 | 1.508367757651144e-02 | 2.138249025617059e-02 | 1.272797172335894e-01 | 8.513377925102400e-01 |

$d = 12$, $n_p = 33$, type $[0, 5, 3]$, quality PI

| | | | | |
|---|---|---|---|---|
| 3 | 6.285822421788510e-02 | 4.575792299757682e-01 | 2.712103850121159e-01 | 2.712103850121159e-01 |
| 3 | 4.369254453803840e-02 | 1.205512154110795e-01 | 4.397243922944603e-01 | 4.397243922944603e-01 |
| 3 | 2.573106644045534e-02 | 2.356522045239023e-02 | 4.882173897738049e-01 | 4.882173897738049e-01 |
| 3 | 3.479611293070894e-02 | 7.448477089168282e-01 | 1.275761455415859e-01 | 1.275761455415859e-01 |
| 3 | 6.166261051559017e-03 | 9.573652990935793e-01 | 2.131735045321037e-02 | 2.131735045321037e-02 |
| 6 | 4.037155776638093e-02 | 1.153434945346980e-01 | 2.757132696855142e-01 | 6.089432357797878e-01 |
| 6 | 2.235677320230345e-02 | 2.283833222225703e-02 | 2.813255809899395e-01 | 6.958360867878034e-01 |
| 6 | 1.731623110865889e-02 | 2.573405054833023e-02 | 1.162519159075971e-01 | 8.580140335440726e-01 |

$d = 12$, $n_p = 33$, type $[0, 5, 3]$, quality NI

| | | | | |
|---|---|---|---|---|
| 3 | 5.992157930040981e-02 | 4.529711389058645e-01 | 2.735144305470678e-01 | 2.735144305470678e-01 |
| 3 | 2.807875643954752e-02 | 2.368917770665134e-02 | 4.881554111466743e-01 | 4.881554111466743e-01 |
| 3 | 5.252899601772313e-02 | 7.321646206597614e-01 | 1.339176896701193e-01 | 1.339176896701193e-01 |
| 3 | 1.617355627623166e-03 | 9.927521106062486e-01 | 3.623944696875718e-03 | 3.623944696875718e-03 |
| 3 | -1.062024194350891e-01 | 8.745335893925173e-01 | 6.273320530374134e-02 | 6.273320530374134e-02 |
| 6 | 5.491810838782295e-02 | 1.202241316165672e-01 | 3.319346641205961e-01 | 5.478412042628367e-01 |
| 6 | 2.544555194057983e-02 | 2.405691547178780e-02 | 2.633690807904016e-01 | 7.125740037378106e-01 |
| 6 | 6.833087236315665e-02 | 4.346701716737803e-02 | 7.887216477846390e-02 | 8.776608180541581e-01 |

$d = 12$, $n_p = 33$, type $[0, 5, 3]$, quality CC

| | | | | |
|---|---|---|---|---|
| 3 | 7.318e-02-i*4.171e-03 | 4.722e-01-i*5.382e-03 | 2.639e-01+i*2.691e-03 | 2.639e-01+i*2.691e-03 |
| 3 | 6.238e-02+i*4.489e-04 | 1.168e-01+i*2.775e-03 | 4.416e-01-i*1.387e-03 | 4.416e-01-i*1.387e-03 |
| 3 | -7.558e-04-i*6.772e-04 | 7.389e-01-i*2.239e-01 | 1.305e-01+i*1.119e-01 | 1.305e-01+i*1.119e-01 |
| 3 | 4.659e-04-i*3.914e-03 | 8.170e-01+i*1.357e-01 | 9.151e-02-i*6.787e-02 | 9.151e-02-i*6.787e-02 |
| 3 | 1.565e-02-i*1.824e-03 | 9.302e-01+i*4.340e-03 | 3.490e-02-i*2.170e-03 | 3.490e-02-i*2.170e-03 |
| 6 | 2.596e-02+i*1.054e-03 | 2.207e-02+i*1.006e-03 | 3.717e-01-i*5.474e-04 | 6.063e-01-i*4.588e-04 |
| 6 | 5.679e-02+i*4.302e-03 | 9.075e-02+i*1.858e-03 | 2.032e-01-i*5.380e-03 | 7.061e-01+i*3.522e-03 |
| 6 | 8.452e-03-i*2.878e-04 | 4.915e-04-i*9.745e-04 | 1.588e-01+i*6.462e-04 | 8.408e-01+i*3.284e-04 |

$d = 12$, $n_p = 33$, type $[0, 5, 3]$, quality CC

| | | | | |
|---|---|---|---|---|
| 3 | 7.318e-02+i*4.171e-03 | 4.722e-01+i*5.382e-03 | 2.639e-01-i*2.691e-03 | 2.639e-01-i*2.691e-03 |
| 3 | 6.238e-02-i*4.489e-04 | 1.168e-01-i*2.775e-03 | 4.416e-01+i*1.387e-03 | 4.416e-01+i*1.387e-03 |
| 3 | -7.558e-04+i*6.772e-04 | 7.389e-01+i*2.239e-01 | 1.305e-01-i*1.119e-01 | 1.305e-01-i*1.119e-01 |
| 3 | 4.659e-04+i*3.914e-03 | 8.170e-01-i*1.357e-01 | 9.151e-02+i*6.787e-02 | 9.151e-02+i*6.787e-02 |
| 3 | 1.565e-02+i*1.824e-03 | 9.302e-01-i*4.340e-03 | 3.490e-02+i*2.170e-03 | 3.490e-02+i*2.170e-03 |
| 6 | 2.596e-02-i*1.054e-03 | 2.207e-02-i*1.006e-03 | 3.717e-01+i*5.474e-04 | 6.063e-01+i*4.588e-04 |
| 6 | 5.679e-02-i*4.302e-03 | 9.075e-02-i*1.858e-03 | 2.032e-01+i*5.380e-03 | 7.061e-01-i*3.522e-03 |
| 6 | 8.452e-03+i*2.878e-04 | 4.915e-04+i*9.745e-04 | 1.588e-01-i*6.462e-04 | 8.408e-01-i*3.284e-04 |

$d = 12$, $n_p = 33$, type $[0, 5, 3]$, quality CC

| | | | | |
|---|---|---|---|---|
| 3 | 8.078e-02-i*5.509e-02 | 1.994e-01+i*3.597e-02 | 4.003e-01-i*1.798e-02 | 4.003e-01-i*1.798e-02 |
| 3 | 2.116e-02+i*4.208e-02 | 1.301e-01+i*6.277e-02 | 4.349e-01-i*3.139e-02 | 4.349e-01-i*3.139e-02 |
| 3 | 5.057e-02-i*2.184e-02 | 6.127e-01-i*5.061e-02 | 1.936e-01+i*2.530e-02 | 1.936e-01+i*2.530e-02 |
| 3 | 4.326e-02-i*7.297e-02 | 7.689e-01+i*4.282e-02 | 1.155e-01-i*2.141e-02 | 1.155e-01-i*2.141e-02 |
| 3 | 1.262e-02-i*5.534e-04 | 9.376e-01+i*1.498e-03 | 3.121e-02-i*7.490e-04 | 3.121e-02-i*7.490e-04 |
| 6 | 3.242e-02+i*7.480e-03 | 2.775e-02+i*6.016e-03 | 3.699e-01-i*2.234e-03 | 6.023e-01-i*3.781e-03 |
| 6 | 2.270e-02+i*4.993e-02 | 1.027e-01+i*1.478e-02 | 1.737e-01-i*4.952e-02 | 7.236e-01+i*3.474e-02 |
| 6 | 7.344e-03-i*3.221e-03 | -1.602e-03-i*1.131e-02 | 1.614e-01+i*6.030e-03 | 8.402e-01+i*5.279e-03 |

$d = 12$, $n_p = 33$, type $[0, 5, 3]$, quality CC

| | | | | |
|---|---|---|---|---|
| 3 | 8.078e-02+i*5.509e-02 | 1.994e-01-i*3.597e-02 | 4.003e-01+i*1.798e-02 | 4.003e-01+i*1.798e-02 |
| 3 | 2.116e-02-i*4.208e-02 | 1.301e-01-i*6.277e-02 | 4.349e-01+i*3.139e-02 | 4.349e-01+i*3.139e-02 |
| 3 | 5.057e-02+i*2.184e-02 | 6.127e-01+i*5.061e-02 | 1.936e-01-i*2.530e-02 | 1.936e-01-i*2.530e-02 |
| 3 | 4.326e-02+i*7.297e-02 | 7.689e-01-i*4.282e-02 | 1.155e-01+i*2.141e-02 | 1.155e-01+i*2.141e-02 |
| 3 | 1.262e-02+i*5.534e-04 | 9.376e-01-i*1.498e-03 | 3.121e-02+i*7.490e-04 | 3.121e-02+i*7.490e-04 |
| 6 | 3.242e-02-i*7.480e-03 | 2.775e-02-i*6.016e-03 | 3.699e-01+i*2.234e-03 | 6.023e-01+i*3.781e-03 |
| 6 | 2.270e-02-i*4.993e-02 | 1.027e-01-i*1.478e-02 | 1.737e-01+i*4.952e-02 | 7.236e-01-i*3.474e-02 |
| 6 | 7.344e-03+i*3.221e-03 | -1.602e-03+i*1.131e-02 | 1.614e-01-i*6.030e-03 | 8.402e-01-i*5.279e-03 |

$d = 12$, $n_p = 33$, type $[0, 5, 3]$, quality CC

| | | | | |
|---|---|---|---|---|
| 3 | 7.703e-02-i*1.045e-02 | 2.045e-01+i*9.835e-03 | 3.978e-01-i*4.918e-03 | 3.978e-01-i*4.918e-03 |
| 3 | 5.917e-02-i*7.145e-03 | 6.026e-01-i*1.239e-02 | 1.987e-01+i*6.197e-03 | 1.987e-01+i*6.197e-03 |
| 3 | 4.365e-02+i*6.095e-02 | 3.000e-02+i*3.283e-02 | 4.850e-01-i*1.642e-02 | 4.850e-01-i*1.642e-02 |
| 3 | 3.695e-02+i*3.728e-03 | 7.924e-01+i*1.060e-02 | 1.038e-01-i*5.300e-03 | 1.038e-01-i*5.300e-03 |
| 3 | 1.091e-02+i*1.260e-03 | 9.421e-01-i*2.941e-03 | 2.893e-02+i*1.470e-03 | 2.893e-02+i*1.470e-03 |
| 6 | 6.005e-02-i*2.381e-02 | 5.385e-02+i*2.762e-02 | 3.360e-01-i*3.075e-02 | 6.101e-01+i*3.129e-03 |
| 6 | -2.054e-02+i*1.402e-03 | 2.055e-02+i*4.101e-02 | 3.908e-01+i*5.614e-02 | 5.886e-01-i*9.715e-02 |
| 6 | 1.330e-02-i*1.765e-03 | 1.363e-02-i*8.600e-03 | 1.519e-01+i*2.101e-02 | 8.344e-01-i*1.241e-02 |

$d = 12$, $n_p = 33$, type $[0, 5, 3]$, quality CC

| | | | | |
|---|---|---|---|---|
| 3 | 7.703e-02+i*1.045e-02 | 2.045e-01-i*9.835e-03 | 3.978e-01+i*4.918e-03 | 3.978e-01+i*4.918e-03 |
| 3 | 5.917e-02+i*7.145e-03 | 6.026e-01+i*1.239e-02 | 1.987e-01-i*6.197e-03 | 1.987e-01-i*6.197e-03 |
| 3 | 4.365e-02-i*6.095e-02 | 3.000e-02-i*3.283e-02 | 4.850e-01+i*1.642e-02 | 4.850e-01+i*1.642e-02 |
| 3 | 3.695e-02-i*3.728e-03 | 7.924e-01-i*1.060e-02 | 1.038e-01+i*5.300e-03 | 1.038e-01+i*5.300e-03 |
| 3 | 1.091e-02-i*1.260e-03 | 9.421e-01+i*2.941e-03 | 2.893e-02-i*1.470e-03 | 2.893e-02-i*1.470e-03 |
| 6 | 6.005e-02+i*2.381e-02 | 5.385e-02-i*2.762e-02 | 3.360e-01+i*3.075e-02 | 6.101e-01-i*3.129e-03 |
| 6 | -2.054e-02-i*1.402e-03 | 2.055e-02-i*4.101e-02 | 3.908e-01-i*5.614e-02 | 5.886e-01+i*9.715e-02 |
| 6 | 1.330e-02+i*1.765e-03 | 1.363e-02+i*8.600e-03 | 1.519e-01-i*2.101e-02 | 8.344e-01+i*1.241e-02 |

$d = 12$, $n_p = 33$, type $[0, 5, 3]$, quality CC

| | | | | |
|---|---|---|---|---|
| 3 | 6.826e-02+i*1.030e-02 | 2.129e-01-i*8.235e-03 | 3.936e-01+i*4.117e-03 | 3.936e-01+i*4.117e-03 |
| 3 | 4.368e-02+i*1.886e-03 | 4.307e-02+i*2.888e-03 | 4.785e-01-i*1.444e-03 | 4.785e-01-i*1.444e-03 |
| 3 | 3.174e-02-i*7.519e-03 | 7.522e-01+i*3.852e-02 | 1.239e-01-i*1.926e-02 | 1.239e-01-i*1.926e-02 |
| 3 | 1.671e-04+i*1.655e-05 | -9.670e-02-i*2.710e-04 | 5.484e-01+i*1.355e-04 | 5.484e-01+i*1.355e-04 |
| 3 | 6.318e-03+i*2.379e-03 | 9.541e-01-i*9.678e-03 | 2.295e-02+i*4.839e-03 | 2.295e-02+i*4.839e-03 |
| 6 | 4.937e-02+i*4.382e-05 | 1.372e-01-i*3.082e-03 | 2.737e-01-i*2.338e-02 | 5.891e-01+i*2.646e-02 |
| 6 | 2.541e-02-i*1.201e-03 | 2.567e-02-i*4.616e-04 | 2.783e-01+i*7.134e-03 | 6.961e-01-i*6.673e-03 |
| 6 | 1.680e-02-i*2.376e-03 | 2.593e-02-i*3.568e-03 | 1.137e-01+i*1.029e-02 | 8.604e-01-i*6.726e-03 |

$d = 12$, $n_p = 33$, type $[0, 5, 3]$, quality CC

| | | | | |
|---|---|---|---|---|
| 3 | 6.826e-02-i*1.030e-02 | 2.129e-01+i*8.235e-03 | 3.936e-01-i*4.117e-03 | 3.936e-01-i*4.117e-03 |
| 3 | 4.368e-02-i*1.886e-03 | 4.307e-02-i*2.888e-03 | 4.785e-01+i*1.444e-03 | 4.785e-01+i*1.444e-03 |
| 3 | 3.174e-02+i*7.519e-03 | 7.522e-01-i*3.852e-02 | 1.239e-01+i*1.926e-02 | 1.239e-01+i*1.926e-02 |
| 3 | 1.671e-04-i*1.655e-05 | -9.670e-02+i*2.710e-04 | 5.484e-01-i*1.355e-04 | 5.484e-01-i*1.355e-04 |
| 3 | 6.318e-03-i*2.379e-03 | 9.541e-01+i*9.678e-03 | 2.295e-02-i*4.839e-03 | 2.295e-02-i*4.839e-03 |
| 6 | 4.937e-02-i*4.382e-05 | 1.372e-01+i*3.082e-03 | 2.737e-01+i*2.338e-02 | 5.891e-01-i*2.646e-02 |
| 6 | 2.541e-02+i*1.201e-03 | 2.567e-02+i*4.616e-04 | 2.783e-01-i*7.134e-03 | 6.961e-01+i*6.673e-03 |
| 6 | 1.680e-02+i*2.376e-03 | 2.593e-02+i*3.568e-03 | 1.137e-01-i*1.029e-02 | 8.604e-01+i*6.726e-03 |

$d = 12$, $n_p = 33$, type $[0, 5, 3]$, quality CC

| | | | | |
|---|---|---|---|---|
| 3 | 1.290e-02+i*6.152e-02 | 4.898e-01+i*6.899e-02 | 2.551e-01-i*3.449e-02 | 2.551e-01-i*3.449e-02 |
| 3 | 3.829e-02+i*1.275e-04 | 3.424e-02+i*5.851e-04 | 4.829e-01-i*2.926e-04 | 4.829e-01-i*2.926e-04 |
| 3 | 4.196e-02+i*1.059e-02 | 7.154e-01-i*2.956e-02 | 1.423e-01+i*1.478e-02 | 1.423e-01+i*1.478e-02 |
| 3 | -3.954e-05+i*4.436e-05 | 5.093e-02+i*2.919e-01 | 4.745e-01-i*1.459e-01 | 4.745e-01-i*1.459e-01 |
| 3 | 3.872e-03-i*9.973e-04 | 9.693e-01+i*8.018e-03 | 1.535e-02-i*4.009e-03 | 1.535e-02-i*4.009e-03 |
| 6 | 7.095e-02-i*3.595e-02 | 1.633e-01-i*2.233e-02 | 2.970e-01+i*1.070e-02 | 5.397e-01+i*1.163e-02 |
| 6 | 2.857e-02-i*1.178e-03 | 2.824e-02-i*1.287e-03 | 2.745e-01-i*1.427e-03 | 6.973e-01+i*2.715e-03 |
| 6 | 1.865e-02+i*1.482e-03 | 2.750e-02+i*1.646e-03 | 1.062e-01-i*2.696e-03 | 8.663e-01+i*1.050e-03 |

$d = 12$, $n_p = 33$, type $[0, 5, 3]$, quality CC

| | | | | |
|---|---|---|---|---|
| 3 | 1.290e-02-i*6.152e-02 | 4.898e-01-i*6.899e-02 | 2.551e-01+i*3.449e-02 | 2.551e-01+i*3.449e-02 |
| 3 | 3.829e-02-i*1.275e-04 | 3.424e-02-i*5.851e-04 | 4.829e-01+i*2.926e-04 | 4.829e-01+i*2.926e-04 |
| 3 | 4.196e-02-i*1.059e-02 | 7.154e-01+i*2.956e-02 | 1.423e-01-i*1.478e-02 | 1.423e-01-i*1.478e-02 |
| 3 | -3.954e-05-i*4.436e-05 | 5.093e-02-i*2.919e-01 | 4.745e-01+i*1.459e-01 | 4.745e-01+i*1.459e-01 |
| 3 | 3.872e-03+i*9.973e-04 | 9.693e-01-i*8.018e-03 | 1.535e-02+i*4.009e-03 | 1.535e-02+i*4.009e-03 |
| 6 | 7.095e-02+i*3.595e-02 | 1.633e-01+i*2.233e-02 | 2.970e-01-i*1.070e-02 | 5.397e-01-i*1.163e-02 |
| 6 | 2.857e-02+i*1.178e-03 | 2.824e-02+i*1.287e-03 | 2.745e-01+i*1.427e-03 | 6.973e-01-i*2.715e-03 |
| 6 | 1.865e-02-i*1.482e-03 | 2.750e-02-i*1.646e-03 | 1.062e-01+i*2.696e-03 | 8.663e-01-i*1.050e-03 |

$d = 12$, $n_p = 33$, type $[0, 5, 3]$, quality CC

| | | | | |
|---|---|---|---|---|
| 3 | 1.282e-01+i*6.330e-03 | 1.731e-01-i*1.956e-02 | 4.134e-01+i*9.782e-03 | 4.134e-01+i*9.782e-03 |
| 3 | -2.653e-02-i*1.036e-02 | 4.667e-01+i*1.853e-01 | 2.667e-01-i*9.265e-02 | 2.667e-01-i*9.265e-02 |
| 3 | 3.401e-02-i*5.259e-03 | 2.975e-02-i*4.196e-03 | 4.851e-01+i*2.098e-03 | 4.851e-01+i*2.098e-03 |
| 3 | 7.317e-02-i*6.923e-04 | 6.715e-01+i*3.776e-03 | 1.643e-01-i*1.888e-03 | 1.643e-01-i*1.888e-03 |
| 3 | 1.327e-03+i*1.385e-03 | 9.906e-01-i*2.504e-02 | 4.682e-03+i*1.252e-02 | 4.682e-03+i*1.252e-02 |
| 6 | 8.378e-03+i*6.332e-03 | 2.484e-01-i*1.686e-01 | 2.579e-01-i*1.416e-02 | 4.937e-01+i*1.828e-01 |
| 6 | 3.385e-02-i*2.411e-03 | 3.263e-02-i*1.890e-03 | 2.688e-01+i*3.810e-03 | 6.986e-01-i*1.920e-03 |
| 6 | 1.934e-02+i*3.784e-04 | 2.733e-02+i*1.404e-03 | 9.601e-02+i*7.081e-03 | 8.767e-01-i*8.484e-03 |

$d = 12$, $n_p = 33$, type $[0, 5, 3]$, quality CC

| | | | | |
|---|---|---|---|---|
| 3 | 1.282e-01-i*6.330e-03 | 1.731e-01+i*1.956e-02 | 4.134e-01-i*9.782e-03 | 4.134e-01-i*9.782e-03 |
| 3 | -2.653e-02+i*1.036e-02 | 4.667e-01-i*1.853e-01 | 2.667e-01+i*9.265e-02 | 2.667e-01+i*9.265e-02 |
| 3 | 3.401e-02+i*5.259e-03 | 2.975e-02+i*4.196e-03 | 4.851e-01-i*2.098e-03 | 4.851e-01-i*2.098e-03 |
| 3 | 7.317e-02+i*6.923e-04 | 6.715e-01-i*3.776e-03 | 1.643e-01+i*1.888e-03 | 1.643e-01+i*1.888e-03 |
| 3 | 1.327e-03-i*1.385e-03 | 9.906e-01+i*2.504e-02 | 4.682e-03-i*1.252e-02 | 4.682e-03-i*1.252e-02 |
| 6 | 8.378e-03-i*6.332e-03 | 2.484e-01+i*1.686e-01 | 2.579e-01+i*1.416e-02 | 4.937e-01-i*1.828e-01 |
| 6 | 3.385e-02+i*2.411e-03 | 3.263e-02+i*1.890e-03 | 2.688e-01-i*3.810e-03 | 6.986e-01+i*1.920e-03 |
| 6 | 1.934e-02-i*3.784e-04 | 2.733e-02-i*1.404e-03 | 9.601e-02-i*7.081e-03 | 8.767e-01+i*8.484e-03 |

$d = 12$, $n_p = 33$, type $[0, 5, 3]$, quality CC

| | | | | |
|---|---|---|---|---|
| 3 | 1.364e-02-i*1.167e-02 | 2.677e-01+i*1.015e-01 | 3.661e-01-i*5.076e-02 | 3.661e-01-i*5.076e-02 |
| 3 | 3.365e-02+i*1.559e-03 | 2.962e-02+i*1.585e-03 | 4.852e-01-i*7.925e-04 | 4.852e-01-i*7.925e-04 |
| 3 | 2.991e-02-i*4.812e-03 | 7.240e-01+i*5.862e-02 | 1.380e-01-i*2.931e-02 | 1.380e-01-i*2.931e-02 |
| 3 | 1.037e-03-i*3.155e-04 | 7.924e-01-i*2.017e-01 | 1.038e-01+i*1.008e-01 | 1.038e-01+i*1.008e-01 |
| 3 | 1.660e-03+i*8.234e-04 | 9.946e-01-i*1.409e-02 | 2.715e-03+i*7.043e-03 | 2.715e-03+i*7.043e-03 |
| 6 | 7.700e-02+i*8.868e-03 | 1.533e-01+i*8.905e-03 | 3.156e-01-i*7.660e-03 | 5.311e-01-i*1.245e-03 |
| 6 | 2.814e-02+i*4.664e-04 | 2.746e-02+i*6.193e-04 | 2.712e-01+i*1.558e-03 | 7.013e-01-i*2.177e-03 |
| 6 | 2.158e-02-i*2.125e-03 | 3.020e-02-i*1.659e-03 | 9.992e-02+i*3.251e-03 | 8.699e-01-i*1.592e-03 |

$d = 12$, $n_p = 33$, type $[0, 5, 3]$, quality CC

| | | | | |
|---|---|---|---|---|
| 3 | 1.364e-02+i*1.167e-02 | 2.677e-01-i*1.015e-01 | 3.661e-01+i*5.076e-02 | 3.661e-01+i*5.076e-02 |
| 3 | 3.365e-02-i*1.559e-03 | 2.962e-02-i*1.585e-03 | 4.852e-01+i*7.925e-04 | 4.852e-01+i*7.925e-04 |
| 3 | 2.991e-02+i*4.812e-03 | 7.240e-01-i*5.862e-02 | 1.380e-01+i*2.931e-02 | 1.380e-01+i*2.931e-02 |
| 3 | 1.037e-03+i*3.155e-04 | 7.924e-01+i*2.017e-01 | 1.038e-01-i*1.008e-01 | 1.038e-01-i*1.008e-01 |
| 3 | 1.660e-03-i*8.234e-04 | 9.946e-01+i*1.409e-02 | 2.715e-03-i*7.043e-03 | 2.715e-03-i*7.043e-03 |
| 6 | 7.700e-02-i*8.868e-03 | 1.533e-01-i*8.905e-03 | 3.156e-01+i*7.660e-03 | 5.311e-01+i*1.245e-03 |
| 6 | 2.814e-02-i*4.664e-04 | 2.746e-02-i*6.193e-04 | 2.712e-01-i*1.558e-03 | 7.013e-01+i*2.177e-03 |
| 6 | 2.158e-02+i*2.125e-03 | 3.020e-02+i*1.659e-03 | 9.992e-02-i*3.251e-03 | 8.699e-01+i*1.592e-03 |

$d = 12$, $n_p = 33$, type $[0, 5, 3]$, quality CC

| | | | | |
|---|---|---|---|---|
| 3 | 9.025491348658970e-02 | 1.934454805168219e-01 | 4.032772597415890e-01 | 4.032772597415890e-01 |
| 3 | 7.357128894764572e-02 | 6.294065278559098e-01 | 1.852967360720451e-01 | 1.852967360720451e-01 |
| 3 | 1.207609924037345e-02 | 9.394713171801555e-01 | 3.026434140992224e-02 | 3.026434140992224e-02 |
| 3 | -3.340e-07-i*7.826e-09 | -3.948e-01+i*3.234e-01 | 6.974e-01-i*1.617e-01 | 6.974e-01-i*1.617e-01 |
| 3 | -3.340e-07+i*7.826e-09 | -3.948e-01-i*3.234e-01 | 6.974e-01+i*1.617e-01 | 6.974e-01+i*1.617e-01 |
| 6 | 4.628872752836702e-02 | 4.029515246241994e-02 | 3.624632940721336e-01 | 5.972415534654465e-01 |
| 6 | 3.242359184500047e-02 | 3.751845230246799e-02 | 1.576081280871773e-01 | 8.048734196103547e-01 |
| 6 | 3.530493603950046e-06 | -2.680320365606058e-01 | 2.537738020571674e-01 | 1.014258234503438e+00 |

$d = 12$, $n_p = 33$, type $[0, 5, 3]$, quality CC

| | | | | |
|---|---|---|---|---|
| 3 | 1.554e-02-i*4.250e-03 | 3.498e-01-i*1.104e-01 | 3.251e-01+i*5.519e-02 | 3.251e-01+i*5.519e-02 |
| 3 | 7.930e-02+i*6.526e-03 | 1.458e-01+i*7.501e-03 | 4.271e-01-i*3.751e-03 | 4.271e-01-i*3.751e-03 |
| 3 | 8.076e-02-i*2.961e-03 | 6.020e-01+i*5.199e-03 | 1.990e-01-i*2.600e-03 | 1.990e-01-i*2.600e-03 |
| 3 | 5.929e-02+i*1.057e-03 | 2.958e-02+i*7.158e-04 | 4.852e-01-i*3.579e-04 | 4.852e-01-i*3.579e-04 |
| 3 | 1.739e-02+i*3.862e-05 | 9.269e-01-i*7.533e-05 | 3.654e-02+i*3.767e-05 | 3.654e-02+i*3.767e-05 |
| 6 | -3.035e-03+i*1.464e-04 | 3.397e-02+i*4.363e-04 | 4.800e-01+i*1.982e-01 | 4.860e-01-i*1.986e-01 |
| 6 | 4.355e-02-i*3.506e-04 | 4.142e-02-i*4.566e-04 | 1.889e-01+i*2.512e-04 | 7.697e-01+i*2.054e-04 |
| 6 | 3.620e-06-i*1.115e-06 | -2.783e-01-i*1.595e-02 | 2.086e-01+i*2.644e-03 | 1.070e+00+i*1.330e-02 |

$d = 12$, $n_p = 33$, type $[0, 5, 3]$, quality CC

| | | | | |
|---|---|---|---|---|
| 3 | 1.554e-02+i*4.250e-03 | 3.498e-01+i*1.104e-01 | 3.251e-01-i*5.519e-02 | 3.251e-01-i*5.519e-02 |
| 3 | 7.930e-02-i*6.526e-03 | 1.458e-01-i*7.501e-03 | 4.271e-01+i*3.751e-03 | 4.271e-01+i*3.751e-03 |
| 3 | 8.076e-02+i*2.961e-03 | 6.020e-01-i*5.199e-03 | 1.990e-01+i*2.600e-03 | 1.990e-01+i*2.600e-03 |
| 3 | 5.929e-02-i*1.057e-03 | 2.958e-02-i*7.158e-04 | 4.852e-01+i*3.579e-04 | 4.852e-01+i*3.579e-04 |
| 3 | 1.739e-02-i*3.862e-05 | 9.269e-01+i*7.533e-05 | 3.654e-02-i*3.767e-05 | 3.654e-02-i*3.767e-05 |
| 6 | -3.035e-03-i*1.464e-04 | 3.397e-02-i*4.363e-04 | 4.800e-01-i*1.982e-01 | 4.860e-01+i*1.986e-01 |
| 6 | 4.355e-02+i*3.506e-04 | 4.142e-02+i*4.566e-04 | 1.889e-01-i*2.512e-04 | 7.697e-01-i*2.054e-04 |
| 6 | 3.620e-06+i*1.115e-06 | -2.783e-01+i*1.595e-02 | 2.086e-01-i*2.644e-03 | 1.070e+00-i*1.330e-02 |

$d = 12$, $n_p = 33$, type $[0, 5, 3]$, quality CC

| | | | | |
|---|---|---|---|---|
| 3 | 1.035122307108925e-01 | 4.675255177056619e-01 | 2.662372411471691e-01 | 2.662372411471691e-01 |
| 3 | 5.340463725129441e-02 | 6.791152890335521e-01 | 1.604423554832239e-01 | 1.604423554832239e-01 |
| 3 | 1.307543778679365e-02 | 9.364592625478135e-01 | 3.177036872609324e-02 | 3.177036872609324e-02 |
| 3 | 2.840e-03+i*4.405e-03 | 1.322e-01+i*1.537e-01 | 4.339e-01-i*7.683e-02 | 4.339e-01-i*7.683e-02 |
| 3 | 2.840e-03-i*4.405e-03 | 1.322e-01-i*1.537e-01 | 4.339e-01+i*7.683e-02 | 4.339e-01+i*7.683e-02 |
| 6 | 4.993461721778829e-02 | 4.178080351092829e-02 | 3.665448020266667e-01 | 5.916743944624050e-01 |
| 6 | 2.889531381784557e-02 | 3.311954761651255e-02 | 1.611089240667322e-01 | 8.057715283167553e-01 |
| 6 | 3.618475831792652e-07 | -3.999113745325838e-01 | 2.958658352262632e-01 | 1.104045539306321e+00 |

$d = 12$, $n_p = 33$, type $[0, 5, 3]$, quality CC

| | | | | |
|---|---|---|---|---|
| 3 | 1.112308226181848e-01 | 4.803234038839840e-01 | 2.598382980580080e-01 | 2.598382980580080e-01 |
| 3 | 5.110141409971637e-02 | 7.103816346042944e-01 | 1.448091826978528e-01 | 1.448091826978528e-01 |
| 3 | 1.388505628942695e-02 | 9.342995943411704e-01 | 3.285020282941480e-02 | 3.285020282941480e-02 |
| 3 | 1.092e-03+i*2.179e-03 | 1.219e-01+i*1.923e-01 | 4.390e-01-i*9.614e-02 | 4.390e-01-i*9.614e-02 |
| 3 | 1.092e-03-i*2.179e-03 | 1.219e-01-i*1.923e-01 | 4.390e-01+i*9.614e-02 | 4.390e-01+i*9.614e-02 |
| 6 | 5.269619270758365e-02 | 4.470737534861031e-02 | 3.657322814715470e-01 | 5.895603431798427e-01 |
| 6 | 2.477004805347968e-02 | 2.752919704254155e-02 | 1.651343238096192e-01 | 8.073364791478393e-01 |
| 6 | 1.987951052298557e-09 | -8.428882381238022e-01 | 4.490357226826952e-01 | 1.393852515441107e+00 |

$d = 12$, $n_p = 33$, type $[0, 5, 3]$, quality CC

| | | | | |
|---|---|---|---|---|
| 3 | 1.150e-02+i*6.854e-03 | 3.617e-01+i*1.368e-01 | 3.191e-01-i*6.842e-02 | 3.191e-01-i*6.842e-02 |
| 3 | 8.444e-02-i*1.107e-02 | 1.519e-01-i*1.165e-02 | 4.241e-01+i*5.827e-03 | 4.241e-01+i*5.827e-03 |
| 3 | 8.315e-02+i*5.616e-03 | 6.114e-01-i*8.144e-03 | 1.943e-01+i*4.072e-03 | 1.943e-01+i*4.072e-03 |
| 3 | 3.661e-02-i*2.826e-03 | 2.717e-02-i*1.754e-03 | 4.864e-01+i*8.769e-04 | 4.864e-01+i*8.769e-04 |
| 3 | 3.223e-02+i*2.143e-03 | 8.952e-01-i*6.397e-03 | 5.241e-02+i*3.198e-03 | 5.241e-02+i*3.198e-03 |
| 6 | 4.269e-02-i*4.564e-04 | 3.708e-02-i*1.089e-04 | 2.355e-01+i*3.493e-03 | 7.274e-01-i*3.384e-03 |
| 6 | 1.317e-05+i*9.663e-05 | -1.229e-01+i*5.915e-02 | 5.302e-02+i*6.414e-05 | 1.070e+00-i*5.921e-02 |
| 6 | 6.921e-10-i*9.501e-10 | 7.994e-02-i*1.238e+00 | 2.917e-01-i*1.048e-02 | 6.284e-01+i*1.248e+00 |

$d = 12$, $n_p = 33$, type $[0, 5, 3]$, quality CC

| | | | | |
|---|---|---|---|---|
| 3 | 1.150e-02-i*6.854e-03 | 3.617e-01-i*1.368e-01 | 3.191e-01+i*6.842e-02 | 3.191e-01+i*6.842e-02 |
| 3 | 8.444e-02+i*1.107e-02 | 1.519e-01+i*1.165e-02 | 4.241e-01-i*5.827e-03 | 4.241e-01-i*5.827e-03 |
| 3 | 8.315e-02-i*5.616e-03 | 6.114e-01+i*8.144e-03 | 1.943e-01-i*4.072e-03 | 1.943e-01-i*4.072e-03 |
| 3 | 3.661e-02+i*2.826e-03 | 2.717e-02+i*1.754e-03 | 4.864e-01-i*8.769e-04 | 4.864e-01-i*8.769e-04 |
| 3 | 3.223e-02-i*2.143e-03 | 8.952e-01+i*6.397e-03 | 5.241e-02-i*3.198e-03 | 5.241e-02-i*3.198e-03 |
| 6 | 4.269e-02+i*4.564e-04 | 3.708e-02+i*1.089e-04 | 2.355e-01-i*3.493e-03 | 7.274e-01+i*3.384e-03 |
| 6 | 1.317e-05-i*9.663e-05 | -1.229e-01-i*5.915e-02 | 5.302e-02-i*6.414e-05 | 1.070e+00+i*5.921e-02 |
| 6 | 6.921e-10+i*9.501e-10 | 7.994e-02+i*1.238e+00 | 2.917e-01+i*1.048e-02 | 6.284e-01-i*1.248e+00 |

$d = 13$, $n_p = 36$, type $[0, 6, 3]$, quality NO

| | | | | |
|---|---|---|---|---|
| 3 | 6.318978359878283e-02 | 4.579994089510506e-01 | 2.710002955244747e-01 | 2.710002955244747e-01 |
| 3 | 5.068506106702577e-02 | 1.193522510438773e-01 | 4.403238744780613e-01 | 4.403238744780613e-01 |
| 3 | 2.387508405516934e-02 | 2.342429853318937e-02 | 4.882878507334053e-01 | 4.882878507334053e-01 |
| 3 | 2.785609711355220e-02 | 7.857592937637046e-01 | 1.071203531181477e-01 | 1.071203531181477e-01 |
| 3 | 8.045069816524590e-03 | 9.504231379326773e-01 | 2.478843103366136e-02 | 2.478843103366136e-02 |
| 3 | -4.438917939249711e-15 | 3.194642494212562e+00 | -1.097321247106281e+00 | -1.097321247106281e+00 |
| 6 | 4.339833070288237e-02 | 1.154580228219941e-01 | 2.531770462425584e-01 | 6.313649309354475e-01 |
| 6 | 2.157569981627577e-02 | 2.291948280481281e-02 | 2.933219413072190e-01 | 6.837585758879682e-01 |
| 6 | 1.486708832198338e-02 | 2.082152084663162e-02 | 1.287194165090116e-01 | 8.504590626443567e-01 |

$d = 13$, $n_p = 36$, type $[0, 6, 3]$, quality NC

| | | | | |
|---|---|---|---|---|
| 3 | 6.759912191384208e-02 | 4.573970726816931e-01 | 2.713014636591534e-01 | 2.713014636591534e-01 |
| 3 | 6.482227922602433e-02 | 9.264399651044037e-02 | 4.536780017447798e-01 | 4.536780017447798e-01 |
| 3 | 5.652698505583247e-02 | 6.300254948226160e-01 | 1.849872525886920e-01 | 1.849872525886920e-01 |
| 3 | 2.996537590633597e-02 | 8.003077142922704e-01 | 9.984614285386479e-02 | 9.984614285386479e-02 |
| 3 | 8.981956274710440e-03 | 9.475416844977801e-01 | 2.622915775110997e-02 | 2.622915775110997e-02 |
| 3 | 6.985977604023551e-03 | -1.104854640054012e-02 | 5.055242732002701e-01 | 5.055242732002701e-01 |
| 6 | 3.658503474861574e-02 | 3.932850687079561e-02 | 2.942856814611542e-01 | 6.663858116680501e-01 |
| 6 | 1.271584481388969e-02 | 1.497643465530995e-02 | 1.391073256947718e-01 | 8.459162396499182e-01 |
| 6 | -7.506088622319255e-05 | 1.848e-01-i*2.550e-01 | 1.848e-01+i*2.550e-01 | 6.304930708132193e-01 |

$d = 13$, $n_p = 36$, type $[0, 6, 3]$, quality CC

| | | | | |
|---|---|---|---|---|
| 3 | 7.948e-02-i*6.481e-05 | 1.981e-01-i*4.789e-04 | 4.010e-01+i*2.394e-04 | 4.010e-01+i*2.394e-04 |
| 3 | 5.981e-02+i*9.515e-03 | 5.878e-01-i*2.190e-03 | 2.061e-01+i*1.095e-03 | 2.061e-01+i*1.095e-03 |
| 3 | 3.776e-02-i*2.289e-03 | 3.535e-02-i*3.723e-03 | 4.823e-01+i*1.861e-03 | 4.823e-01+i*1.861e-03 |
| 3 | -1.195e-04+i*2.177e-04 | 9.267e-02+i*2.222e-01 | 4.537e-01-i*1.111e-01 | 4.537e-01-i*1.111e-01 |
| 3 | 3.159e-02-i*7.860e-04 | 7.850e-01-i*1.652e-02 | 1.075e-01+i*8.261e-03 | 1.075e-01+i*8.261e-03 |
| 3 | 8.756e-03-i*9.485e-04 | 9.477e-01+i*2.724e-03 | 2.614e-02-i*1.362e-03 | 2.614e-02-i*1.362e-03 |
| 6 | 2.213e-02+i*5.824e-02 | 4.631e-02-i*3.944e-02 | 3.040e-01+i*1.194e-02 | 6.496e-01+i*2.750e-02 |
| 6 | 2.188e-02-i*6.315e-02 | 3.218e-02-i*2.743e-02 | 3.021e-01+i*9.911e-04 | 6.657e-01+i*2.644e-02 |
| 6 | 1.402e-02+i*2.083e-03 | 1.968e-02+i*5.244e-03 | 1.303e-01-i*9.008e-03 | 8.500e-01+i*3.764e-03 |

$d = 13$, $n_p = 36$, type $[0, 6, 3]$, quality CC

| | | | | |
|---|---|---|---|---|
| 3 | 7.948e-02+i*6.481e-05 | 1.981e-01+i*4.789e-04 | 4.010e-01-i*2.394e-04 | 4.010e-01-i*2.394e-04 |
| 3 | 5.981e-02-i*9.515e-03 | 5.878e-01+i*2.190e-03 | 2.061e-01-i*1.095e-03 | 2.061e-01-i*1.095e-03 |
| 3 | 3.776e-02+i*2.289e-03 | 3.535e-02+i*3.723e-03 | 4.823e-01-i*1.861e-03 | 4.823e-01-i*1.861e-03 |
| 3 | -1.195e-04-i*2.177e-04 | 9.267e-02-i*2.222e-01 | 4.537e-01+i*1.111e-01 | 4.537e-01+i*1.111e-01 |
| 3 | 3.159e-02+i*7.860e-04 | 7.850e-01+i*1.652e-02 | 1.075e-01-i*8.261e-03 | 1.075e-01-i*8.261e-03 |
| 3 | 8.756e-03+i*9.485e-04 | 9.477e-01-i*2.724e-03 | 2.614e-02+i*1.362e-03 | 2.614e-02+i*1.362e-03 |
| 6 | 2.213e-02-i*5.824e-02 | 4.631e-02+i*3.944e-02 | 3.040e-01-i*1.194e-02 | 6.496e-01-i*2.750e-02 |
| 6 | 2.188e-02+i*6.315e-02 | 3.218e-02+i*2.743e-02 | 3.021e-01-i*9.911e-04 | 6.657e-01-i*2.644e-02 |
| 6 | 1.402e-02-i*2.083e-03 | 1.968e-02-i*5.244e-03 | 1.303e-01+i*9.008e-03 | 8.500e-01-i*3.764e-03 |

$d = 13$, $n_p = 36$, type $[0, 6, 3]$, quality CC

| | | | | |
|---|---|---|---|---|
| 3 | 5.185e-02-i*3.447e-03 | 2.268e-01+i*6.166e-03 | 3.866e-01-i*3.083e-03 | 3.866e-01-i*3.083e-03 |
| 3 | 4.532e-02+i*7.699e-03 | 5.543e-01+i*1.225e-02 | 2.228e-01-i*6.124e-03 | 2.228e-01-i*6.124e-03 |
| 3 | 3.853e-02-i*6.338e-04 | 9.669e-02+i*1.529e-02 | 4.517e-01-i*7.647e-03 | 4.517e-01-i*7.647e-03 |
| 3 | 2.080e-02+i*4.792e-03 | 2.057e-02+i*4.463e-03 | 4.897e-01-i*2.232e-03 | 4.897e-01-i*2.232e-03 |
| 3 | 3.114e-02+i*1.033e-03 | 7.736e-01-i*7.427e-03 | 1.132e-01+i*3.713e-03 | 1.132e-01+i*3.713e-03 |
| 3 | 8.113e-03-i*2.459e-04 | 9.499e-01+i*7.637e-04 | 2.505e-02-i*3.819e-04 | 2.505e-02-i*3.819e-04 |
| 6 | 3.515e-02-i*1.574e-03 | 9.605e-02-i*1.454e-02 | 2.686e-01+i*1.037e-02 | 6.354e-01+i*4.166e-03 |
| 6 | 1.838e-02-i*3.609e-03 | 1.958e-02-i*4.256e-03 | 2.926e-01-i*1.510e-03 | 6.878e-01+i*5.766e-03 |
| 6 | 1.527e-02+i*5.841e-04 | 2.175e-02+i*1.243e-03 | 1.271e-01-i*2.072e-03 | 8.511e-01+i*8.291e-04 |

$d = 13$, $n_p = 36$, type $[0, 6, 3]$, quality CC

| | | | | |
|---|---|---|---|---|
| 3 | 5.185e-02+i*3.447e-03 | 2.268e-01-i*6.166e-03 | 3.866e-01+i*3.083e-03 | 3.866e-01+i*3.083e-03 |
| 3 | 4.532e-02-i*7.699e-03 | 5.543e-01-i*1.225e-02 | 2.228e-01+i*6.124e-03 | 2.228e-01+i*6.124e-03 |
| 3 | 3.853e-02+i*6.338e-04 | 9.669e-02-i*1.529e-02 | 4.517e-01+i*7.647e-03 | 4.517e-01+i*7.647e-03 |
| 3 | 2.080e-02-i*4.792e-03 | 2.057e-02-i*4.463e-03 | 4.897e-01+i*2.232e-03 | 4.897e-01+i*2.232e-03 |
| 3 | 3.114e-02-i*1.033e-03 | 7.736e-01+i*7.427e-03 | 1.132e-01-i*3.713e-03 | 1.132e-01-i*3.713e-03 |
| 3 | 8.113e-03+i*2.459e-04 | 9.499e-01-i*7.637e-04 | 2.505e-02+i*3.819e-04 | 2.505e-02+i*3.819e-04 |
| 6 | 3.515e-02+i*1.574e-03 | 9.605e-02+i*1.454e-02 | 2.686e-01-i*1.037e-02 | 6.354e-01-i*4.166e-03 |
| 6 | 1.838e-02+i*3.609e-03 | 1.958e-02+i*4.256e-03 | 2.926e-01+i*1.510e-03 | 6.878e-01-i*5.766e-03 |
| 6 | 1.527e-02-i*5.841e-04 | 2.175e-02-i*1.243e-03 | 1.271e-01+i*2.072e-03 | 8.511e-01-i*8.291e-04 |

$d = 13$, $n_p = 36$, type $[0, 6, 3]$, quality CC

| | | | | |
|---|---|---|---|---|
| 3 | 3.960e-02+i*3.446e-02 | 4.514e-01+i*4.524e-02 | 2.743e-01-i*2.262e-02 | 2.743e-01-i*2.262e-02 |
| 3 | 5.218e-02-i*3.447e-03 | 1.355e-01-i*8.621e-03 | 4.322e-01+i*4.311e-03 | 4.322e-01+i*4.311e-03 |
| 3 | 4.554e-02-i*3.024e-02 | 5.558e-01+i*4.309e-02 | 2.221e-01-i*2.155e-02 | 2.221e-01-i*2.155e-02 |
| 3 | 2.723e-02-i*7.514e-04 | 2.551e-02+i*2.107e-05 | 4.872e-01-i*1.053e-05 | 4.872e-01-i*1.053e-05 |
| 3 | 3.148e-02-i*3.117e-03 | 7.639e-01+i*2.116e-02 | 1.180e-01-i*1.058e-02 | 1.180e-01-i*1.058e-02 |
| 3 | 7.721e-03+i*7.344e-04 | 9.510e-01-i*2.485e-03 | 2.449e-02+i*1.242e-03 | 2.449e-02+i*1.242e-03 |
| 6 | 3.677e-02-i*2.245e-03 | 7.609e-02+i*1.261e-02 | 2.815e-01-i*7.207e-03 | 6.425e-01-i*5.400e-03 |
| 6 | 1.180e-02+i*4.988e-03 | 1.159e-02+i*8.183e-03 | 2.898e-01+i*5.243e-03 | 6.986e-01-i*1.343e-02 |
| 6 | 1.622e-02-i*1.564e-03 | 2.390e-02-i*2.874e-03 | 1.235e-01+i*4.636e-03 | 8.526e-01-i*1.762e-03 |

$d = 13$, $n_p = 36$, type $[0, 6, 3]$, quality CC

| | | | | |
|---|---|---|---|---|
| 3 | 3.960e-02-i*3.446e-02 | 4.514e-01-i*4.524e-02 | 2.743e-01+i*2.262e-02 | 2.743e-01+i*2.262e-02 |
| 3 | 5.218e-02+i*3.447e-03 | 1.355e-01+i*8.621e-03 | 4.322e-01-i*4.311e-03 | 4.322e-01-i*4.311e-03 |
| 3 | 4.554e-02+i*3.024e-02 | 5.558e-01-i*4.309e-02 | 2.221e-01+i*2.155e-02 | 2.221e-01+i*2.155e-02 |
| 3 | 2.723e-02+i*7.514e-04 | 2.551e-02-i*2.107e-05 | 4.872e-01+i*1.053e-05 | 4.872e-01+i*1.053e-05 |
| 3 | 3.148e-02+i*3.117e-03 | 7.639e-01-i*2.116e-02 | 1.180e-01+i*1.058e-02 | 1.180e-01+i*1.058e-02 |
| 3 | 7.721e-03-i*7.344e-04 | 9.510e-01+i*2.485e-03 | 2.449e-02-i*1.242e-03 | 2.449e-02-i*1.242e-03 |
| 6 | 3.677e-02+i*2.245e-03 | 7.609e-02-i*1.261e-02 | 2.815e-01+i*7.207e-03 | 6.425e-01+i*5.400e-03 |
| 6 | 1.180e-02-i*4.988e-03 | 1.159e-02-i*8.183e-03 | 2.898e-01-i*5.243e-03 | 6.986e-01+i*1.343e-02 |
| 6 | 1.622e-02+i*1.564e-03 | 2.390e-02+i*2.874e-03 | 1.235e-01-i*4.636e-03 | 8.526e-01+i*1.762e-03 |

$d = 13$, $n_p = 37$, type $[1,4,4]$, quality PI

| | | | | |
|---|---|---|---|---|
| 1 | 6.666531183964321e-02 | 3.333333333333333e-01 | 3.333333333333333e-01 | 3.333333333333333e-01 |
| 3 | 5.637138317907531e-02 | 1.416807749137785e-01 | 4.291596125431107e-01 | 4.291596125431107e-01 |
| 3 | 5.703687953133591e-02 | 5.483198542641960e-01 | 2.258400728679020e-01 | 2.258400728679020e-01 |
| 3 | 2.704770288106011e-02 | 2.514270940526753e-02 | 4.874286452973662e-01 | 4.874286452973662e-01 |
| 3 | 3.254577710106209e-02 | 7.510843558720015e-01 | 1.244578220639993e-01 | 1.244578220639993e-01 |
| 6 | 3.846210380706763e-02 | 7.127447151191104e-02 | 2.845207640198182e-01 | 6.442047644682707e-01 |
| 6 | 9.138438814371032e-03 | 4.935323489543055e-03 | 2.862147535443420e-01 | 7.088499229661149e-01 |
| 6 | 1.751340205091933e-02 | 2.673280979433629e-02 | 1.245254158513282e-01 | 8.487417743543355e-01 |
| 6 | 3.940965341434761e-03 | 1.635078050759145e-02 | 3.285424868085981e-02 | 9.507949708115487e-01 |

$d = 13$, $n_p = 37$, type $[1,4,4]$, quality PI

| | | | | |
|---|---|---|---|---|
| 1 | 6.796003658683164e-02 | 3.333333333333333e-01 | 3.333333333333333e-01 | 3.333333333333333e-01 |
| 3 | 5.560196753045333e-02 | 1.461171714803992e-01 | 4.269414142598004e-01 | 4.269414142598004e-01 |
| 3 | 5.827848511919998e-02 | 5.572554274163342e-01 | 2.213722862918329e-01 | 2.213722862918329e-01 |
| 3 | 2.399440192889473e-02 | 2.184610709492130e-02 | 4.890769464525393e-01 | 4.890769464525393e-01 |
| 3 | 6.052337103539172e-03 | 9.569806377823136e-01 | 2.150968110884318e-02 | 2.150968110884318e-02 |
| 6 | 3.464127614084837e-02 | 6.801224355420665e-02 | 3.084417608921178e-01 | 6.235459955536756e-01 |
| 6 | 2.417903981159382e-02 | 8.789548303219732e-02 | 1.635974010678505e-01 | 7.485071158999522e-01 |
| 6 | 9.590681003543263e-03 | 5.126389102382369e-03 | 2.725158177734297e-01 | 7.223577931241880e-01 |
| 6 | 1.496540110516567e-02 | 2.437018690109383e-02 | 1.109220428034634e-01 | 8.647077702954428e-01 |

$d = 13$, $n_p = 37$, type $[1,4,4]$, quality NI

| | | | | |
|---|---|---|---|---|
| 1 | -1.056360738456401e-01 | 3.333333333333333e-01 | 3.333333333333333e-01 | 3.333333333333333e-01 |
| 3 | 9.690034727804083e-02 | 4.242813469723264e-01 | 2.878593265138368e-01 | 2.878593265138368e-01 |
| 3 | 5.018216635227328e-02 | 1.131979829755801e-01 | 4.434010085122100e-01 | 4.434010085122100e-01 |
| 3 | 2.102855973694512e-02 | 2.147839246570478e-02 | 4.892608037671476e-01 | 4.892608037671476e-01 |
| 3 | 2.672599067349385e-02 | 8.000919735991067e-01 | 9.995401320044664e-02 | 9.995401320044664e-02 |
| 6 | 4.607891261373841e-02 | 1.192644209390402e-01 | 2.495054689443353e-01 | 6.312301101166245e-01 |
| 6 | 2.135290362787687e-02 | 2.361515966854858e-02 | 3.017346932372817e-01 | 6.746501470941697e-01 |
| 6 | 1.450394248637925e-02 | 2.089774464177895e-02 | 1.430257663819780e-01 | 8.360764889762430e-01 |
| 6 | 4.918388225902278e-03 | 1.497391087216802e-02 | 3.985330690077000e-02 | 9.451727822270620e-01 |

$d = 13$, $n_p = 37$, type $[1,4,4]$, quality NI

| | | | | |
|---|---|---|---|---|
| 1 | -9.794282830779282e-01 | 3.333333333333333e-01 | 3.333333333333333e-01 | 3.333333333333333e-01 |
| 3 | 3.851843248196896e-01 | 3.731714975085028e-01 | 3.134142512457486e-01 | 3.134142512457486e-01 |
| 3 | 4.707074375139372e-02 | 1.036731386947847e-01 | 4.481634306526077e-01 | 4.481634306526077e-01 |
| 3 | 1.947159860023236e-02 | 1.876094369614878e-02 | 4.906195281519256e-01 | 4.906195281519256e-01 |
| 3 | 8.598559295098043e-03 | 9.482924272447965e-01 | 2.585378637760174e-02 | 2.585378637760174e-02 |
| 6 | 4.686871755715881e-02 | 1.280748545621051e-01 | 2.559060504714026e-01 | 6.160190949664922e-01 |
| 6 | 2.321458227198339e-02 | 2.466575888342652e-02 | 2.937275637422268e-01 | 6.816066773743466e-01 |
| 6 | 1.865886541493881e-02 | 7.660504708654196e-02 | 1.303752945362578e-01 | 7.930196583772002e-01 |
| 6 | 1.099993536903349e-02 | 1.517155770635715e-02 | 1.295372633260821e-01 | 8.552911789675607e-01 |

$d = 13$, $n_p = 37$, type $[1,4,4]$, quality NI

| | | | | |
|---|---|---|---|---|
| 1 | -6.961938918173517e-01 | 3.333333333333333e-01 | 3.333333333333333e-01 | 3.333333333333333e-01 |
| 3 | 2.916465048495467e-01 | 3.802409844193277e-01 | 3.098795077903361e-01 | 3.098795077903361e-01 |
| 3 | 4.702284598963952e-02 | 1.047710914472636e-01 | 4.476144542763682e-01 | 4.476144542763682e-01 |
| 3 | 2.943707721076129e-02 | 7.979373791902761e-01 | 1.010313104048620e-01 | 1.010313104048620e-01 |
| 3 | 7.060478452030929e-03 | 9.526826973365726e-01 | 2.365865133171368e-02 | 2.365865133171368e-02 |
| 6 | 4.748213927210297e-02 | 1.255412745019193e-01 | 2.552672945625177e-01 | 6.191914309355630e-01 |
| 6 | 1.837479881995625e-02 | 2.035044354178874e-02 | 3.990878803018775e-01 | 5.805616761563338e-01 |
| 6 | 1.907290693660829e-02 | 2.679648266402744e-02 | 2.407898961433650e-01 | 7.324136211926076e-01 |
| 6 | 1.018568368990188e-02 | 1.643529593541106e-02 | 1.139836801912405e-01 | 8.695810238733484e-01 |

$d = 13$, $n_p = 37$, type $[1,4,4]$, quality PO

| | | | | |
|---|---|---|---|---|
| 1 | 6.657635373140225e-02 | 3.333333333333333e-01 | 3.333333333333333e-01 | 3.333333333333333e-01 |
| 3 | 3.781760342355384e-02 | 4.065083803063968e-02 | 4.796745809846802e-01 | 4.796745809846802e-01 |
| 3 | 3.727970689588019e-02 | 6.799099857155733e-01 | 1.600450071422134e-01 | 1.600450071422134e-01 |
| 3 | 2.162170839832446e-02 | 8.164270302175394e-01 | 9.178648489123030e-02 | 9.178648489123030e-02 |
| 3 | 7.834565977584906e-03 | 9.511357024397497e-01 | 2.443214878012517e-02 | 2.443214878012517e-02 |
| 6 | 5.561753196072258e-02 | 1.631186598891134e-01 | 3.234656038369160e-01 | 5.134157362739705e-01 |
| 6 | 3.364468429923003e-02 | 4.272125954432780e-02 | 2.753651363931316e-01 | 6.819136040625406e-01 |
| 6 | 1.249955798858142e-02 | 1.639809613318692e-02 | 1.310604460192536e-01 | 8.525414578475595e-01 |
| 6 | 1.532041115227232e-03 | -2.858841454522855e-02 | 3.723512893200343e-01 | 6.562371252251942e-01 |

$d = 13$, $n_p = 37$, type $[1, 4, 4]$, quality PO

| | | | | |
|---|---|---|---|---|
| 1 | 7.451979772889958e-02 | 3.333333333333333e-01 | 3.333333333333333e-01 | 3.333333333333333e-01 |
| 3 | 3.542731490741545e-02 | 3.972412896990688e-02 | 4.801379355150466e-01 | 4.801379355150466e-01 |
| 3 | 4.517738077189447e-02 | 7.182901883279177e-01 | 1.408549058360412e-01 | 1.408549058360412e-01 |
| 3 | 6.162545963317280e-03 | 9.573846620847588e-01 | 2.130766895762062e-02 | 2.130766895762062e-02 |
| 3 | 1.323218846515062e-03 | -2.601973034214071e-02 | 5.130098651710704e-01 | 5.130098651710704e-01 |
| 6 | 6.125618747949810e-02 | 1.559162590783967e-01 | 3.179678761553044e-01 | 5.261158647662990e-01 |
| 6 | 3.041341546050036e-02 | 3.217025916078637e-02 | 2.807446145522045e-01 | 6.870851262870091e-01 |
| 6 | 1.852676980014065e-02 | 2.739010027672666e-02 | 1.165439820433089e-01 | 8.560659176799644e-01 |
| 6 | 5.097393806491604e-06 | -1.866257643790296e-01 | 3.024088556633660e-01 | 8.842169087156636e-01 |

$d = 13$, $n_p = 37$, type $[1, 4, 4]$, quality PO

| | | | | |
|---|---|---|---|---|
| 1 | 7.300062457734237e-02 | 3.333333333333333e-01 | 3.333333333333333e-01 | 3.333333333333333e-01 |
| 3 | 2.754670756416041e-02 | 5.216902384317640e-01 | 2.391548807841180e-01 | 2.391548807841180e-01 |
| 3 | 2.900643831823423e-02 | 2.633671825444963e-02 | 4.868316408727752e-01 | 4.868316408727752e-01 |
| 3 | 4.597983286514976e-02 | 7.180106966241533e-01 | 1.409946516879233e-01 | 1.409946516879233e-01 |
| 3 | 5.865133413824131e-03 | 9.586309099161649e-01 | 2.068454504191755e-02 | 2.068454504191755e-02 |
| 6 | 5.250904751674010e-02 | 1.361671314686231e-01 | 3.375913179304945e-01 | 5.262415506008824e-01 |
| 6 | 2.952438833939019e-02 | 3.130525499340692e-02 | 2.778286750949170e-01 | 6.908660699116761e-01 |
| 6 | 1.826471389539543e-02 | 2.716694939047455e-02 | 1.147053694470084e-01 | 8.581276811625171e-01 |
| 6 | 2.690071566281446e-06 | -2.191472603091626e-01 | 3.367710364820478e-01 | 8.823762238271148e-01 |

$d = 13$, $n_p = 37$, type $[1, 4, 4]$, quality PO

| | | | | |
|---|---|---|---|---|
| 1 | 6.157175300444431e-02 | 3.333333333333333e-01 | 3.333333333333333e-01 | 3.333333333333333e-01 |
| 3 | 5.964392785259157e-02 | 1.665866173488305e-01 | 4.167066913255847e-01 | 4.167066913255847e-01 |
| 3 | 6.445237215677630e-02 | 5.929249213048502e-01 | 2.035375393475749e-01 | 2.035375393475749e-01 |
| 3 | 1.342215175667655e-02 | 1.008800009761598e-02 | 4.949559999511920e-01 | 4.949559999511920e-01 |
| 3 | 5.245617399745472e-07 | 1.271565998766019e+00 | -1.357829993830094e-01 | -1.357829993830094e-01 |
| 6 | 4.161497351249294e-02 | 5.849890860214470e-02 | 3.402219418488622e-01 | 6.012791495489931e-01 |
| 6 | 3.304118721007654e-02 | 5.672027207146819e-02 | 1.581945847384451e-01 | 7.850851431900867e-01 |
| 6 | 8.130591706453491e-03 | 1.267448669978824e-02 | 5.857464525645708e-02 | 9.287508680437547e-01 |
| 6 | 4.858467239677446e-03 | -1.018678736414063e-02 | 2.536495436450076e-01 | 7.565372437191330e-01 |

$d = 13$, $n_p = 37$, type $[1, 4, 4]$, quality NO

| | | | | |
|---|---|---|---|---|
| 1 | -8.825075577480786e-01 | 3.333333333333333e-01 | 3.333333333333333e-01 | 3.333333333333333e-01 |
| 3 | 3.714998848303912e-01 | 2.807076426850682e-01 | 3.596461786574659e-01 | 3.596461786574659e-01 |
| 3 | 6.546863782953757e-02 | 6.410873577715350e-01 | 1.794563211142325e-01 | 1.794563211142325e-01 |
| 3 | 2.515149380737124e-02 | 8.467360995450211e-01 | 7.663195022748946e-02 | 7.663195022748946e-02 |
| 3 | -1.191020242242123e-03 | -1.512607380197372e-01 | 5.756303690098686e-01 | 5.756303690098686e-01 |
| 6 | 5.297774618092841e-02 | 5.803862527152615e-02 | 3.693288083004901e-01 | 5.726325664279838e-01 |
| 6 | 2.440917570339561e-02 | 2.757907080505288e-02 | 2.011676081306144e-01 | 7.712533210643327e-01 |
| 6 | 4.914920377831646e-03 | 2.575083462406479e-03 | 5.286237388283830e-02 | 9.445625426547552e-01 |
| 6 | 9.849192499951766e-04 | -1.345310819743311e-01 | 5.309667818341154e-01 | 6.035643001402157e-01 |

$d = 13$, $n_p = 37$, type $[1, 4, 4]$, quality NO

| | | | | |
|---|---|---|---|---|
| 1 | -4.067297235220971e-02 | 3.333333333333333e-01 | 3.333333333333333e-01 | 3.333333333333333e-01 |
| 3 | 7.679595838627680e-02 | 4.423584089816469e-01 | 2.788207955091765e-01 | 2.788207955091765e-01 |
| 3 | 4.913203301248851e-02 | 1.160547741188262e-01 | 4.419726129405869e-01 | 4.419726129405869e-01 |
| 3 | 2.519694548602949e-02 | 7.568504061877176e-01 | 1.215747969061412e-01 | 1.215747969061412e-01 |
| 3 | 1.851341229555045e-02 | 9.023316585782802e-01 | 4.883417071085991e-02 | 4.883417071085991e-02 |
| 6 | 4.268573007490437e-02 | 1.158860310190741e-01 | 2.571809830742116e-01 | 6.269329859067143e-01 |
| 6 | 2.447246972059732e-02 | 2.263785786186450e-02 | 3.809449323408714e-01 | 5.964172097972641e-01 |
| 6 | 2.019135324548976e-02 | 2.299411479142018e-02 | 1.854712230079724e-01 | 7.915346622006074e-01 |
| 6 | 1.276767760870889e-03 | -1.811422647488586e-02 | 4.511466590857513e-02 | 9.729995605663107e-01 |

$d = 13$, $n_p = 37$, type $[1, 4, 4]$, quality NO

| | | | | |
|---|---|---|---|---|
| 1 | 8.068166732459353e-02 | 3.333333333333333e-01 | 3.333333333333333e-01 | 3.333333333333333e-01 |
| 3 | 3.337341843097953e-02 | 3.038125065488849e-02 | 4.848093746725558e-01 | 4.848093746725558e-01 |
| 3 | 4.526129963807856e-02 | 7.273626342270340e-01 | 1.363186828864830e-01 | 1.363186828864830e-01 |
| 3 | 5.701965545220250e-03 | 9.588790888518748e-01 | 2.056045557406259e-02 | 2.056045557406259e-02 |
| 3 | -3.082950357078510e-12 | -1.637644137683095e+00 | 1.318822068841548e+00 | 1.318822068841548e+00 |
| 6 | 6.534161313539429e-02 | 1.488794015915434e-01 | 3.187277444324656e-01 | 5.323928539759910e-01 |
| 6 | 2.857585945671945e-02 | 2.920156913778056e-02 | 2.760761350600847e-01 | 6.947222958021347e-01 |
| 6 | 1.713390735210246e-02 | 2.575366809527307e-02 | 1.124651138407637e-01 | 8.617812180639632e-01 |
| 6 | 3.627538555011575e-10 | -9.545286851797705e-01 | 7.816269316590252e-01 | 1.172901753520745e+00 |

$d = 13$, $n_p = 37$, type $[1, 4, 4]$, quality NO

| | | | | |
|---|---|---|---|---|
| 1 | -1.431504100389215e-01 | 3.333333333333333e-01 | 3.333333333333333e-01 | 3.333333333333333e-01 |
| 3 | 1.098530881576121e-01 | 4.183965005327344e-01 | 2.908017497336328e-01 | 2.908017497336328e-01 |
| 3 | 1.176437320533769e-02 | 2.402918404365186e-02 | 4.879854079781741e-01 | 4.879854079781741e-01 |
| 3 | 4.909285219444239e-02 | 7.065556933723821e-01 | 1.467221533138090e-01 | 1.467221533138090e-01 |
| 3 | 1.308721082996616e-02 | 9.361244323204546e-01 | 3.193778383977269e-02 | 3.193778383977269e-02 |
| 6 | 5.313026593464549e-02 | 1.136297564468251e-01 | 3.355109949107582e-01 | 5.508592486424168e-01 |
| 6 | 2.080815064139438e-02 | 2.107047140020372e-02 | 3.479783894808914e-01 | 6.309511391189049e-01 |
| 6 | 2.468788956691464e-02 | 2.906693434825857e-02 | 1.591229044853649e-01 | 8.118101611663765e-01 |
| 6 | 3.186565840020815e-12 | -1.429663250493880e+00 | 7.338637432875792e-02 | 2.356276876165122e+00 |

$d = 13$, $n_p = 37$, type $[1, 4, 4]$, quality NO

| | | | | |
|---|---|---|---|---|
| 1 | -9.688924879929315e-01 | 3.333333333333333e-01 | 3.333333333333333e-01 | 3.333333333333333e-01 |
| 3 | 3.884405258615987e-01 | 3.761394010171109e-01 | 3.119302994914446e-01 | 3.119302994914446e-01 |
| 3 | 5.013374111155032e-02 | 7.053689928729936e-01 | 1.473155035635032e-01 | 1.473155035635032e-01 |
| 3 | 1.391408043300610e-02 | 9.342232304732655e-01 | 3.288838476336726e-02 | 3.288838476336726e-02 |
| 3 | -2.479543272592906e-02 | 1.631468804221832e-01 | 4.184265597889084e-01 | 4.184265597889084e-01 |
| 6 | 6.235534309525672e-02 | 1.207470045979425e-01 | 3.420461167460383e-01 | 5.372068786560192e-01 |
| 6 | 2.613289077288576e-02 | 2.224013136102244e-02 | 3.720248490670640e-01 | 6.057350195719135e-01 |
| 6 | 2.581405678843072e-02 | 2.891060343979004e-02 | 1.651414492747100e-01 | 8.059479472855000e-01 |
| 6 | 2.135693912699861e-12 | -1.513523180297373e+00 | 7.001175879918162e-02 | 2.443511421498192e+00 |

$d = 13$, $n_p = 37$, type $[1, 4, 4]$, quality PC

| | | | | |
|---|---|---|---|---|
| 1 | 5.327701422379910e-02 | 3.333333333333333e-01 | 3.333333333333333e-01 | 3.333333333333333e-01 |
| 3 | 4.956315504016233e-02 | 1.738578929713038e-01 | 4.130710535143481e-01 | 4.130710535143481e-01 |
| 3 | 5.184743450421248e-02 | 5.570211705161545e-01 | 2.214894147419227e-01 | 2.214894147419227e-01 |
| 3 | 3.766685008734954e-02 | 7.557962440396628e-01 | 1.221018779801686e-01 | 1.221018779801686e-01 |
| 3 | 1.009316588867590e-02 | 9.443755198018481e-01 | 2.781224009907596e-02 | 2.781224009907596e-02 |
| 6 | 4.566482382925503e-02 | 7.675670629433959e-02 | 3.184561988612754e-01 | 6.047870948443850e-01 |
| 6 | 1.762860882973527e-02 | 1.287778573646135e-02 | 3.548264300679861e-01 | 6.322957841955526e-01 |
| 6 | 1.890097406130929e-02 | 2.293186716326466e-02 | 1.445646443036824e-01 | 8.325034885330530e-01 |
| 6 | 1.007454815533763e-03 | 4.079162664420078e-02 | 4.796e-01-i*2.118e-01 | 4.796e-01+i*2.118e-01 |

$d = 13$, $n_p = 37$, type $[1, 4, 4]$, quality PC

| | | | | |
|---|---|---|---|---|
| 1 | 6.582556142567921e-02 | 3.333333333333333e-01 | 3.333333333333333e-01 | 3.333333333333333e-01 |
| 3 | 5.525921608742764e-02 | 1.484711760712435e-01 | 4.257644119643782e-01 | 4.257644119643782e-01 |
| 3 | 5.680041226967791e-02 | 5.544982563976321e-01 | 2.227508718011840e-01 | 2.227508718011840e-01 |
| 3 | 3.436273251687278e-02 | 7.568504274137131e-01 | 1.215747862931434e-01 | 1.215747862931434e-01 |
| 3 | 8.285172168256209e-03 | 9.495344922596102e-01 | 2.523275387019491e-02 | 2.523275387019491e-02 |
| 6 | 4.098891449773591e-02 | 6.912312355386110e-02 | 2.944370813739796e-01 | 6.364397950721593e-01 |
| 6 | 1.106678247224028e-02 | 6.313971288073639e-03 | 3.136505386724772e-01 | 6.800354900394491e-01 |
| 6 | 1.739179114554864e-02 | 2.395407663318719e-02 | 1.297249348983630e-01 | 8.463209884684498e-01 |
| 6 | 8.894485125744692e-03 | 2.783879297326313e-02 | 4.861e-01-i*8.183e-02 | 4.861e-01+i*8.183e-02 |

$d = 13$, $n_p = 37$, type $[1, 4, 4]$, quality NC

| | | | | |
|---|---|---|---|---|
| 1 | 8.900137113715172e-02 | 3.333333333333333e-01 | 3.333333333333333e-01 | 3.333333333333333e-01 |
| 3 | 7.690330230531596e-02 | 5.642491373489309e-01 | 2.178754313255346e-01 | 2.178754313255346e-01 |
| 3 | 6.986875208423810e-02 | 9.898452298088092e-02 | 4.505077385095595e-01 | 4.505077385095595e-01 |
| 3 | 3.988624516757436e-02 | 7.759480776875440e-01 | 1.120259611562280e-01 | 1.120259611562280e-01 |
| 3 | 8.994603341891589e-03 | -7.331395351972058e-03 | 5.036656976759860e-01 | 5.036656976759860e-01 |
| 6 | 3.878201400822055e-02 | 3.968999237923934e-02 | 2.832946834976565e-01 | 6.770153241231041e-01 |
| 6 | 1.286782607395437e-02 | 1.081941212565521e-02 | 1.128548946007767e-01 | 8.763256932735681e-01 |
| 6 | 2.362098932469997e-03 | 1.862e-02-i*2.673e-02 | 1.862e-02+i*2.673e-02 | 9.627627700030414e-01 |
| 6 | -5.285653680206915e-06 | 1.812e-01-i*3.789e-01 | 1.812e-01+i*3.789e-01 | 6.376908811245179e-01 |

$d = 13$, $n_p = 37$, type $[1, 4, 4]$, quality NC

| | | | | |
|---|---|---|---|---|
| 1 | -6.229467305784935e-01 | 3.333333333333333e-01 | 3.333333333333333e-01 | 3.333333333333333e-01 |
| 3 | 2.509370896722812e-01 | 3.683510780673502e-01 | 3.158244609663249e-01 | 3.158244609663249e-01 |
| 3 | 4.371574692447432e-02 | 7.398987768928085e-01 | 1.300506115535957e-01 | 1.300506115535957e-01 |
| 3 | 1.133777402596749e-02 | 9.410433056655650e-01 | 2.947834716721750e-02 | 2.947834716721750e-02 |
| 3 | 4.762650088787337e-06 | -1.950607405563629e-01 | 5.975303702781815e-01 | 5.975303702781815e-01 |
| 6 | 6.156040207959973e-02 | 1.365723540950427e-01 | 3.134997480437585e-01 | 5.499278978611988e-01 |
| 6 | 3.482239076903912e-02 | 2.878621367963786e-02 | 3.588580371393092e-01 | 6.123557491810530e-01 |
| 6 | 2.103709467788147e-02 | 2.417237074149550e-02 | 1.529613736319179e-01 | 8.228662556265866e-01 |
| 6 | 7.354760015604281e-05 | 6.054058390846535e-02 | 4.697e-01-i*3.462e-01 | 4.697e-01+i*3.462e-01 |

$d = 13$, $n_p = 37$, type $[1, 4, 4]$, quality NC

| | | | | |
|---|---|---|---|---|
| 1 | -1.374797596941201e+00 | 3.333333333333333e-01 | 3.333333333333333e-01 | 3.333333333333333e-01 |
| 3 | 5.152174344813276e-01 | 3.008465621703329e-01 | 3.495767189148336e-01 | 3.495767189148336e-01 |
| 3 | 3.530102475817532e-02 | 7.723079453051379e-01 | 1.138460273474310e-01 | 1.138460273474310e-01 |
| 3 | 9.323482434761800e-03 | 9.463937175749520e-01 | 2.680314121252402e-02 | 2.680314121252402e-02 |
| 3 | 5.859823745093778e-03 | -2.712455686895237e-03 | 5.013562278434476e-01 | 5.013562278434476e-01 |
| 6 | 5.717651206557081e-02 | 1.302259211900409e-01 | 2.831675629283798e-01 | 5.866065158815793e-01 |
| 6 | 3.009258344463333e-02 | 2.964086504452444e-02 | 3.127385667170466e-01 | 6.576205682384289e-01 |
| 6 | 1.574840736163642e-02 | 2.016688940300140e-02 | 1.377611450058289e-01 | 8.420719655911697e-01 |
| 6 | 9.931213908680345e-03 | 6.987642286542089e-02 | 4.651e-01-i*1.090e-01 | 4.651e-01+i*1.090e-01 |

$d = 13$, $n_p = 37$, type $[1, 4, 4]$, quality NC

| | | | | |
|---|---|---|---|---|
| 1 | -6.052313060850973e-01 | 3.333333333333333e-01 | 3.333333333333333e-01 | 3.333333333333333e-01 |
| 3 | 2.770923494621823e-01 | 2.737918662917410e-01 | 3.631040668541295e-01 | 3.631040668541295e-01 |
| 3 | 4.761520370971413e-02 | 4.302801512884106e-02 | 4.784859924355795e-01 | 4.784859924355795e-01 |
| 3 | 4.522135351177988e-02 | 8.231240273009565e-01 | 8.843798634952175e-02 | 8.843798634952175e-02 |
| 3 | 1.219952710253470e-02 | 9.403065994532564e-01 | 2.984670027337179e-02 | 2.984670027337179e-02 |
| 6 | 6.144801054218288e-02 | 1.113089327964524e-01 | 2.654642528038222e-01 | 6.232268143997254e-01 |
| 6 | 1.550879715781349e-02 | 1.185656449316256e-03 | 2.633419069948082e-01 | 7.354724365558755e-01 |
| 6 | 1.286866170951235e-06 | -6.251e-02-i*2.897e-01 | -6.251e-02+i*2.897e-01 | 1.125029189582666e+00 |
| 6 | -4.837604450899225e-04 | 3.184e-02-i*1.286e-01 | 3.184e-02+i*1.286e-01 | 9.363268303868305e-01 |

$d = 13$, $n_p = 37$, type $[1, 4, 4]$, quality NC

| | | | | |
|---|---|---|---|---|
| 1 | -1.812145819046238e-01 | 3.333333333333333e-01 | 3.333333333333333e-01 | 3.333333333333333e-01 |
| 3 | 1.228349023857947e-01 | 4.133773994507944e-01 | 2.933113002746028e-01 | 2.933113002746028e-01 |
| 3 | 3.539080940513252e-02 | 1.994988867454507e-02 | 4.900250556627275e-01 | 4.900250556627275e-01 |
| 3 | 4.974673121073023e-02 | 7.018252756730103e-01 | 1.490873621634948e-01 | 1.490873621634948e-01 |
| 3 | 2.208268402502157e-02 | 9.143042754579791e-01 | 4.284786227101044e-02 | 4.284786227101044e-02 |
| 6 | 5.252142325818130e-02 | 1.123838137023100e-01 | 3.374127376003617e-01 | 5.502034486973284e-01 |
| 6 | 2.974079836291232e-02 | 2.701912219223362e-02 | 2.056707729754690e-01 | 7.673101048322974e-01 |
| 6 | 3.301622611989690e-05 | -1.295146073943166e-01 | 4.825428041983074e-02 | 1.081260326974486e+00 |
| 6 | -4.537043764490737e-04 | 1.098689500969775e-02 | 4.945e-01-i*2.468e-01 | 4.945e-01+i*2.468e-01 |

$d = 13$, $n_p = 37$, type $[1, 4, 4]$, quality NC

| | | | | |
|---|---|---|---|---|
| 1 | 8.265550196285195e-02 | 3.333333333333333e-01 | 3.333333333333333e-01 | 3.333333333333333e-01 |
| 3 | 3.683198801467296e-02 | 3.011937458711750e-02 | 4.849403127064412e-01 | 4.849403127064412e-01 |
| 3 | 4.500425669666815e-02 | 7.456046629999698e-01 | 1.271976685000151e-01 | 1.271976685000151e-01 |
| 3 | 4.184194426232192e-04 | 1.029681062244632e+00 | -1.484053112231597e-02 | -1.484053112231597e-02 |
| 3 | 1.309797017081165e-08 | -5.524330716188160e-01 | 7.762165358094080e-01 | 7.762165358094080e-01 |
| 6 | 6.773178966269137e-02 | 1.474761035201529e-01 | 3.148350538932194e-01 | 5.376888425866277e-01 |
| 6 | 3.011123786839425e-02 | 2.821486740596230e-02 | 2.545733848005434e-01 | 7.172117477934943e-01 |
| 6 | 1.392040336828142e-02 | 1.934903564248239e-02 | 8.069268802237129e-02 | 8.999582763351463e-01 |
| 6 | -1.985247628357332e-08 | -4.428531015491356e-02 | 5.221e-01-i*7.720e-01 | 5.221e-01+i*7.720e-01 |

$d = 13$, $n_p = 37$, type $[1, 4, 4]$, quality NC

| | | | | |
|---|---|---|---|---|
| 1 | 9.068207950896532e-02 | 3.333333333333333e-01 | 3.333333333333333e-01 | 3.333333333333333e-01 |
| 3 | 2.624621005226525e-01 | 1.535741418096078e-01 | 4.232129290951961e-01 | 4.232129290951961e-01 |
| 3 | 3.038942455930421e-02 | 2.718695432246124e-02 | 4.864065228387694e-01 | 4.864065228387694e-01 |
| 3 | 5.707010054001433e-02 | 6.971297869824137e-01 | 1.514351065087931e-01 | 1.514351065087931e-01 |
| 3 | 4.699215895018137e-03 | 9.648413260083125e-01 | 1.757933699584375e-02 | 1.757933699584375e-02 |
| 6 | 3.084069992351499e-02 | 3.144565778856376e-02 | 2.748608789144515e-01 | 6.936934632969848e-01 |
| 6 | 1.884779108854913e-02 | 2.791667627891237e-02 | 1.096794345862066e-01 | 8.624038891348811e-01 |
| 6 | 3.502717198964019e-08 | -4.638580655695387e-01 | 3.947576811936851e-01 | 1.069100384375854e+00 |
| 6 | -7.544596004922492e-02 | 1.590169338273293e-01 | 4.205e-01-i*7.057e-02 | 4.205e-01+i*7.057e-02 |

$d = 13$, $n_p = 37$, type $[1, 4, 4]$, quality NC

| | | | | |
|---|---|---|---|---|
| 1 | -4.603093100903433e-02 | 3.333333333333333e-01 | 3.333333333333333e-01 | 3.333333333333333e-01 |
| 3 | 7.542485117106085e-02 | 4.361562641535820e-01 | 2.819218679232090e-01 | 2.819218679232090e-01 |
| 3 | 4.792131665116771e-02 | 7.182928055519864e-01 | 1.408535972240068e-01 | 1.408535972240068e-01 |
| 3 | 1.277446364441980e-02 | 9.372616325959613e-01 | 3.136918370201933e-02 | 3.136918370201933e-02 |
| 3 | 1.695907003266448e-21 | -8.023500942434875e+00 | 4.511750471217437e+00 | 4.511750471217437e+00 |
| 6 | 5.470668829202123e-02 | 1.181154790317033e-01 | 3.318492572812515e-01 | 5.500352636870452e-01 |
| 6 | 2.749784723078251e-02 | 2.316904466412991e-02 | 3.691863252531523e-01 | 6.076446300827178e-01 |
| 6 | 2.407356442971929e-02 | 2.704696827624587e-02 | 1.604192907302339e-01 | 8.125337409935203e-01 |
| 6 | 7.281565851725047e-08 | 6.350040341831263e-02 | 4.682e-01-i*7.556e-01 | 4.682e-01+i*7.556e-01 |

$d = 13$, $n_p = 37$, type $[1, 4, 4]$, quality CC

| | | | | |
|---|---|---|---|---|
| 1 | 1.310888773539221e-01 | 3.333333333333333e-01 | 3.333333333333333e-01 | 3.333333333333333e-01 |
| 3 | 5.562729298583807e-02 | 1.296737192623555e-01 | 4.351631403688223e-01 | 4.351631403688223e-01 |
| 3 | 2.681547925070409e-02 | 8.378220762055029e-01 | 8.108896189724853e-02 | 8.108896189724853e-02 |
| 3 | 1.029e-04-i*1.851e-03 | 4.268e-01+i*2.085e-01 | 2.866e-01-i*1.042e-01 | 2.866e-01-i*1.042e-01 |
| 3 | 1.029e-04+i*1.851e-03 | 4.268e-01-i*2.085e-01 | 2.866e-01+i*1.042e-01 | 2.866e-01+i*1.042e-01 |
| 6 | 5.236109820173689e-02 | 1.255693302051869e-01 | 2.427375468614003e-01 | 6.316931229334127e-01 |
| 6 | 2.647414927450817e-02 | 2.518964216375821e-02 | 3.827741904732067e-01 | 5.920361673630350e-01 |
| 6 | 1.954475219007801e-02 | 2.248279490124633e-02 | 1.927209962236042e-01 | 7.847962088751495e-01 |
| 6 | 5.114222537734984e-03 | 5.122038056876521e-03 | 5.090042760280465e-02 | 9.439775343403188e-01 |

$d = 13$, $n_p = 37$, type $[1, 4, 4]$, quality CC

| | | | | |
|---|---|---|---|---|
| 1 | 7.061777044728916e-02 | 3.333333333333333e-01 | 3.333333333333333e-01 | 3.333333333333333e-01 |
| 3 | 6.376467958275305e-02 | 1.291178098125080e-01 | 4.354410950937460e-01 | 4.354410950937460e-01 |
| 3 | 6.000841373519355e-02 | 5.485357926774912e-01 | 2.257321036612544e-01 | 2.257321036612544e-01 |
| 3 | 3.419478764257396e-02 | 2.488033520132759e-02 | 4.875598323993362e-01 | 4.875598323993362e-01 |
| 3 | 2.287608312878228e-02 | 9.184092163381360e-01 | 4.079539183093199e-02 | 4.079539183093199e-02 |
| 6 | 5.034939863399181e-02 | 7.527239234555322e-02 | 2.190830977852264e-01 | 7.056445098692204e-01 |
| 6 | 1.413754390168612e-02 | 8.376628474483748e-03 | 2.270309953676205e-01 | 7.645923761578957e-01 |
| 6 | -5.943e-06-i*1.669e-04 | 4.183e-02+i*5.940e-03 | 8.658e-02-i*2.321e-01 | 8.716e-01+i*2.262e-01 |
| 6 | -5.943e-06+i*1.669e-04 | 4.183e-02-i*5.940e-03 | 8.658e-02+i*2.321e-01 | 8.716e-01-i*2.262e-01 |

$d = 13$, $n_p = 37$, type $[1, 4, 4]$, quality CC

| | | | | |
|---|---|---|---|---|
| 1 | 8.245e-02-i*4.363e-03 | 3.333333333333333e-01 | 3.333333333333333e-01 | 3.333333333333333e-01 |
| 3 | 6.935e-02-i*5.187e-03 | 1.354e-01-i*1.084e-03 | 4.323e-01+i*5.419e-04 | 4.323e-01+i*5.419e-04 |
| 3 | 7.195e-02-i*6.616e-03 | 5.951e-01-i*2.257e-02 | 2.025e-01+i*1.129e-02 | 2.025e-01+i*1.129e-02 |
| 3 | 3.245e-02-i*5.810e-03 | 2.532e-02-i*2.767e-03 | 4.873e-01+i*1.383e-03 | 4.873e-01+i*1.383e-03 |
| 3 | 3.796e-02+i*1.412e-02 | 8.990e-01-i*4.099e-02 | 5.051e-02+i*2.049e-02 | 5.051e-02+i*2.049e-02 |
| 6 | 5.145e-02+i*1.495e-03 | 4.491e-02+i*1.021e-02 | 2.375e-01+i*2.335e-02 | 7.176e-01-i*3.357e-02 |
| 6 | -1.603e-03+i*6.389e-04 | -2.290e-02+i*6.299e-02 | 2.280e-01-i*7.634e-03 | 7.949e-01-i*5.536e-02 |
| 6 | 5.183e-06+i*4.038e-05 | 6.882e-02+i*1.400e-03 | 9.450e-02+i*3.426e-01 | 8.367e-01-i*3.440e-01 |
| 6 | -2.776e-03+i*2.994e-04 | -9.580e-03+i*6.095e-02 | 4.852e-02+i*1.057e-02 | 9.611e-01-i*7.152e-02 |

$d = 13$, $n_p = 37$, type $[1, 4, 4]$, quality CC

| | | | | |
|---|---|---|---|---|
| 1 | 8.245e-02+i*4.363e-03 | 3.333333333333333e-01 | 3.333333333333333e-01 | 3.333333333333333e-01 |
| 3 | 6.935e-02+i*5.187e-03 | 1.354e-01+i*1.084e-03 | 4.323e-01-i*5.419e-04 | 4.323e-01-i*5.419e-04 |
| 3 | 7.195e-02+i*6.616e-03 | 5.951e-01+i*2.257e-02 | 2.025e-01-i*1.129e-02 | 2.025e-01-i*1.129e-02 |
| 3 | 3.245e-02+i*5.810e-03 | 2.532e-02+i*2.767e-03 | 4.873e-01-i*1.383e-03 | 4.873e-01-i*1.383e-03 |
| 3 | 3.796e-02-i*1.412e-02 | 8.990e-01+i*4.099e-02 | 5.051e-02-i*2.049e-02 | 5.051e-02-i*2.049e-02 |
| 6 | 5.145e-02-i*1.495e-03 | 4.491e-02-i*1.021e-02 | 2.375e-01-i*2.335e-02 | 7.176e-01+i*3.357e-02 |
| 6 | -1.603e-03-i*6.389e-04 | -2.290e-02-i*6.299e-02 | 2.280e-01+i*7.634e-03 | 7.949e-01+i*5.536e-02 |
| 6 | 5.183e-06-i*4.038e-05 | 6.882e-02-i*1.400e-03 | 9.450e-02-i*3.426e-01 | 8.367e-01+i*3.440e-01 |
| 6 | -2.776e-03-i*2.994e-04 | -9.580e-03-i*6.095e-02 | 4.852e-02-i*1.057e-02 | 9.611e-01+i*7.152e-02 |

$d = 13$, $n_p = 37$, type $[1, 4, 4]$, quality CC

| | | | | |
|---|---|---|---|---|
| 1 | -3.363e-02+i*6.774e-02 | 3.333333333333333e-01 | 3.333333333333333e-01 | 3.333333333333333e-01 |
| 3 | 7.354e-02-i*2.060e-02 | 4.368e-01+i*2.330e-02 | 2.816e-01-i*1.165e-02 | 2.816e-01-i*1.165e-02 |
| 3 | 5.038e-02+i*3.433e-03 | 1.156e-01+i*3.957e-03 | 4.422e-01-i*1.979e-03 | 4.422e-01-i*1.979e-03 |
| 3 | 2.414e-02-i*3.224e-03 | 7.774e-01+i*1.860e-02 | 1.113e-01-i*9.302e-03 | 1.113e-01-i*9.302e-03 |
| 3 | 1.561e-02+i*4.470e-03 | 9.333e-01-i*1.213e-02 | 3.336e-02+i*6.064e-03 | 3.336e-02+i*6.064e-03 |
| 6 | 4.452e-02+i*3.425e-04 | 1.176e-01-i*4.586e-03 | 2.514e-01-i*8.664e-03 | 6.310e-01+i*1.325e-02 |
| 6 | 2.498e-02-i*9.044e-04 | 2.258e-02+i*4.522e-04 | 3.786e-01+i*6.137e-03 | 5.988e-01-i*6.589e-03 |
| 6 | 2.082e-02-i*2.374e-03 | 2.309e-02-i*2.364e-03 | 1.782e-01+i*1.467e-02 | 7.987e-01-i*1.230e-02 |
| 6 | 1.153e-04-i*3.943e-04 | 8.314e-03+i*1.040e-01 | 3.825e-02-i*7.549e-03 | 9.534e-01-i*9.641e-02 |

$d = 13$, $n_p = 37$, type $[1, 4, 4]$, quality CC

| | | | | |
|---|---|---|---|---|
| 1 | -3.363e-02-i*6.774e-02 | 3.333333333333333e-01 | 3.333333333333333e-01 | 3.333333333333333e-01 |
| 3 | 7.354e-02+i*2.060e-02 | 4.368e-01-i*2.330e-02 | 2.816e-01+i*1.165e-02 | 2.816e-01+i*1.165e-02 |
| 3 | 5.038e-02-i*3.433e-03 | 1.156e-01-i*3.957e-03 | 4.422e-01+i*1.979e-03 | 4.422e-01+i*1.979e-03 |
| 3 | 2.414e-02+i*3.224e-03 | 7.774e-01-i*1.860e-02 | 1.113e-01+i*9.302e-03 | 1.113e-01+i*9.302e-03 |
| 3 | 1.561e-02-i*4.470e-03 | 9.333e-01+i*1.213e-02 | 3.336e-02-i*6.064e-03 | 3.336e-02-i*6.064e-03 |
| 6 | 4.452e-02-i*3.425e-04 | 1.176e-01+i*4.586e-03 | 2.514e-01+i*8.664e-03 | 6.310e-01-i*1.325e-02 |
| 6 | 2.498e-02+i*9.044e-04 | 2.258e-02-i*4.522e-04 | 3.786e-01-i*6.137e-03 | 5.988e-01+i*6.589e-03 |
| 6 | 2.082e-02+i*2.374e-03 | 2.309e-02+i*2.364e-03 | 1.782e-01-i*1.467e-02 | 7.987e-01+i*1.230e-02 |
| 6 | 1.153e-04+i*3.943e-04 | 8.314e-03-i*1.040e-01 | 3.825e-02+i*7.549e-03 | 9.534e-01+i*9.641e-02 |

$d = 13$, $n_p = 37$, type $[1, 4, 4]$, quality CC

| | | | | |
|---|---|---|---|---|
| 1 | 7.009e-02-i*2.495e-03 | 3.333333333333333e-01 | 3.333333333333333e-01 | 3.333333333333333e-01 |
| 3 | 6.186e-02+i*7.146e-04 | 1.312e-01-i*2.399e-03 | 4.344e-01+i*1.200e-03 | 4.344e-01+i*1.200e-03 |
| 3 | 5.941e-02-i*1.340e-03 | 5.481e-01-i*8.013e-03 | 2.260e-01+i*4.007e-03 | 2.260e-01+i*4.007e-03 |
| 3 | 3.080e-02+i*3.681e-03 | 2.358e-02+i*2.824e-03 | 4.882e-01-i*1.412e-03 | 4.882e-01-i*1.412e-03 |
| 3 | 1.133e-02+i*4.855e-03 | 9.403e-01-i*1.065e-02 | 2.984e-02+i*5.323e-03 | 2.984e-02+i*5.323e-03 |
| 6 | 5.536e-02-i*1.149e-02 | 7.441e-02+i*9.199e-03 | 2.195e-01-i*1.682e-02 | 7.061e-01+i*7.622e-03 |
| 6 | -4.194e-03+i*6.634e-03 | 5.432e-02+i*1.282e-02 | 2.370e-01-i*1.187e-01 | 7.087e-01+i*1.059e-01 |
| 6 | 1.361e-02-i*5.253e-03 | 9.541e-03-i*2.649e-03 | 2.314e-01+i*2.695e-02 | 7.591e-01-i*2.430e-02 |
| 6 | 8.505e-03+i*6.569e-03 | 2.970e-02-i*3.651e-03 | 1.242e-01+i*6.187e-02 | 8.461e-01-i*5.822e-02 |

$d = 13$, $n_p = 37$, type $[1, 4, 4]$, quality CC

| | | | | |
|---|---|---|---|---|
| 1 | 7.009e-02+i*2.495e-03 | 3.333333333333333e-01 | 3.333333333333333e-01 | 3.333333333333333e-01 |
| 3 | 6.186e-02-i*7.146e-04 | 1.312e-01+i*2.399e-03 | 4.344e-01-i*1.200e-03 | 4.344e-01-i*1.200e-03 |
| 3 | 5.941e-02+i*1.340e-03 | 5.481e-01+i*8.013e-03 | 2.260e-01-i*4.007e-03 | 2.260e-01-i*4.007e-03 |
| 3 | 3.080e-02-i*3.681e-03 | 2.358e-02-i*2.824e-03 | 4.882e-01+i*1.412e-03 | 4.882e-01+i*1.412e-03 |
| 3 | 1.133e-02-i*4.855e-03 | 9.403e-01+i*1.065e-02 | 2.984e-02-i*5.323e-03 | 2.984e-02-i*5.323e-03 |
| 6 | 5.536e-02+i*1.149e-02 | 7.441e-02-i*9.199e-03 | 2.195e-01+i*1.682e-02 | 7.061e-01-i*7.622e-03 |
| 6 | -4.194e-03-i*6.634e-03 | 5.432e-02-i*1.282e-02 | 2.370e-01+i*1.187e-01 | 7.087e-01-i*1.059e-01 |
| 6 | 1.361e-02+i*5.253e-03 | 9.541e-03+i*2.649e-03 | 2.314e-01-i*2.695e-02 | 7.591e-01+i*2.430e-02 |
| 6 | 8.505e-03-i*6.569e-03 | 2.970e-02+i*3.651e-03 | 1.242e-01-i*6.187e-02 | 8.461e-01+i*5.822e-02 |

$d = 13$, $n_p = 37$, type $[1, 4, 4]$, quality CC

| | | | | |
|---|---|---|---|---|
| 1 | 7.525e-02+i*3.185e-02 | 3.333333333333333e-01 | 3.333333333333333e-01 | 3.333333333333333e-01 |
| 3 | 1.165e-02-i*2.589e-03 | 4.484e-01+i*9.590e-02 | 2.758e-01-i*4.795e-02 | 2.758e-01-i*4.795e-02 |
| 3 | 4.427e-02+i*2.332e-03 | 7.370e-01-i*1.033e-02 | 1.315e-01+i*5.166e-03 | 1.315e-01+i*5.166e-03 |
| 3 | -2.585e-06-i*1.887e-07 | -2.057e-01-i*1.237e-01 | 6.028e-01+i*6.185e-02 | 6.028e-01+i*6.185e-02 |
| 3 | 1.149e-02+i*5.496e-04 | 9.406e-01-i*1.452e-03 | 2.968e-02+i*7.259e-04 | 2.968e-02+i*7.259e-04 |
| 6 | 6.400e-02-i*4.137e-03 | 1.404e-01-i*6.380e-03 | 3.139e-01+i*8.168e-03 | 5.457e-01-i*1.788e-03 |
| 6 | 3.491e-02-i*2.676e-03 | 2.888e-02-i*1.882e-03 | 3.612e-01+i*4.971e-03 | 6.099e-01-i*3.090e-03 |
| 6 | -2.087e-05-i*4.492e-05 | 6.145e-02+i*1.297e-03 | 3.707e-01+i*3.607e-01 | 5.679e-01-i*3.620e-01 |
| 6 | 2.153e-02+i*1.403e-03 | 2.460e-02+i*1.308e-03 | 1.541e-01+i*3.075e-03 | 8.213e-01-i*4.384e-03 |

$d = 13$, $n_p = 37$, type $[1, 4, 4]$, quality CC

| | | | | |
|---|---|---|---|---|
| 1 | 7.525e-02-i*3.185e-02 | 3.333333333333333e-01 | 3.333333333333333e-01 | 3.333333333333333e-01 |
| 3 | 1.165e-02+i*2.589e-03 | 4.484e-01-i*9.590e-02 | 2.758e-01+i*4.795e-02 | 2.758e-01+i*4.795e-02 |
| 3 | 4.427e-02-i*2.332e-03 | 7.370e-01+i*1.033e-02 | 1.315e-01-i*5.166e-03 | 1.315e-01-i*5.166e-03 |
| 3 | -2.585e-06+i*1.887e-07 | -2.057e-01+i*1.237e-01 | 6.028e-01-i*6.185e-02 | 6.028e-01-i*6.185e-02 |
| 3 | 1.149e-02-i*5.496e-04 | 9.406e-01+i*1.452e-03 | 2.968e-02-i*7.259e-04 | 2.968e-02-i*7.259e-04 |
| 6 | 6.400e-02+i*4.137e-03 | 1.404e-01+i*6.380e-03 | 3.139e-01-i*8.168e-03 | 5.457e-01+i*1.788e-03 |
| 6 | 3.491e-02+i*2.676e-03 | 2.888e-02+i*1.882e-03 | 3.612e-01-i*4.971e-03 | 6.099e-01+i*3.090e-03 |
| 6 | -2.087e-05+i*4.492e-05 | 6.145e-02-i*1.297e-03 | 3.707e-01-i*3.607e-01 | 5.679e-01+i*3.620e-01 |
| 6 | 2.153e-02-i*1.403e-03 | 2.460e-02-i*1.308e-03 | 1.541e-01-i*3.075e-03 | 8.213e-01+i*4.384e-03 |

$d = 13$, $n_p = 37$, type $[1, 4, 4]$, quality CC

| | | | | |
|---|---|---|---|---|
| 1 | 7.082534281154145e-02 | 3.333333333333333e-01 | 3.333333333333333e-01 | 3.333333333333333e-01 |
| 3 | 6.208746428064061e-02 | 1.298498269353057e-01 | 4.350750865323471e-01 | 4.350750865323471e-01 |
| 3 | 6.049431887859109e-02 | 5.492015635508979e-01 | 2.253992182245510e-01 | 2.253992182245510e-01 |
| 3 | 2.773645794511300e-02 | 1.998295356567991e-02 | 4.900085232171600e-01 | 4.900085232171600e-01 |
| 3 | 1.137431080107364e-02 | 9.416835806542733e-01 | 2.915820967286334e-02 | 2.915820967286334e-02 |
| 6 | 5.688607549803780e-02 | 6.837274981862250e-02 | 2.422665053173885e-01 | 6.893607448639890e-01 |
| 6 | 2.831427958686885e-02 | 1.999721588487616e-02 | 1.752945459555348e-01 | 8.047082381595890e-01 |
| 6 | -5.592e-03-i*2.261e-03 | 3.254e-02+i*2.940e-02 | 1.902e-01-i*1.018e-01 | 7.772e-01+i*7.236e-02 |
| 6 | -5.592e-03+i*2.261e-03 | 3.254e-02-i*2.940e-02 | 1.902e-01+i*1.018e-01 | 7.772e-01-i*7.236e-02 |

$d = 13$, $n_p = 37$, type $[1, 4, 4]$, quality CC

| | | | | |
|---|---|---|---|---|
| 1 | 6.471e-02-i*1.127e-02 | 3.333333333333333e-01 | 3.333333333333333e-01 | 3.333333333333333e-01 |
| 3 | 3.983e-02+i*5.264e-03 | 4.128e-02+i*8.201e-03 | 4.794e-01-i*4.101e-03 | 4.794e-01-i*4.101e-03 |
| 3 | -5.424e-04+i*2.654e-04 | -3.958e-02+i*6.294e-02 | 5.198e-01-i*3.147e-02 | 5.198e-01-i*3.147e-02 |
| 3 | 2.468e-02+i*6.153e-03 | 7.997e-01-i*2.267e-02 | 1.002e-01+i*1.134e-02 | 1.002e-01+i*1.134e-02 |
| 3 | 8.389e-03+i*3.408e-04 | 9.493e-01-i*1.239e-03 | 2.537e-02+i*6.195e-04 | 2.537e-02+i*6.195e-04 |
| 6 | 5.361e-02-i*9.069e-03 | 1.650e-01+i*1.311e-02 | 3.241e-01+i*4.167e-03 | 5.109e-01-i*1.728e-02 |
| 6 | 2.953e-02+i*4.439e-03 | 1.088e-01+i*6.250e-03 | 2.246e-01+i*2.908e-02 | 6.666e-01-i*3.533e-02 |
| 6 | 2.300e-02-i*7.837e-04 | 2.489e-02-i*9.175e-04 | 2.977e-01-i*1.845e-03 | 6.774e-01+i*2.763e-03 |
| 6 | 1.357e-02+i*1.282e-03 | 1.816e-02+i*2.342e-03 | 1.317e-01-i*8.775e-04 | 8.501e-01-i*1.464e-03 |

$d = 13$, $n_p = 37$, type $[1, 4, 4]$, quality CC

| | | | | |
|---|---|---|---|---|
| 1 | 6.471e-02+i*1.127e-02 | 3.333333333333333e-01 | 3.333333333333333e-01 | 3.333333333333333e-01 |
| 3 | 3.983e-02-i*5.264e-03 | 4.128e-02-i*8.201e-03 | 4.794e-01+i*4.101e-03 | 4.794e-01+i*4.101e-03 |
| 3 | -5.424e-04-i*2.654e-04 | -3.958e-02-i*6.294e-02 | 5.198e-01+i*3.147e-02 | 5.198e-01+i*3.147e-02 |
| 3 | 2.468e-02-i*6.153e-03 | 7.997e-01+i*2.267e-02 | 1.002e-01-i*1.134e-02 | 1.002e-01-i*1.134e-02 |
| 3 | 8.389e-03-i*3.408e-04 | 9.493e-01+i*1.239e-03 | 2.537e-02-i*6.195e-04 | 2.537e-02-i*6.195e-04 |
| 6 | 5.361e-02+i*9.069e-03 | 1.650e-01-i*1.311e-02 | 3.241e-01-i*4.167e-03 | 5.109e-01+i*1.728e-02 |
| 6 | 2.953e-02-i*4.439e-03 | 1.088e-01-i*6.250e-03 | 2.246e-01-i*2.908e-02 | 6.666e-01+i*3.533e-02 |
| 6 | 2.300e-02+i*7.837e-04 | 2.489e-02+i*9.175e-04 | 2.977e-01+i*1.845e-03 | 6.774e-01-i*2.763e-03 |
| 6 | 1.357e-02-i*1.282e-03 | 1.816e-02-i*2.342e-03 | 1.317e-01+i*8.775e-04 | 8.501e-01+i*1.464e-03 |

$d = 13$, $n_p = 37$, type $[1, 4, 4]$, quality CC

| | | | | |
|---|---|---|---|---|
| 1 | -3.652e-02-i*7.615e-02 | 3.333333333333333e-01 | 3.333333333333333e-01 | 3.333333333333333e-01 |
| 3 | 7.519e-02+i*2.218e-02 | 4.355e-01-i*2.666e-02 | 2.823e-01+i*1.333e-02 | 2.823e-01+i*1.333e-02 |
| 3 | 2.379e-02-i*9.469e-04 | 2.258e-02-i*9.539e-04 | 4.887e-01+i*4.769e-04 | 4.887e-01+i*4.769e-04 |
| 3 | 4.396e-02+i*1.268e-02 | 7.395e-01-i*3.696e-02 | 1.303e-01+i*1.848e-02 | 1.303e-01+i*1.848e-02 |
| 3 | 8.115e-03-i*1.131e-04 | 9.497e-01+i*4.239e-04 | 2.514e-02-i*2.120e-04 | 2.514e-02-i*2.120e-04 |
| 6 | 5.723e-02-i*9.304e-03 | 1.162e-01-i*3.706e-04 | 3.314e-01+i*2.086e-02 | 5.523e-01-i*2.049e-02 |
| 6 | 1.567e-03+i*1.506e-03 | 1.352e-01+i*2.893e-03 | 2.263e-01+i*1.689e-01 | 6.384e-01-i*1.718e-01 |
| 6 | 2.118e-02+i*9.740e-04 | 2.217e-02+i*1.092e-03 | 2.886e-01-i*1.573e-04 | 6.892e-01-i*9.350e-04 |
| 6 | 1.724e-02+i*2.615e-03 | 2.497e-02+i*3.633e-03 | 1.258e-01-i*2.847e-05 | 8.493e-01-i*3.605e-03 |

$d = 13$, $n_p = 37$, type $[1, 4, 4]$, quality CC

| | | | | |
|---|---|---|---|---|
| 1 | -3.652e-02+i*7.615e-02 | 3.333333333333333e-01 | 3.333333333333333e-01 | 3.333333333333333e-01 |
| 3 | 7.519e-02-i*2.218e-02 | 4.355e-01+i*2.666e-02 | 2.823e-01-i*1.333e-02 | 2.823e-01-i*1.333e-02 |
| 3 | 2.379e-02+i*9.469e-04 | 2.258e-02+i*9.539e-04 | 4.887e-01-i*4.769e-04 | 4.887e-01-i*4.769e-04 |
| 3 | 4.396e-02-i*1.268e-02 | 7.395e-01+i*3.696e-02 | 1.303e-01-i*1.848e-02 | 1.303e-01-i*1.848e-02 |
| 3 | 8.115e-03+i*1.131e-04 | 9.497e-01-i*4.239e-04 | 2.514e-02+i*2.120e-04 | 2.514e-02+i*2.120e-04 |
| 6 | 5.723e-02+i*9.304e-03 | 1.162e-01+i*3.706e-04 | 3.314e-01-i*2.086e-02 | 5.523e-01+i*2.049e-02 |
| 6 | 1.567e-03-i*1.506e-03 | 1.352e-01-i*2.893e-03 | 2.263e-01-i*1.689e-01 | 6.384e-01+i*1.718e-01 |
| 6 | 2.118e-02-i*9.740e-04 | 2.217e-02-i*1.092e-03 | 2.886e-01+i*1.573e-04 | 6.892e-01+i*9.350e-04 |
| 6 | 1.724e-02-i*2.615e-03 | 2.497e-02-i*3.633e-03 | 1.258e-01+i*2.847e-05 | 8.493e-01+i*3.605e-03 |

$d = 13$, $n_p = 37$, type $[1, 4, 4]$, quality CC

| | | | | |
|---|---|---|---|---|
| 1 | 7.283e-02-i*1.314e-02 | 3.333333333333333e-01 | 3.333333333333333e-01 | 3.333333333333333e-01 |
| 3 | 5.677e-02+i*9.421e-03 | 1.422e-01+i*1.158e-02 | 4.289e-01-i*5.792e-03 | 4.289e-01-i*5.792e-03 |
| 3 | 2.769e-02+i*1.683e-03 | 2.581e-02+i*2.143e-03 | 4.871e-01-i*1.072e-03 | 4.871e-01-i*1.072e-03 |
| 3 | 3.181e-02-i*2.865e-03 | 7.604e-01+i*2.022e-02 | 1.198e-01-i*1.011e-02 | 1.198e-01-i*1.011e-02 |
| 3 | 7.536e-03+i*7.608e-04 | 9.516e-01-i*2.688e-03 | 2.418e-02+i*1.344e-03 | 2.418e-02+i*1.344e-03 |
| 6 | 4.407e-02-i*2.249e-02 | 1.581e-01+i*3.469e-02 | 2.692e-01-i*2.603e-02 | 5.728e-01-i*8.658e-03 |
| 6 | 1.136e-02+i*1.160e-02 | 8.143e-02+i*6.883e-02 | 2.913e-01-i*1.511e-02 | 6.272e-01-i*5.372e-02 |
| 6 | 2.069e-02+i*1.008e-02 | 2.145e-02+i*1.081e-02 | 2.880e-01+i*2.851e-03 | 6.905e-01-i*1.366e-02 |
| 6 | 1.650e-02-i*1.497e-03 | 2.441e-02-i*2.653e-03 | 1.226e-01+i*4.388e-03 | 8.530e-01-i*1.734e-03 |

$d = 13$, $n_p = 37$, type $[1, 4, 4]$, quality CC

| | | | | |
|---|---|---|---|---|
| 1 | 7.283e-02+i*1.314e-02 | 3.333333333333333e-01 | 3.333333333333333e-01 | 3.333333333333333e-01 |
| 3 | 5.677e-02-i*9.421e-03 | 1.422e-01-i*1.158e-02 | 4.289e-01+i*5.792e-03 | 4.289e-01+i*5.792e-03 |
| 3 | 2.769e-02-i*1.683e-03 | 2.581e-02-i*2.143e-03 | 4.871e-01+i*1.072e-03 | 4.871e-01+i*1.072e-03 |
| 3 | 3.181e-02+i*2.865e-03 | 7.604e-01-i*2.022e-02 | 1.198e-01+i*1.011e-02 | 1.198e-01+i*1.011e-02 |
| 3 | 7.536e-03-i*7.608e-04 | 9.516e-01+i*2.688e-03 | 2.418e-02-i*1.344e-03 | 2.418e-02-i*1.344e-03 |
| 6 | 4.407e-02+i*2.249e-02 | 1.581e-01-i*3.469e-02 | 2.692e-01+i*2.603e-02 | 5.728e-01+i*8.658e-03 |
| 6 | 1.136e-02-i*1.160e-02 | 8.143e-02-i*6.883e-02 | 2.913e-01+i*1.511e-02 | 6.272e-01+i*5.372e-02 |
| 6 | 2.069e-02-i*1.008e-02 | 2.145e-02-i*1.081e-02 | 2.880e-01-i*2.851e-03 | 6.905e-01+i*1.366e-02 |
| 6 | 1.650e-02+i*1.497e-03 | 2.441e-02+i*2.653e-03 | 1.226e-01-i*4.388e-03 | 8.530e-01+i*1.734e-03 |

$d = 13$, $n_p = 37$, type $[1, 4, 4]$, quality CC

| | | | | |
|---|---|---|---|---|
| 1 | 7.783e-02-i*9.000e-03 | 3.333333333333333e-01 | 3.333333333333333e-01 | 3.333333333333333e-01 |
| 3 | 5.481e-02+i*2.010e-02 | 5.929e-01-i*2.442e-02 | 2.035e-01+i*1.221e-02 | 2.035e-01+i*1.221e-02 |
| 3 | 2.860e-02-i*2.140e-04 | 2.626e-02+i*4.939e-04 | 4.869e-01-i*2.470e-04 | 4.869e-01-i*2.470e-04 |
| 3 | 2.805e-02-i*1.390e-03 | 7.615e-01+i*2.638e-02 | 1.193e-01-i*1.319e-02 | 1.193e-01-i*1.319e-02 |
| 3 | 7.024e-03+i*1.185e-03 | 9.533e-01-i*4.474e-03 | 2.337e-02+i*2.237e-03 | 2.337e-02+i*2.237e-03 |
| 6 | 4.466e-02-i*1.691e-02 | 1.443e-01+i*4.092e-03 | 3.458e-01+i*2.854e-02 | 5.100e-01-i*3.264e-02 |
| 6 | 3.005e-02+i*1.256e-02 | 2.902e-02+i*1.396e-02 | 2.828e-01+i*2.618e-03 | 6.882e-01-i*1.657e-02 |
| 6 | 2.702e-03-i*2.121e-03 | 3.140e-02+i*8.875e-02 | 2.859e-01-i*8.828e-03 | 6.827e-01-i*7.992e-02 |
| 6 | 1.704e-02-i*1.875e-03 | 2.566e-02-i*3.099e-03 | 1.194e-01+i*6.187e-03 | 8.549e-01-i*3.088e-03 |

$d = 13$, $n_p = 37$, type $[1, 4, 4]$, quality CC

| | | | | |
|---|---|---|---|---|
| 1 | 7.783e-02+i*9.000e-03 | 3.333333333333333e-01 | 3.333333333333333e-01 | 3.333333333333333e-01 |
| 3 | 5.481e-02-i*2.010e-02 | 5.929e-01+i*2.442e-02 | 2.035e-01-i*1.221e-02 | 2.035e-01-i*1.221e-02 |
| 3 | 2.860e-02+i*2.140e-04 | 2.626e-02-i*4.939e-04 | 4.869e-01+i*2.470e-04 | 4.869e-01+i*2.470e-04 |
| 3 | 2.805e-02+i*1.390e-03 | 7.615e-01-i*2.638e-02 | 1.193e-01+i*1.319e-02 | 1.193e-01+i*1.319e-02 |
| 3 | 7.024e-03-i*1.185e-03 | 9.533e-01+i*4.474e-03 | 2.337e-02-i*2.237e-03 | 2.337e-02-i*2.237e-03 |
| 6 | 4.466e-02+i*1.691e-02 | 1.443e-01-i*4.092e-03 | 3.458e-01-i*2.854e-02 | 5.100e-01+i*3.264e-02 |
| 6 | 3.005e-02-i*1.256e-02 | 2.902e-02-i*1.396e-02 | 2.828e-01-i*2.618e-03 | 6.882e-01+i*1.657e-02 |
| 6 | 2.702e-03+i*2.121e-03 | 3.140e-02-i*8.875e-02 | 2.859e-01+i*8.828e-03 | 6.827e-01+i*7.992e-02 |
| 6 | 1.704e-02+i*1.875e-03 | 2.566e-02+i*3.099e-03 | 1.194e-01-i*6.187e-03 | 8.549e-01+i*3.088e-03 |

$d = 13$, $n_p = 37$, type $[1, 4, 4]$, quality CC

| | | | | |
|---|---|---|---|---|
| 1 | 7.919266891864734e-02 | 3.333333333333333e-01 | 3.333333333333333e-01 | 3.333333333333333e-01 |
| 3 | 6.762098292156684e-02 | 1.328043002600861e-01 | 4.335978498699569e-01 | 4.335978498699569e-01 |
| 3 | 6.714910115056593e-02 | 5.790606069300059e-01 | 2.104696965349970e-01 | 2.104696965349970e-01 |
| 3 | 3.719232922218045e-02 | 2.592098906699400e-02 | 4.870395054665030e-01 | 4.870395054665030e-01 |
| 3 | 2.294777170984416e-02 | 9.168298407893882e-01 | 4.158507960530589e-02 | 4.158507960530589e-02 |
| 6 | 5.264659146749711e-02 | 5.624850804281010e-02 | 2.149827024218964e-01 | 7.287687895352935e-01 |
| 6 | 3.392007174430577e-03 | -2.056379346579599e-02 | 2.258825366969561e-01 | 7.946812567688399e-01 |
| 6 | -1.290e-05-i*8.244e-06 | 4.009e-02+i*9.282e-03 | 5.990e-02-i*3.629e-01 | 9.000e-01+i*3.536e-01 |
| 6 | -1.290e-05+i*8.244e-06 | 4.009e-02-i*9.282e-03 | 5.990e-02+i*3.629e-01 | 9.000e-01-i*3.536e-01 |

$d = 13$, $n_p = 37$, type $[1, 4, 4]$, quality CC

| | | | | |
|---|---|---|---|---|
| 1 | 8.041495715078091e-02 | 3.333333333333333e-01 | 3.333333333333333e-01 | 3.333333333333333e-01 |
| 3 | 9.326413732109834e-02 | 1.478963157093126e-01 | 4.260518421453437e-01 | 4.260518421453437e-01 |
| 3 | 7.490407815152348e-02 | 6.675903265959551e-01 | 1.662048367020225e-01 | 1.662048367020225e-01 |
| 3 | 1.237866375782164e-02 | 9.382804785126661e-01 | 3.085976074366695e-02 | 3.085976074366695e-02 |
| 3 | 2.667870098539202e-07 | -3.472862308318017e-01 | 6.736431154159008e-01 | 6.736431154159008e-01 |
| 6 | 3.576574811191508e-02 | 3.022249786928454e-02 | 3.644069363843497e-01 | 6.053705657463657e-01 |
| 6 | 2.757506052806151e-02 | 3.106675790674559e-02 | 1.580160483976066e-01 | 8.109171936956478e-01 |
| 6 | -1.751e-04-i*3.411e-05 | 1.292e-01+i*1.388e-02 | 3.503e-01-i*3.719e-01 | 5.205e-01+i*3.580e-01 |
| 6 | -1.751e-04+i*3.411e-05 | 1.292e-01-i*1.388e-02 | 3.503e-01+i*3.719e-01 | 5.205e-01-i*3.580e-01 |

$d = 13$, $n_p = 37$, type $[1, 4, 4]$, quality CC

| | | | | |
|---|---|---|---|---|
| 1 | 9.262e-02+i*1.222e-02 | 3.333333333333333e-01 | 3.333333333333333e-01 | 3.333333333333333e-01 |
| 3 | 5.610e-02-i*3.618e-02 | 1.546e-01-i*1.428e-02 | 4.227e-01+i*7.139e-03 | 4.227e-01+i*7.139e-03 |
| 3 | 3.976e-02+i*1.987e-02 | 7.373e-01-i*6.381e-02 | 1.314e-01+i*3.191e-02 | 1.314e-01+i*3.191e-02 |
| 3 | 1.214e-02+i*2.635e-03 | 9.389e-01-i*6.998e-03 | 3.055e-02+i*3.499e-03 | 3.055e-02+i*3.499e-03 |
| 3 | -4.731e-08-i*4.638e-08 | -2.404e-01-i*4.940e-01 | 6.202e-01+i*2.470e-01 | 6.202e-01+i*2.470e-01 |
| 6 | 4.139e-02+i*2.587e-03 | 1.465e-01+i*1.176e-02 | 2.763e-01+i*6.315e-02 | 5.772e-01-i*7.491e-02 |
| 6 | 3.342e-02-i*3.860e-03 | 2.875e-02-i*2.026e-03 | 3.696e-01+i*7.610e-03 | 6.016e-01-i*5.585e-03 |
| 6 | 2.234e-02+i*6.121e-03 | 2.468e-02+i*6.457e-03 | 1.597e-01+i*1.066e-02 | 8.156e-01-i*1.712e-02 |
| 6 | 7.364e-05-i*4.433e-05 | 6.197e-02+i*3.123e-02 | 1.428e-01+i*2.752e-01 | 7.953e-01-i*3.065e-01 |

$d = 13$, $n_p = 37$, type $[1, 4, 4]$, quality CC

| | | | | |
|---|---|---|---|---|
| 1 | 9.262e-02-i*1.222e-02 | 3.333333333333333e-01 | 3.333333333333333e-01 | 3.333333333333333e-01 |
| 3 | 5.610e-02+i*3.618e-02 | 1.546e-01+i*1.428e-02 | 4.227e-01-i*7.139e-03 | 4.227e-01-i*7.139e-03 |
| 3 | 3.976e-02-i*1.987e-02 | 7.373e-01+i*6.381e-02 | 1.314e-01-i*3.191e-02 | 1.314e-01-i*3.191e-02 |
| 3 | 1.214e-02-i*2.635e-03 | 9.389e-01+i*6.998e-03 | 3.055e-02-i*3.499e-03 | 3.055e-02-i*3.499e-03 |
| 3 | -4.731e-08+i*4.638e-08 | -2.404e-01+i*4.940e-01 | 6.202e-01-i*2.470e-01 | 6.202e-01-i*2.470e-01 |
| 6 | 4.139e-02-i*2.587e-03 | 1.465e-01-i*1.176e-02 | 2.763e-01-i*6.315e-02 | 5.772e-01+i*7.491e-02 |
| 6 | 3.342e-02+i*3.860e-03 | 2.875e-02+i*2.026e-03 | 3.696e-01-i*7.610e-03 | 6.016e-01+i*5.585e-03 |
| 6 | 2.234e-02-i*6.121e-03 | 2.468e-02-i*6.457e-03 | 1.597e-01-i*1.066e-02 | 8.156e-01+i*1.712e-02 |
| 6 | 7.364e-05+i*4.433e-05 | 6.197e-02-i*3.123e-02 | 1.428e-01-i*2.752e-01 | 7.953e-01+i*3.065e-01 |

$d = 13$, $n_p = 37$, type $[1, 4, 4]$, quality CC

| | | | | |
|---|---|---|---|---|
| 1 | 1.842111205608723e-01 | 3.333333333333333e-01 | 3.333333333333333e-01 | 3.333333333333333e-01 |
| 3 | 8.440379022874152e-02 | 6.039814756606795e-01 | 1.980092621696602e-01 | 1.980092621696602e-01 |
| 3 | 1.404179059659796e-02 | 9.338810704303560e-01 | 3.305946478482202e-02 | 3.305946478482202e-02 |
| 3 | 9.862e-03+i*1.740e-02 | 1.573e-01+i*9.896e-02 | 4.214e-01-i*4.948e-02 | 4.214e-01-i*4.948e-02 |
| 3 | 9.862e-03-i*1.740e-02 | 1.573e-01-i*9.896e-02 | 4.214e-01+i*4.948e-02 | 4.214e-01+i*4.948e-02 |
| 6 | 4.137009218267099e-02 | 3.497001690425307e-02 | 3.702422590351511e-01 | 5.947877240605959e-01 |
| 6 | 3.550257306007979e-02 | 4.091877188890895e-02 | 1.657492736286540e-01 | 7.933319544824370e-01 |
| 6 | 7.890795315702297e-06 | -2.143952736372467e-01 | 1.529464844872490e-01 | 1.061448789149998e+00 |
| 6 | -8.198329242509033e-07 | 3.309e-01-i*5.946e-01 | 3.309e-01+i*5.946e-01 | 3.381066910864813e-01 |

$d = 13$, $n_p = 37$, type $[1, 4, 4]$, quality CC

| | | | | |
|---|---|---|---|---|
| 1 | 8.659e-02-i*1.473e-02 | 3.333333333333333e-01 | 3.333333333333333e-01 | 3.333333333333333e-01 |
| 3 | 6.392e-02-i*8.183e-03 | 1.322e-01-i*7.228e-03 | 4.339e-01+i*3.614e-03 | 4.339e-01+i*3.614e-03 |
| 3 | 5.216e-02-i*2.206e-02 | 5.721e-01-i*7.060e-02 | 2.139e-01+i*3.530e-02 | 2.139e-01+i*3.530e-02 |
| 3 | 1.879e-02-i*3.294e-03 | 8.494e-01+i*2.525e-02 | 7.532e-02-i*1.263e-02 | 7.532e-02-i*1.263e-02 |
| 3 | 9.284e-03-i*2.451e-03 | 9.451e-01+i*7.921e-03 | 2.746e-02-i*3.960e-03 | 2.746e-02-i*3.960e-03 |
| 6 | 2.830e-02+i*5.868e-04 | 2.530e-02-i*1.240e-04 | 3.759e-01-i*3.565e-03 | 5.988e-01+i*3.690e-03 |
| 6 | 4.053e-02+i*9.566e-03 | 9.023e-02+i*3.937e-02 | 2.121e-01+i*4.786e-03 | 6.977e-01-i*4.415e-02 |
| 6 | 1.132e-02+i*1.029e-02 | 1.223e-02+i*1.957e-02 | 1.746e-01+i*6.344e-03 | 8.132e-01-i*2.591e-02 |
| 6 | -5.885e-07+i*3.018e-06 | -1.915e-01-i*2.847e-03 | 9.697e-02+i*1.201e-01 | 1.095e+00-i*1.173e-01 |

$d = 13$, $n_p = 37$, type $[1, 4, 4]$, quality CC

| | | | | |
|---|---|---|---|---|
| 1 | 8.659e-02+i*1.473e-02 | 3.333333333333333e-01 | 3.333333333333333e-01 | 3.333333333333333e-01 |
| 3 | 6.392e-02+i*8.183e-03 | 1.322e-01+i*7.228e-03 | 4.339e-01-i*3.614e-03 | 4.339e-01-i*3.614e-03 |
| 3 | 5.216e-02+i*2.206e-02 | 5.721e-01+i*7.060e-02 | 2.139e-01-i*3.530e-02 | 2.139e-01-i*3.530e-02 |
| 3 | 1.879e-02+i*3.294e-03 | 8.494e-01-i*2.525e-02 | 7.532e-02+i*1.263e-02 | 7.532e-02+i*1.263e-02 |
| 3 | 9.284e-03+i*2.451e-03 | 9.451e-01-i*7.921e-03 | 2.746e-02+i*3.960e-03 | 2.746e-02+i*3.960e-03 |
| 6 | 2.830e-02-i*5.868e-04 | 2.530e-02+i*1.240e-04 | 3.759e-01+i*3.565e-03 | 5.988e-01-i*3.690e-03 |
| 6 | 4.053e-02-i*9.566e-03 | 9.023e-02-i*3.937e-02 | 2.121e-01-i*4.786e-03 | 6.977e-01+i*4.415e-02 |
| 6 | 1.132e-02-i*1.029e-02 | 1.223e-02-i*1.957e-02 | 1.746e-01-i*6.344e-03 | 8.132e-01+i*2.591e-02 |
| 6 | -5.885e-07-i*3.018e-06 | -1.915e-01+i*2.847e-03 | 9.697e-02-i*1.201e-01 | 1.095e+00+i*1.173e-01 |

$d = 13$, $n_p = 37$, type $[1, 4, 4]$, quality CC

| | | | | |
|---|---|---|---|---|
| 1 | 8.636025156543955e-02 | 3.333333333333333e-01 | 3.333333333333333e-01 | 3.333333333333333e-01 |
| 3 | 3.906373431437603e-02 | 3.082726668253919e-02 | 4.845863666587304e-01 | 4.845863666587304e-01 |
| 3 | 4.436784809196691e-02 | 7.562402837782593e-01 | 1.218798581108703e-01 | 1.218798581108703e-01 |
| 3 | 1.652138082964800e-02 | 9.321499571814929e-01 | 3.392502140925355e-02 | 3.392502140925355e-02 |
| 3 | 2.884273339401765e-12 | -1.461810166344774e+00 | 1.230905083172387e+00 | 1.230905083172387e+00 |
| 6 | 6.968498266864900e-02 | 1.449119029168101e-01 | 3.119378911596087e-01 | 5.431502059235812e-01 |
| 6 | 3.281513547598445e-02 | 2.377956244579305e-02 | 2.318648777735211e-01 | 7.443555597806859e-01 |
| 6 | -1.017e-04-i*3.494e-04 | -1.082e-03-i*6.877e-03 | 1.269e-01-i*1.658e-01 | 8.742e-01+i*1.727e-01 |
| 6 | -1.017e-04+i*3.494e-04 | -1.082e-03+i*6.877e-03 | 1.269e-01+i*1.658e-01 | 8.742e-01-i*1.727e-01 |

$d = 13$, $n_p = 37$, type $[1, 4, 4]$, quality CC

| | | | | |
|---|---|---|---|---|
| 1 | -3.023865007819504e-01 | 3.333333333333333e-01 | 3.333333333333333e-01 | 3.333333333333333e-01 |
| 3 | 4.918560572699650e-02 | 7.066305399255854e-01 | 1.466847300372073e-01 | 1.466847300372073e-01 |
| 3 | 1.397432214805221e-02 | 9.340614102695140e-01 | 3.296929486524299e-02 | 3.296929486524299e-02 |
| 3 | 6.998e-02+i*1.340e-02 | 2.740e-01+i*6.782e-02 | 3.630e-01-i*3.391e-02 | 3.630e-01-i*3.391e-02 |
| 3 | 6.998e-02-i*1.340e-02 | 2.740e-01-i*6.782e-02 | 3.630e-01+i*3.391e-02 | 3.630e-01+i*3.391e-02 |
| 6 | 6.230551972973326e-02 | 1.269310794380879e-01 | 3.359488489380662e-01 | 5.371200716238459e-01 |
| 6 | 2.741649945183694e-02 | 2.336983803975973e-02 | 3.719492422633747e-01 | 6.046809196968655e-01 |
| 6 | 2.578415826600292e-02 | 2.888503629056402e-02 | 1.654151167571881e-01 | 8.056998469522478e-01 |
| 6 | 1.774787838692892e-11 | -1.201697321579604e+00 | 7.059391165924179e-02 | 2.131103409920362e+00 |

$d = 13$, $n_p = 37$, type $[1, 4, 4]$, quality CC

| | | | | |
|---|---|---|---|---|
| 1 | -5.680e-02-i*7.159e-02 | 3.333333333333333e-01 | 3.333333333333333e-01 | 3.333333333333333e-01 |
| 3 | 7.788e-02+i*2.059e-02 | 4.280e-01-i*2.042e-02 | 2.860e-01+i*1.021e-02 | 2.860e-01+i*1.021e-02 |
| 3 | -1.188e-03-i*3.051e-04 | 1.101e-01+i*1.123e-01 | 4.450e-01-i*5.615e-02 | 4.450e-01-i*5.615e-02 |
| 3 | 4.922e-02-i*4.623e-04 | 7.082e-01+i*7.277e-04 | 1.459e-01-i*3.638e-04 | 1.459e-01-i*3.638e-04 |
| 3 | 1.386e-02+i*1.571e-05 | 9.344e-01-i*4.047e-05 | 3.282e-02+i*2.024e-05 | 3.282e-02+i*2.024e-05 |
| 6 | 5.541e-02+i*4.856e-04 | 1.161e-01+i*5.953e-03 | 3.373e-01-i*4.439e-03 | 5.465e-01-i*1.514e-03 |
| 6 | 2.534e-02+i*1.560e-03 | 2.148e-02+i*1.372e-03 | 3.724e-01-i*1.021e-04 | 6.061e-01-i*1.269e-03 |
| 6 | 2.550e-02-i*3.034e-05 | 2.855e-02-i*4.037e-05 | 1.650e-01+i*9.581e-05 | 8.065e-01-i*5.545e-05 |
| 6 | 2.864e-13+i*3.126e-13 | -1.782e+00+i*1.524e-01 | 6.769e-02+i*6.485e-04 | 2.714e+00-i*1.531e-01 |

$d = 13$, $n_p = 37$, type $[1, 4, 4]$, quality CC

| | | | | |
|---|---|---|---|---|
| 1 | -5.680e-02+i*7.159e-02 | 3.333333333333333e-01 | 3.333333333333333e-01 | 3.333333333333333e-01 |
| 3 | 7.788e-02-i*2.059e-02 | 4.280e-01+i*2.042e-02 | 2.860e-01-i*1.021e-02 | 2.860e-01-i*1.021e-02 |
| 3 | -1.188e-03+i*3.051e-04 | 1.101e-01-i*1.123e-01 | 4.450e-01+i*5.615e-02 | 4.450e-01+i*5.615e-02 |
| 3 | 4.922e-02+i*4.623e-04 | 7.082e-01-i*7.277e-04 | 1.459e-01+i*3.638e-04 | 1.459e-01+i*3.638e-04 |
| 3 | 1.386e-02-i*1.571e-05 | 9.344e-01+i*4.047e-05 | 3.282e-02-i*2.024e-05 | 3.282e-02-i*2.024e-05 |
| 6 | 5.541e-02-i*4.856e-04 | 1.161e-01-i*5.953e-03 | 3.373e-01+i*4.439e-03 | 5.465e-01+i*1.514e-03 |
| 6 | 2.534e-02-i*1.560e-03 | 2.148e-02-i*1.372e-03 | 3.724e-01+i*1.021e-04 | 6.061e-01+i*1.269e-03 |
| 6 | 2.550e-02+i*3.034e-05 | 2.855e-02+i*4.037e-05 | 1.650e-01-i*9.581e-05 | 8.065e-01+i*5.545e-05 |
| 6 | 2.864e-13-i*3.126e-13 | -1.782e+00-i*1.524e-01 | 6.769e-02-i*6.485e-04 | 2.714e+00+i*1.531e-01 |

$d = 14$, $n_p = 42$, type $[0, 6, 4]$, quality PI

| | | | | |
|---|---|---|---|---|
| 3 | 5.177410450729159e-02 | 4.530449433823227e-01 | 2.734775283088387e-01 | 2.734775283088387e-01 |
| 3 | 3.278835354412535e-02 | 1.647105613190922e-01 | 4.176447193404539e-01 | 4.176447193404539e-01 |
| 3 | 2.188358136942889e-02 | 2.207217927564272e-02 | 4.889639103621786e-01 | 4.889639103621786e-01 |
| 3 | 4.216258873699302e-02 | 6.455889351749131e-01 | 1.772055324125434e-01 | 1.772055324125434e-01 |
| 3 | 1.443369966977667e-02 | 8.764002338182548e-01 | 6.179988309087260e-02 | 6.179988309087260e-02 |
| 3 | 4.923403602400082e-03 | 9.612180775025979e-01 | 1.939096124870105e-02 | 1.939096124870105e-02 |
| 6 | 3.857151078706068e-02 | 9.291624935697182e-02 | 3.368614597963450e-01 | 5.702222908466832e-01 |
| 6 | 1.443630811353384e-02 | 1.464695005565441e-02 | 2.983728821362578e-01 | 6.869801678080878e-01 |
| 6 | 2.466575321256367e-02 | 5.712475740364794e-02 | 1.722666878213556e-01 | 7.706085547749965e-01 |
| 6 | 5.010228838500672e-03 | 1.268330932872025e-03 | 1.189744976969568e-01 | 8.797571713701711e-01 |

$d = 14$, $n_p = 42$, type $[0, 6, 4]$, quality PO

| | | | | |
|---|---|---|---|---|
| 3 | 4.735232219639136e-02 | 4.414528345364719e-01 | 2.792735827317640e-01 | 2.792735827317640e-01 |
| 3 | 4.826291838361207e-02 | 1.423961166444606e-01 | 4.288019416777697e-01 | 4.288019416777697e-01 |
| 3 | 3.776314827295545e-02 | 6.017815081273018e-01 | 1.991092459363491e-01 | 1.991092459363491e-01 |
| 3 | 2.375205305940770e-02 | 3.607408016791399e-02 | 4.819629599160430e-01 | 4.819629599160430e-01 |
| 3 | 3.079286771854907e-02 | 7.853795229280119e-01 | 1.073102385359941e-01 | 1.073102385359941e-01 |
| 3 | 3.683270920271777e-04 | 1.013904596311739e+00 | -6.952298155869309e-03 | -6.952298155869309e-03 |
| 6 | 3.630257798740242e-02 | 8.470855469770665e-02 | 2.861519747012905e-01 | 6.291394706010028e-01 |
| 6 | 1.077550783424831e-02 | 9.826464555983021e-03 | 3.571831462356840e-01 | 6.329903892083330e-01 |
| 6 | 1.677035403716677e-02 | 2.236630267915131e-02 | 1.869165124977385e-01 | 7.907171848231102e-01 |
| 6 | 8.672408446377745e-03 | 1.703778849115937e-02 | 6.284062382845155e-02 | 9.201215876803891e-01 |

$d = 14$, $n_p = 42$, type $[0, 6, 4]$, quality PO

| | | | | |
|---|---|---|---|---|
| 3 | 5.861439939072805e-02 | 4.557182415405124e-01 | 2.721408792297438e-01 | 2.721408792297438e-01 |
| 3 | 4.884049826504986e-02 | 1.333191004129563e-01 | 4.333404497935218e-01 | 4.333404497935218e-01 |
| 3 | 2.283887786452004e-02 | 2.959161837577697e-02 | 4.852041908121115e-01 | 4.852041908121115e-01 |
| 3 | 3.412396308176992e-02 | 6.413511851367721e-01 | 1.793244074316139e-01 | 1.793244074316139e-01 |
| 3 | 2.642216980965235e-02 | 8.117706258014142e-01 | 9.411468709929288e-02 | 9.411468709929288e-02 |
| 3 | 6.107422896840903e-07 | 1.214552664189376e+00 | -1.072763320946880e-01 | -1.072763320946880e-01 |
| 6 | 3.625176712198585e-02 | 8.699984129223626e-02 | 2.821170463378581e-01 | 6.308831123699056e-01 |
| 6 | 1.201806573515757e-02 | 1.265958897078039e-02 | 3.384718637829319e-01 | 6.488685472462877e-01 |
| 6 | 1.663537301706133e-02 | 2.256974409728162e-02 | 1.742861010985593e-01 | 8.031441548041591e-01 |
| 6 | 6.341201215456964e-03 | 1.155510130650972e-02 | 5.131464126414650e-02 | 9.371302574293438e-01 |

$d = 14$, $n_p = 42$, type $[0, 6, 4]$, quality PO

| | | | | |
|---|---|---|---|---|
| 3 | 6.387330903846114e-02 | 4.614560873284399e-01 | 2.692719563357801e-01 | 2.692719563357801e-01 |
| 3 | 4.297238936638888e-02 | 1.313254749215604e-01 | 4.343372625392198e-01 | 4.343372625392198e-01 |
| 3 | 2.446744644521815e-02 | 2.377211683466673e-02 | 4.881139415826666e-01 | 4.881139415826666e-01 |
| 3 | 4.014352343231663e-02 | 6.852460897319853e-01 | 1.573769551340073e-01 | 1.573769551340073e-01 |
| 3 | 9.237240414338262e-03 | 9.458251981070595e-01 | 2.708740094647025e-02 | 2.708740094647025e-02 |
| 3 | 3.179816669351946e-12 | 2.042181643629574e+00 | -5.210908218147870e-01 | -5.210908218147870e-01 |
| 6 | 3.542447579267120e-02 | 9.458334529225215e-02 | 2.982750834975766e-01 | 6.071415712101712e-01 |
| 6 | 1.673378707542202e-02 | 1.735989078957790e-02 | 2.930955436383901e-01 | 6.895445655720320e-01 |
| 6 | 2.393310804664644e-02 | 3.753490449180281e-02 | 1.337341131383630e-01 | 8.287309823698342e-01 |
| 6 | 2.283414019755738e-04 | -5.314442294845679e-02 | 1.130612801274061e-01 | 9.400831428210507e-01 |

$d = 14$, $n_p = 42$, type $[0, 6, 4]$, quality NO

| | | | | |
|---|---|---|---|---|
| 3 | 5.788101798347453e-02 | 2.219200343461749e-01 | 3.890399828269125e-01 | 3.890399828269125e-01 |
| 3 | 5.123776547289575e-02 | 5.704885348973071e-01 | 2.147557325513464e-01 | 2.147557325513464e-01 |
| 3 | 3.784475207462875e-02 | 8.473723827701675e-02 | 4.576313808614916e-01 | 4.576313808614916e-01 |
| 3 | 3.434654328194147e-02 | 7.704201397060418e-01 | 1.147899301469791e-01 | 1.147899301469791e-01 |
| 3 | 1.535937354015345e-03 | 9.852218789044735e-01 | 7.389060547763266e-03 | 7.389060547763266e-03 |
| 3 | -2.536679541790402e-03 | -3.024114828241834e-02 | 5.151205741412092e-01 | 5.151205741412092e-01 |
| 6 | 3.672465344034776e-02 | 7.914526259063815e-02 | 2.962782740484395e-01 | 6.245764633609223e-01 |
| 6 | 1.733448923597091e-02 | 2.183574975289631e-02 | 2.053031250494872e-01 | 7.728611251976165e-01 |
| 6 | 1.051106029591571e-02 | 2.023882221276647e-02 | 7.572712157844160e-02 | 9.040340562087919e-01 |
| 6 | 1.194179538184958e-02 | -4.033488624518524e-04 | 4.172163249104165e-01 | 5.831870239520353e-01 |

$d = 14$, $n_p = 42$, type $[0, 6, 4]$, quality NO

| | | | | |
|---|---|---|---|---|
| 3 | 5.085044617638537e-02 | 2.280031642520815e-01 | 3.859984178739592e-01 | 3.859984178739592e-01 |
| 3 | 4.366322968706157e-02 | 5.511720517318575e-01 | 2.244139741340712e-01 | 2.244139741340712e-01 |
| 3 | 4.082456755206065e-02 | 9.769459204662300e-02 | 4.511527039766885e-01 | 4.511527039766885e-01 |
| 3 | 3.261868662343659e-02 | 7.882039563825111e-01 | 1.058980218087444e-01 | 1.058980218087444e-01 |
| 3 | -2.235050559546006e-01 | 9.099385250458252e-01 | 4.503073747708742e-02 | 4.503073747708742e-02 |
| 3 | 6.633437374925972e-04 | 1.002166935445334e+00 | -1.083467722667213e-03 | -1.083467722667213e-03 |
| 6 | 3.730212846166806e-02 | 9.733652838384453e-02 | 2.652005201803774e-01 | 6.374629514357781e-01 |
| 6 | 1.939844860402404e-02 | 1.907672676909504e-02 | 3.893428309052869e-01 | 5.915804423256181e-01 |
| 6 | 1.641588852706486e-02 | 1.922005212877580e-02 | 2.032107834735713e-01 | 7.775691643976529e-01 |
| 6 | 1.209925921629916e-01 | 3.743283097598675e-02 | 5.221602419890010e-02 | 9.103511448251132e-01 |

$d = 14$, $n_p = 42$, type $[0, 6, 4]$, quality NO

| | | | | |
|---|---|---|---|---|
| 3 | 6.121610118503491e-02 | 4.573599118903699e-01 | 2.713200440548150e-01 | 2.713200440548150e-01 |
| 3 | 5.205493316955565e-02 | 1.262176702793705e-01 | 4.368911648603148e-01 | 4.368911648603148e-01 |
| 3 | 1.625063615460928e-01 | 8.665578449121469e-01 | 6.672107754392655e-02 | 6.672107754392655e-02 |
| 3 | -2.338815316193022e-01 | 8.868533541762545e-01 | 5.657332291187277e-02 | 5.657332291187277e-02 |
| 3 | 5.121565594141744e-05 | -8.251026231623125e-02 | 5.412551311581156e-01 | 5.412551311581156e-01 |
| 3 | 7.330974928007583e-06 | 1.129209896353310e+00 | -6.460494817665493e-02 | -6.460494817665493e-02 |
| 6 | 4.632890957308841e-02 | 1.149650667656872e-01 | 2.411359564992748e-01 | 6.438989767350380e-01 |
| 6 | 2.552006550864898e-02 | 2.669330126921553e-02 | 3.875121054031674e-01 | 5.857945933276171e-01 |
| 6 | 1.650579427617930e-02 | 1.885039399240126e-02 | 2.086373621488192e-01 | 7.725122438587796e-01 |
| 6 | 5.733469185262471e-02 | 3.536745607862866e-02 | 5.851755484756319e-02 | 9.061149890738081e-01 |

$d = 14$, $n_p = 42$, type $[0, 6, 4]$, quality NC

| | | | | |
|---|---|---|---|---|
| 3 | 7.899217337076116e-02 | 2.081491143965518e-01 | 3.959254428017241e-01 | 3.959254428017241e-01 |
| 3 | 5.971258655627905e-02 | 7.005530034316653e-02 | 4.649723498284167e-01 | 4.649723498284167e-01 |
| 3 | 6.395164805579595e-02 | 6.243708111478847e-01 | 1.878145944260576e-01 | 1.878145944260576e-01 |
| 3 | 2.869898328101138e-02 | 8.175001249989955e-01 | 9.124993750050223e-02 | 9.124993750050223e-02 |
| 3 | 7.607142725514389e-03 | 9.517753875360652e-01 | 2.411230623196741e-02 | 2.411230623196741e-02 |
| 3 | 4.584177706862996e-03 | -3.230630826437048e-02 | 5.161531541321852e-01 | 5.161531541321852e-01 |
| 6 | 3.659207623246399e-02 | 4.099927479488294e-02 | 2.701668642812836e-01 | 6.888338609238334e-01 |
| 6 | 9.663296633986364e-03 | 1.068500764878253e-02 | 1.295959073537648e-01 | 8.597190849974527e-01 |
| 6 | -1.324913180057843e-03 | 1.317162657867497e-01 | 4.341e-01-i*1.970e-01 | 4.341e-01+i*1.970e-01 |
| 6 | -3.714886783830432e-05 | -1.204023460334879e-01 | 5.602e-01-i*1.704e-01 | 5.602e-01+i*1.704e-01 |

$d = 14$, $n_p = 42$, type $[0, 6, 4]$, quality NC

| | | | | |
|---|---|---|---|---|
| 3 | 6.036107327619314e-02 | 2.193018628907821e-01 | 3.903490685546090e-01 | 3.903490685546090e-01 |
| 3 | 5.169752309880823e-02 | 5.726767187772525e-01 | 2.136616406113738e-01 | 2.136616406113738e-01 |
| 3 | 3.355576613863322e-02 | 7.330081307802145e-01 | 1.334959346098927e-01 | 1.334959346098927e-01 |
| 3 | 1.506384628636618e-02 | 8.570205475937774e-01 | 7.148972620311129e-02 | 7.148972620311129e-02 |
| 3 | 5.135647976525186e-03 | 9.608216000965490e-01 | 1.958919995172550e-02 | 1.958919995172550e-02 |
| 3 | 1.042684001460524e-02 | -1.064439866516381e-02 | 5.053221993325819e-01 | 5.053221993325819e-01 |
| 6 | 4.533609793115580e-02 | 7.660541053502708e-02 | 3.643363365599871e-01 | 5.590582529049858e-01 |
| 6 | 2.509428583432804e-02 | 3.077337611501881e-02 | 2.413763556891033e-01 | 7.278502681958779e-01 |
| 6 | 8.186605614157225e-03 | 1.183929843892195e-02 | 1.115562742403937e-01 | 8.766044273206843e-01 |
| 6 | -7.067110853998875e-05 | -8.730125789906420e-02 | 5.437e-01-i*1.785e-01 | 5.437e-01+i*1.785e-01 |

$d = 14$, $n_p = 42$, type $[0, 6, 4]$, quality NC

| | | | | |
|---|---|---|---|---|
| 3 | 4.309108217220078e-02 | 4.347362032136069e-01 | 2.826318983931966e-01 | 2.826318983931966e-01 |
| 3 | 4.804430854350398e-02 | 1.467426896235835e-01 | 4.266286551882082e-01 | 4.266286551882082e-01 |
| 3 | 5.802614300546659e-02 | 6.065200990868811e-01 | 1.967399504565595e-01 | 1.967399504565595e-01 |
| 3 | 3.650144799219219e-02 | 7.658947476576926e-01 | 1.170526261711537e-01 | 1.170526261711537e-01 |
| 3 | 3.039237508679500e-03 | 9.715132339923887e-01 | 1.424338300380563e-02 | 1.424338300380563e-02 |
| 3 | 6.460137321847395e-03 | -7.612585320984501e-03 | 5.038062926604923e-01 | 5.038062926604923e-01 |
| 6 | 3.897677796677360e-02 | 5.394095210690680e-02 | 3.585419662804056e-01 | 5.875170816126876e-01 |
| 6 | 1.850052682881061e-02 | 2.110288178165555e-02 | 2.275702241710919e-01 | 7.513268940472525e-01 |
| 6 | 1.184122528171312e-02 | 2.154893672813047e-02 | 8.806764719168290e-02 | 8.903834160801866e-01 |
| 6 | -2.330416825758784e-04 | 1.421e-01-i*1.733e-01 | 1.421e-01+i*1.733e-01 | 7.157745229003832e-01 |

$d = 14$, $n_p = 42$, type $[0, 6, 4]$, quality CC

| | | | | |
|---|---|---|---|---|
| 3 | 1.083e-02-i*7.412e-03 | 3.735e-01-i*1.159e-01 | 3.133e-01+i*5.793e-02 | 3.133e-01+i*5.793e-02 |
| 3 | 6.767e-02+i*9.941e-03 | 1.585e-01+i*1.232e-02 | 4.208e-01-i*6.162e-03 | 4.208e-01-i*6.162e-03 |
| 3 | 7.108e-02-i*2.791e-03 | 5.713e-01+i*4.975e-03 | 2.144e-01-i*2.487e-03 | 2.144e-01-i*2.487e-03 |
| 3 | 3.195e-02+i*1.476e-03 | 3.172e-02+i*1.330e-03 | 4.841e-01-i*6.651e-04 | 4.841e-01-i*6.651e-04 |
| 3 | 3.180e-02+i*9.348e-05 | 7.888e-01-i*2.416e-04 | 1.056e-01+i*1.208e-04 | 1.056e-01+i*1.208e-04 |
| 3 | 8.424e-03+i*3.776e-05 | 9.490e-01-i*1.203e-04 | 2.551e-02+i*6.015e-05 | 2.551e-02+i*6.015e-05 |
| 6 | 4.106e-02+i*7.810e-05 | 5.256e-02-i*2.381e-03 | 2.785e-01+i*1.792e-03 | 6.689e-01+i*5.893e-04 |
| 6 | 1.580e-03-i*7.733e-04 | -2.763e-02-i*1.039e-02 | 3.244e-01+i*5.790e-03 | 7.032e-01+i*4.601e-03 |
| 6 | 1.316e-02+i*2.320e-05 | 1.741e-02-i*3.299e-06 | 1.307e-01+i*2.618e-04 | 8.519e-01-i*2.585e-04 |
| 6 | -6.681e-07-i*5.123e-08 | 2.431e-01+i*1.642e-02 | 3.765e-01-i*5.310e-01 | 3.804e-01+i*5.146e-01 |

$d = 14$, $n_p = 42$, type $[0, 6, 4]$, quality CC

| | | | | |
|---|---|---|---|---|
| 3 | 1.083e-02+i*7.412e-03 | 3.735e-01+i*1.159e-01 | 3.133e-01-i*5.793e-02 | 3.133e-01-i*5.793e-02 |
| 3 | 6.767e-02-i*9.941e-03 | 1.585e-01-i*1.232e-02 | 4.208e-01+i*6.162e-03 | 4.208e-01+i*6.162e-03 |
| 3 | 7.108e-02+i*2.791e-03 | 5.713e-01-i*4.975e-03 | 2.144e-01+i*2.487e-03 | 2.144e-01+i*2.487e-03 |
| 3 | 3.195e-02-i*1.476e-03 | 3.172e-02-i*1.330e-03 | 4.841e-01+i*6.651e-04 | 4.841e-01+i*6.651e-04 |
| 3 | 3.180e-02-i*9.348e-05 | 7.888e-01+i*2.416e-04 | 1.056e-01-i*1.208e-04 | 1.056e-01-i*1.208e-04 |
| 3 | 8.424e-03-i*3.776e-05 | 9.490e-01+i*1.203e-04 | 2.551e-02-i*6.015e-05 | 2.551e-02-i*6.015e-05 |
| 6 | 4.106e-02-i*7.810e-05 | 5.256e-02+i*2.381e-03 | 2.785e-01-i*1.792e-03 | 6.689e-01-i*5.893e-04 |
| 6 | 1.580e-03+i*7.733e-04 | -2.763e-02+i*1.039e-02 | 3.244e-01-i*5.790e-03 | 7.032e-01-i*4.601e-03 |
| 6 | 1.316e-02-i*2.320e-05 | 1.741e-02+i*3.299e-06 | 1.307e-01-i*2.618e-04 | 8.519e-01+i*2.585e-04 |
| 6 | -6.681e-07+i*5.123e-08 | 2.431e-01-i*1.642e-02 | 3.765e-01+i*5.310e-01 | 3.804e-01-i*5.146e-01 |

$d = 14$, $n_p = 42$, type $[0, 6, 4]$, quality CC

| | | | | |
|---|---|---|---|---|
| 3 | 2.285231300346243e-02 | 2.011609950078643e-02 | 4.899419502496068e-01 | 4.899419502496068e-01 |
| 3 | 5.110130602097285e-02 | 6.836637175783202e-01 | 1.581681412108399e-01 | 1.581681412108399e-01 |
| 3 | 1.241853814575278e-01 | 8.367715332951012e-01 | 8.161423335244940e-02 | 8.161423335244940e-02 |
| 3 | 7.773628991513187e-03 | 9.512654374245281e-01 | 2.436728128773595e-02 | 2.436728128773595e-02 |
| 3 | -4.455e-03-i*2.065e-02 | 1.830e-01+i*8.341e-02 | 4.085e-01-i*4.170e-02 | 4.085e-01-i*4.170e-02 |
| 3 | -4.455e-03+i*2.065e-02 | 1.830e-01-i*8.341e-02 | 4.085e-01+i*4.170e-02 | 4.085e-01+i*4.170e-02 |
| 6 | 8.046880476157059e-02 | 1.419380314080090e-01 | 3.529383752682232e-01 | 5.051235933237678e-01 |
| 6 | 2.793994202195584e-02 | 2.901088299196997e-02 | 2.832730838874707e-01 | 6.877160331205593e-01 |
| 6 | 9.670362536879857e-04 | -3.645193780620453e-02 | 1.500916251277416e-01 | 8.863603126784629e-01 |
| 6 | -4.121092061127956e-02 | 8.210e-02-i*2.863e-02 | 8.210e-02+i*2.863e-02 | 8.357981607738939e-01 |

$d = 14$, $n_p = 42$, type $[0, 6, 4]$, quality CC

| | | | | |
|---|---|---|---|---|
| 3 | 5.316e-02-i*3.636e-03 | 2.285e-01+i*1.251e-03 | 3.858e-01-i*6.255e-04 | 3.858e-01-i*6.255e-04 |
| 3 | 4.931e-02-i*5.225e-03 | 5.705e-01-i*2.065e-02 | 2.148e-01+i*1.032e-02 | 2.148e-01+i*1.032e-02 |
| 3 | 2.030e-02+i*2.686e-04 | 1.951e-02+i*4.739e-06 | 4.902e-01-i*2.370e-06 | 4.902e-01-i*2.370e-06 |
| 3 | 2.806e-03-i*6.205e-04 | 7.133e-01-i*1.460e-01 | 1.434e-01+i*7.299e-02 | 1.434e-01+i*7.299e-02 |
| 3 | 4.250e-03-i*6.977e-03 | 8.563e-01+i*6.121e-02 | 7.183e-02-i*3.060e-02 | 7.183e-02-i*3.060e-02 |
| 3 | 7.565e-03-i*1.394e-03 | 9.517e-01+i*4.449e-03 | 2.417e-02-i*2.225e-03 | 2.417e-02-i*2.225e-03 |
| 6 | 4.297e-02+i*4.241e-04 | 9.743e-02+i*1.784e-03 | 3.488e-01-i*5.998e-05 | 5.537e-01-i*1.724e-03 |
| 6 | 1.731e-02+i*1.140e-03 | 1.802e-02+i*1.261e-03 | 2.918e-01-i*2.147e-03 | 6.902e-01+i*8.854e-04 |
| 6 | 3.235e-02+i*7.454e-03 | 7.091e-02+i*5.422e-03 | 1.577e-01-i*1.022e-02 | 7.714e-01+i*4.800e-03 |
| 6 | 5.351e-03-i*2.269e-04 | 1.510e-03-i*1.029e-03 | 1.222e-01+i*9.761e-04 | 8.762e-01+i*5.265e-05 |

$d = 14$, $n_p = 42$, type $[0, 6, 4]$, quality CC

| | | | | |
|---|---|---|---|---|
| 3 | 5.316e-02+i*3.636e-03 | 2.285e-01-i*1.251e-03 | 3.858e-01+i*6.255e-04 | 3.858e-01+i*6.255e-04 |
| 3 | 4.931e-02+i*5.225e-03 | 5.705e-01+i*2.065e-02 | 2.148e-01-i*1.032e-02 | 2.148e-01-i*1.032e-02 |
| 3 | 2.030e-02-i*2.686e-04 | 1.951e-02-i*4.739e-06 | 4.902e-01+i*2.370e-06 | 4.902e-01+i*2.370e-06 |
| 3 | 2.806e-03+i*6.205e-04 | 7.133e-01+i*1.460e-01 | 1.434e-01-i*7.299e-02 | 1.434e-01-i*7.299e-02 |
| 3 | 4.250e-03+i*6.977e-03 | 8.563e-01-i*6.121e-02 | 7.183e-02+i*3.060e-02 | 7.183e-02+i*3.060e-02 |
| 3 | 7.565e-03+i*1.394e-03 | 9.517e-01-i*4.449e-03 | 2.417e-02+i*2.225e-03 | 2.417e-02+i*2.225e-03 |
| 6 | 4.297e-02-i*4.241e-04 | 9.743e-02-i*1.784e-03 | 3.488e-01+i*5.998e-05 | 5.537e-01+i*1.724e-03 |
| 6 | 1.731e-02-i*1.140e-03 | 1.802e-02-i*1.261e-03 | 2.918e-01+i*2.147e-03 | 6.902e-01-i*8.854e-04 |
| 6 | 3.235e-02-i*7.454e-03 | 7.091e-02-i*5.422e-03 | 1.577e-01+i*1.022e-02 | 7.714e-01-i*4.800e-03 |
| 6 | 5.351e-03+i*2.269e-04 | 1.510e-03+i*1.029e-03 | 1.222e-01-i*9.761e-04 | 8.762e-01-i*5.265e-05 |

$d = 14$, $n_p = 42$, type $[0, 6, 4]$, quality CC

| | | | | |
|---|---|---|---|---|
| 3 | 5.891e-02-i*7.859e-03 | 4.499e-01-i*7.215e-03 | 2.750e-01+i*3.607e-03 | 2.750e-01+i*3.607e-03 |
| 3 | -1.395e-04-i*2.757e-04 | 9.788e-02+i*1.801e-01 | 4.511e-01-i*9.006e-02 | 4.511e-01-i*9.006e-02 |
| 3 | 2.201e-02+i*3.081e-03 | 1.964e-02+i*3.141e-03 | 4.902e-01-i*1.571e-03 | 4.902e-01-i*1.571e-03 |
| 3 | 5.258e-02-i*4.593e-03 | 6.873e-01-i*2.255e-03 | 1.564e-01+i*1.128e-03 | 1.564e-01+i*1.128e-03 |
| 3 | 6.417e-02+i*9.827e-03 | 8.263e-01+i*9.065e-03 | 8.685e-02-i*4.533e-03 | 8.685e-02-i*4.533e-03 |
| 3 | 7.537e-03+i*5.558e-05 | 9.519e-01-i*9.778e-05 | 2.406e-02+i*4.889e-05 | 2.406e-02+i*4.889e-05 |
| 6 | 4.983e-02+i*1.908e-03 | 1.156e-01+i*1.100e-02 | 3.495e-01-i*6.968e-03 | 5.349e-01-i*4.028e-03 |
| 6 | 2.450e-02+i*2.080e-03 | 2.551e-02+i*2.120e-03 | 2.832e-01-i*5.618e-04 | 6.913e-01-i*1.558e-03 |
| 6 | -1.320e-02-i*2.047e-03 | 8.891e-02-i*5.765e-02 | 9.650e-02+i*3.525e-02 | 8.146e-01+i*2.240e-02 |
| 6 | 2.998e-03-i*2.059e-03 | -8.120e-03-i*1.263e-02 | 1.314e-01+i*7.368e-03 | 8.767e-01+i*5.261e-03 |

$d = 14$, $n_p = 42$, type $[0, 6, 4]$, quality CC

| | | | | |
|---|---|---|---|---|
| 3 | 5.891e-02+i*7.859e-03 | 4.499e-01+i*7.215e-03 | 2.750e-01-i*3.607e-03 | 2.750e-01-i*3.607e-03 |
| 3 | -1.395e-04+i*2.757e-04 | 9.788e-02-i*1.801e-01 | 4.511e-01+i*9.006e-02 | 4.511e-01+i*9.006e-02 |
| 3 | 2.201e-02-i*3.081e-03 | 1.964e-02-i*3.141e-03 | 4.902e-01+i*1.571e-03 | 4.902e-01+i*1.571e-03 |
| 3 | 5.258e-02+i*4.593e-03 | 6.873e-01+i*2.255e-03 | 1.564e-01-i*1.128e-03 | 1.564e-01-i*1.128e-03 |
| 3 | 6.417e-02-i*9.827e-03 | 8.263e-01-i*9.065e-03 | 8.685e-02+i*4.533e-03 | 8.685e-02+i*4.533e-03 |
| 3 | 7.537e-03-i*5.558e-05 | 9.519e-01+i*9.778e-05 | 2.406e-02-i*4.889e-05 | 2.406e-02-i*4.889e-05 |
| 6 | 4.983e-02-i*1.908e-03 | 1.156e-01-i*1.100e-02 | 3.495e-01+i*6.968e-03 | 5.349e-01+i*4.028e-03 |
| 6 | 2.450e-02-i*2.080e-03 | 2.551e-02-i*2.120e-03 | 2.832e-01+i*5.618e-04 | 6.913e-01+i*1.558e-03 |
| 6 | -1.320e-02+i*2.047e-03 | 8.891e-02+i*5.765e-02 | 9.650e-02-i*3.525e-02 | 8.146e-01-i*2.240e-02 |
| 6 | 2.998e-03+i*2.059e-03 | -8.120e-03+i*1.263e-02 | 1.314e-01-i*7.368e-03 | 8.767e-01-i*5.261e-03 |

$d = 14$, $n_p = 42$, type $[0, 6, 4]$, quality CC

| | | | | |
|---|---|---|---|---|
| 3 | 5.179e-02-i*3.182e-04 | 2.276e-01-i*8.535e-04 | 3.862e-01+i*4.268e-04 | 3.862e-01+i*4.268e-04 |
| 3 | 4.429e-02-i*3.047e-03 | 5.552e-01-i*7.971e-03 | 2.224e-01+i*3.986e-03 | 2.224e-01+i*3.986e-03 |
| 3 | 4.249e-02+i*3.743e-03 | 9.650e-02-i*2.930e-03 | 4.518e-01+i*1.465e-03 | 4.518e-01+i*1.465e-03 |
| 3 | 1.996e-02-i*4.979e-04 | 1.887e-02-i*1.083e-03 | 4.906e-01+i*5.414e-04 | 4.906e-01+i*5.414e-04 |
| 3 | 2.928e-02-i*3.129e-03 | 7.878e-01+i*1.640e-02 | 1.061e-01-i*8.199e-03 | 1.061e-01-i*8.199e-03 |
| 3 | 7.436e-03-i*5.322e-04 | 9.522e-01+i*1.816e-03 | 2.389e-02-i*9.079e-04 | 2.389e-02-i*9.079e-04 |
| 6 | 3.694e-02+i*1.838e-03 | 9.653e-02+i*5.848e-03 | 2.592e-01-i*1.552e-02 | 6.442e-01+i*9.675e-03 |
| 6 | 1.839e-02+i*1.630e-03 | 1.918e-02+i*1.645e-03 | 2.894e-01-i*4.587e-03 | 6.915e-01+i*2.942e-03 |
| 6 | 1.372e-02-i*1.579e-03 | 1.959e-02-i*2.133e-03 | 1.236e-01-i*3.088e-03 | 8.568e-01+i*5.221e-03 |
| 6 | -2.448e-06+i*1.124e-06 | 7.491e-02-i*6.742e-03 | 2.073e-01-i*3.942e-01 | 7.178e-01+i*4.010e-01 |

$d = 14$, $n_p = 42$, type $[0, 6, 4]$, quality CC

| | | | | |
|---|---|---|---|---|
| 3 | 5.179e-02+i*3.182e-04 | 2.276e-01+i*8.535e-04 | 3.862e-01-i*4.268e-04 | 3.862e-01-i*4.268e-04 |
| 3 | 4.429e-02+i*3.047e-03 | 5.552e-01+i*7.971e-03 | 2.224e-01-i*3.986e-03 | 2.224e-01-i*3.986e-03 |
| 3 | 4.249e-02-i*3.743e-03 | 9.650e-02+i*2.930e-03 | 4.518e-01-i*1.465e-03 | 4.518e-01-i*1.465e-03 |
| 3 | 1.996e-02+i*4.979e-04 | 1.887e-02+i*1.083e-03 | 4.906e-01-i*5.414e-04 | 4.906e-01-i*5.414e-04 |
| 3 | 2.928e-02+i*3.129e-03 | 7.878e-01-i*1.640e-02 | 1.061e-01+i*8.199e-03 | 1.061e-01+i*8.199e-03 |
| 3 | 7.436e-03+i*5.322e-04 | 9.522e-01-i*1.816e-03 | 2.389e-02+i*9.079e-04 | 2.389e-02+i*9.079e-04 |
| 6 | 3.694e-02-i*1.838e-03 | 9.653e-02-i*5.848e-03 | 2.592e-01+i*1.552e-02 | 6.442e-01-i*9.675e-03 |
| 6 | 1.839e-02-i*1.630e-03 | 1.918e-02-i*1.645e-03 | 2.894e-01+i*4.587e-03 | 6.915e-01-i*2.942e-03 |
| 6 | 1.372e-02+i*1.579e-03 | 1.959e-02+i*2.133e-03 | 1.236e-01+i*3.088e-03 | 8.568e-01-i*5.221e-03 |
| 6 | -2.448e-06-i*1.124e-06 | 7.491e-02+i*6.742e-03 | 2.073e-01+i*3.942e-01 | 7.178e-01-i*4.010e-01 |

$d = 14$, $n_p = 42$, type $[0, 6, 4]$, quality CC

| | | | | |
|---|---|---|---|---|
| 3 | 9.182e-02-i*2.426e-02 | 5.129e-01+i*3.582e-02 | 2.436e-01-i*1.791e-02 | 2.436e-01-i*1.791e-02 |
| 3 | 5.121e-02+i*3.246e-02 | 1.518e-01+i*3.265e-02 | 4.241e-01-i*1.633e-02 | 4.241e-01-i*1.633e-02 |
| 3 | 3.491e-03+i*4.467e-04 | 3.598e-01-i*2.145e-01 | 3.201e-01+i*1.073e-01 | 3.201e-01+i*1.073e-01 |
| 3 | 2.827e-02+i*2.043e-03 | 2.614e-02+i*1.802e-03 | 4.869e-01-i*9.010e-04 | 4.869e-01-i*9.010e-04 |
| 3 | 3.893e-02-i*9.588e-04 | 7.332e-01+i*2.153e-03 | 1.334e-01-i*1.076e-03 | 1.334e-01-i*1.076e-03 |
| 3 | 7.146e-03+i*7.428e-05 | 9.533e-01-i*2.723e-04 | 2.333e-02+i*1.361e-04 | 2.333e-02+i*1.361e-04 |
| 6 | 3.807e-02-i*4.734e-03 | 3.934e-02-i*6.772e-03 | 2.859e-01+i*5.164e-04 | 6.748e-01+i*6.256e-03 |
| 6 | 3.283e-05-i*1.530e-04 | 6.263e-02-i*2.492e-01 | 3.178e-01-i*3.389e-03 | 6.196e-01+i*2.525e-01 |
| 6 | 1.816e-02-i*4.715e-05 | 2.669e-02-i*8.447e-05 | 1.215e-01+i*4.200e-04 | 8.519e-01-i*3.355e-04 |
| 6 | -2.617e-05+i*3.273e-05 | -1.146e-01-i*1.178e-01 | 2.833e-01-i*1.445e-02 | 8.313e-01+i*1.322e-01 |

$d = 14$, $n_p = 42$, type $[0, 6, 4]$, quality CC

| | | | | |
|---|---|---|---|---|
| 3 | 9.182e-02+i*2.426e-02 | 5.129e-01-i*3.582e-02 | 2.436e-01+i*1.791e-02 | 2.436e-01+i*1.791e-02 |
| 3 | 5.121e-02-i*3.246e-02 | 1.518e-01-i*3.265e-02 | 4.241e-01+i*1.633e-02 | 4.241e-01+i*1.633e-02 |
| 3 | 3.491e-03-i*4.467e-04 | 3.598e-01+i*2.145e-01 | 3.201e-01-i*1.073e-01 | 3.201e-01-i*1.073e-01 |
| 3 | 2.827e-02-i*2.043e-03 | 2.614e-02-i*1.802e-03 | 4.869e-01+i*9.010e-04 | 4.869e-01+i*9.010e-04 |
| 3 | 3.893e-02+i*9.588e-04 | 7.332e-01-i*2.153e-03 | 1.334e-01+i*1.076e-03 | 1.334e-01+i*1.076e-03 |
| 3 | 7.146e-03-i*7.428e-05 | 9.533e-01+i*2.723e-04 | 2.333e-02-i*1.361e-04 | 2.333e-02-i*1.361e-04 |
| 6 | 3.807e-02+i*4.734e-03 | 3.934e-02+i*6.772e-03 | 2.859e-01-i*5.164e-04 | 6.748e-01-i*6.256e-03 |
| 6 | 3.283e-05+i*1.530e-04 | 6.263e-02+i*2.492e-01 | 3.178e-01+i*3.389e-03 | 6.196e-01-i*2.525e-01 |
| 6 | 1.816e-02+i*4.715e-05 | 2.669e-02+i*8.447e-05 | 1.215e-01-i*4.200e-04 | 8.519e-01+i*3.355e-04 |
| 6 | -2.617e-05-i*3.273e-05 | -1.146e-01+i*1.178e-01 | 2.833e-01+i*1.445e-02 | 8.313e-01-i*1.322e-01 |

$d = 14$, $n_p = 42$, type $[0, 6, 4]$, quality CC

| | | | | |
|---|---|---|---|---|
| 3 | 6.071e-02+i*2.938e-03 | 4.527e-01+i*1.688e-03 | 2.737e-01-i*8.441e-04 | 2.737e-01-i*8.441e-04 |
| 3 | -2.077e-02+i*3.316e-02 | 9.382e-02-i*4.427e-02 | 4.531e-01+i*2.213e-02 | 4.531e-01+i*2.213e-02 |
| 3 | 6.798e-03+i*2.477e-02 | 3.871e-02+i*2.825e-02 | 4.806e-01-i*1.412e-02 | 4.806e-01-i*1.412e-02 |
| 3 | 4.831e-02-i*2.028e-05 | 6.536e-01+i*3.849e-03 | 1.732e-01-i*1.924e-03 | 1.732e-01-i*1.924e-03 |
| 3 | 2.345e-02+i*1.902e-04 | 8.335e-01-i*5.141e-04 | 8.325e-02+i*2.570e-04 | 8.325e-02+i*2.570e-04 |
| 3 | 6.538e-03-i*6.625e-05 | 9.552e-01+i*1.750e-04 | 2.242e-02-i*8.751e-05 | 2.242e-02-i*8.751e-05 |
| 6 | 6.410e-02-i*2.885e-02 | 8.857e-02-i*2.647e-03 | 3.908e-01-i*1.675e-02 | 5.207e-01+i*1.940e-02 |
| 6 | 4.042e-03-i*1.009e-03 | -9.410e-03-i*6.445e-03 | 3.509e-01+i*1.837e-02 | 6.585e-01-i*1.192e-02 |
| 6 | 2.815e-02-i*5.099e-04 | 4.251e-02-i*3.427e-03 | 2.338e-01+i*1.776e-03 | 7.237e-01+i*1.652e-03 |
| 6 | 7.863e-03-i*1.195e-04 | 9.240e-03+i*9.822e-05 | 1.193e-01-i*1.496e-03 | 8.715e-01+i*1.398e-03 |

$d = 14$, $n_p = 42$, type $[0, 6, 4]$, quality CC

| | | | | |
|---|---|---|---|---|
| 3 | 6.071e-02-i*2.938e-03 | 4.527e-01-i*1.688e-03 | 2.737e-01+i*8.441e-04 | 2.737e-01+i*8.441e-04 |
| 3 | -2.077e-02-i*3.316e-02 | 9.382e-02+i*4.427e-02 | 4.531e-01-i*2.213e-02 | 4.531e-01-i*2.213e-02 |
| 3 | 6.798e-03-i*2.477e-02 | 3.871e-02-i*2.825e-02 | 4.806e-01+i*1.412e-02 | 4.806e-01+i*1.412e-02 |
| 3 | 4.831e-02+i*2.028e-05 | 6.536e-01-i*3.849e-03 | 1.732e-01+i*1.924e-03 | 1.732e-01+i*1.924e-03 |
| 3 | 2.345e-02-i*1.902e-04 | 8.335e-01+i*5.141e-04 | 8.325e-02-i*2.570e-04 | 8.325e-02-i*2.570e-04 |
| 3 | 6.538e-03+i*6.625e-05 | 9.552e-01-i*1.750e-04 | 2.242e-02+i*8.751e-05 | 2.242e-02+i*8.751e-05 |
| 6 | 6.410e-02+i*2.885e-02 | 8.857e-02+i*2.647e-03 | 3.908e-01+i*1.675e-02 | 5.207e-01-i*1.940e-02 |
| 6 | 4.042e-03+i*1.009e-03 | -9.410e-03+i*6.445e-03 | 3.509e-01-i*1.837e-02 | 6.585e-01+i*1.192e-02 |
| 6 | 2.815e-02+i*5.099e-04 | 4.251e-02+i*3.427e-03 | 2.338e-01-i*1.776e-03 | 7.237e-01-i*1.652e-03 |
| 6 | 7.863e-03+i*1.195e-04 | 9.240e-03-i*9.822e-05 | 1.193e-01+i*1.496e-03 | 8.715e-01-i*1.398e-03 |

$d = 14$, $n_p = 42$, type $[0, 6, 4]$, quality CC

| | | | | |
|---|---|---|---|---|
| 3 | 5.161e-02+i*2.672e-03 | 2.284e-01-i*3.842e-03 | 3.858e-01+i*1.921e-03 | 3.858e-01+i*1.921e-03 |
| 3 | 4.865e-02-i*3.297e-03 | 5.618e-01-i*3.920e-03 | 2.191e-01+i*1.960e-03 | 2.191e-01+i*1.960e-03 |
| 3 | 3.776e-02+i*2.073e-03 | 1.007e-01-i*1.064e-02 | 4.496e-01+i*5.318e-03 | 4.496e-01+i*5.318e-03 |
| 3 | 1.740e-02+i*1.974e-03 | 1.696e-02-i*6.028e-03 | 4.915e-01+i*3.014e-03 | 4.915e-01+i*3.014e-03 |
| 3 | 3.310e-02-i*1.913e-03 | 7.700e-01+i*7.914e-03 | 1.150e-01-i*3.957e-03 | 1.150e-01-i*3.957e-03 |
| 3 | 2.416e-03-i*2.407e-03 | 9.698e-01+i*1.515e-02 | 1.511e-02-i*7.573e-03 | 1.511e-02-i*7.573e-03 |
| 6 | 3.572e-02-i*1.373e-04 | 8.680e-02+i*7.876e-03 | 2.819e-01-i*1.360e-02 | 6.313e-01+i*5.723e-03 |
| 6 | 8.352e-03+i*5.057e-03 | 1.590e-02+i*8.583e-03 | 3.366e-01-i*6.411e-02 | 6.475e-01+i*5.552e-02 |
| 6 | 1.634e-02-i*2.092e-03 | 2.219e-02+i*1.116e-03 | 2.064e-01-i*3.735e-02 | 7.715e-01+i*3.624e-02 |
| 6 | 1.078e-02-i*2.378e-03 | 2.178e-02-i*2.055e-03 | 8.237e-02-i*2.008e-02 | 8.959e-01+i*2.214e-02 |

$d = 14$, $n_p = 42$, type $[0, 6, 4]$, quality CC

| | | | | |
|---|---|---|---|---|
| 3 | 5.161e-02-i*2.672e-03 | 2.284e-01+i*3.842e-03 | 3.858e-01-i*1.921e-03 | 3.858e-01-i*1.921e-03 |
| 3 | 4.865e-02+i*3.297e-03 | 5.618e-01+i*3.920e-03 | 2.191e-01-i*1.960e-03 | 2.191e-01-i*1.960e-03 |
| 3 | 3.776e-02-i*2.073e-03 | 1.007e-01+i*1.064e-02 | 4.496e-01-i*5.318e-03 | 4.496e-01-i*5.318e-03 |
| 3 | 1.740e-02-i*1.974e-03 | 1.696e-02+i*6.028e-03 | 4.915e-01-i*3.014e-03 | 4.915e-01-i*3.014e-03 |
| 3 | 3.310e-02+i*1.913e-03 | 7.700e-01-i*7.914e-03 | 1.150e-01+i*3.957e-03 | 1.150e-01+i*3.957e-03 |
| 3 | 2.416e-03+i*2.407e-03 | 9.698e-01-i*1.515e-02 | 1.511e-02+i*7.573e-03 | 1.511e-02+i*7.573e-03 |
| 6 | 3.572e-02+i*1.373e-04 | 8.680e-02-i*7.876e-03 | 2.819e-01+i*1.360e-02 | 6.313e-01-i*5.723e-03 |
| 6 | 8.352e-03-i*5.057e-03 | 1.590e-02-i*8.583e-03 | 3.366e-01+i*6.411e-02 | 6.475e-01-i*5.552e-02 |
| 6 | 1.634e-02+i*2.092e-03 | 2.219e-02-i*1.116e-03 | 2.064e-01+i*3.735e-02 | 7.715e-01-i*3.624e-02 |
| 6 | 1.078e-02+i*2.378e-03 | 2.178e-02+i*2.055e-03 | 8.237e-02+i*2.008e-02 | 8.959e-01-i*2.214e-02 |

$d = 14$, $n_p = 42$, type $[0, 6, 4]$, quality CC

| | | | | |
|---|---|---|---|---|
| 3 | 6.714775853834737e-02 | 2.145795682524511e-01 | 3.927102158737744e-01 | 3.927102158737744e-01 |
| 3 | 8.893483877930180e-02 | 6.027575580868557e-01 | 1.986212209565721e-01 | 1.986212209565721e-01 |
| 3 | 4.823713249983220e-02 | 7.485479114407030e-01 | 1.257260442796485e-01 | 1.257260442796485e-01 |
| 3 | 2.869452057913410e-03 | 9.732544097719718e-01 | 1.337279511401408e-02 | 1.337279511401408e-02 |
| 3 | -5.741e-03-i*4.567e-03 | 3.103e-02+i*5.439e-02 | 4.845e-01-i*2.719e-02 | 4.845e-01-i*2.719e-02 |
| 3 | -5.741e-03+i*4.567e-03 | 3.103e-02-i*5.439e-02 | 4.845e-01+i*2.719e-02 | 4.845e-01+i*2.719e-02 |
| 6 | 4.841142228832320e-02 | 4.352212175140839e-02 | 3.994784948205347e-01 | 5.569993834280569e-01 |
| 6 | 1.846341376297695e-02 | 2.060267992833075e-02 | 2.305469436319839e-01 | 7.488503764396853e-01 |
| 6 | 1.260462525869242e-02 | 2.246705562433306e-02 | 8.842756550763719e-02 | 8.891053788680297e-01 |
| 6 | -1.066679465858193e-02 | 1.664e-01-i*7.537e-02 | 1.664e-01+i*7.537e-02 | 6.671490996360089e-01 |

$d = 14$, $n_p = 42$, type $[0, 6, 4]$, quality CC

| | | | | |
|---|---|---|---|---|
| 3 | 5.925e-02-i*4.465e-02 | 4.795e-01-i*3.217e-02 | 2.602e-01+i*1.608e-02 | 2.602e-01+i*1.608e-02 |
| 3 | 4.170e-02+i*5.934e-03 | 8.151e-02+i*3.211e-03 | 4.592e-01-i*1.605e-03 | 4.592e-01-i*1.605e-03 |
| 3 | 1.587e-03-i*1.529e-02 | 6.091e-01+i*1.216e-01 | 1.955e-01-i*6.082e-02 | 1.955e-01-i*6.082e-02 |
| 3 | 1.392e-02-i*6.316e-04 | 1.107e-02-i*1.089e-03 | 4.945e-01+i*5.447e-04 | 4.945e-01+i*5.447e-04 |
| 3 | 2.676e-02-i*1.084e-02 | 7.553e-01+i*4.868e-02 | 1.223e-01-i*2.434e-02 | 1.223e-01-i*2.434e-02 |
| 3 | 7.518e-03+i*6.369e-04 | 9.517e-01-i*2.257e-03 | 2.415e-02+i*1.129e-03 | 2.415e-02+i*1.129e-03 |
| 6 | 4.567e-02+i*3.433e-02 | 1.612e-01+i*2.381e-02 | 2.724e-01-i*3.206e-02 | 5.664e-01+i*8.244e-03 |
| 6 | 2.792e-02+i*8.623e-04 | 2.907e-02+i*9.150e-04 | 2.865e-01+i*1.184e-03 | 6.844e-01-i*2.099e-03 |
| 6 | 1.772e-02-i*2.777e-03 | 2.642e-02-i*4.216e-03 | 1.220e-01+i*3.209e-03 | 8.515e-01+i*1.007e-03 |
| 6 | -4.947e-07-i*6.000e-08 | -2.427e-01-i*1.292e-01 | 2.131e-01+i*4.092e-02 | 1.030e+00+i*8.826e-02 |

$d = 14$, $n_p = 42$, type $[0, 6, 4]$, quality CC

| | | | | |
|---|---|---|---|---|
| 3 | 5.925e-02+i*4.465e-02 | 4.795e-01+i*3.217e-02 | 2.602e-01-i*1.608e-02 | 2.602e-01-i*1.608e-02 |
| 3 | 4.170e-02-i*5.934e-03 | 8.151e-02-i*3.211e-03 | 4.592e-01+i*1.605e-03 | 4.592e-01+i*1.605e-03 |
| 3 | 1.587e-03+i*1.529e-02 | 6.091e-01-i*1.216e-01 | 1.955e-01+i*6.082e-02 | 1.955e-01+i*6.082e-02 |
| 3 | 1.392e-02+i*6.316e-04 | 1.107e-02+i*1.089e-03 | 4.945e-01-i*5.447e-04 | 4.945e-01-i*5.447e-04 |
| 3 | 2.676e-02+i*1.084e-02 | 7.553e-01-i*4.868e-02 | 1.223e-01+i*2.434e-02 | 1.223e-01+i*2.434e-02 |
| 3 | 7.518e-03-i*6.369e-04 | 9.517e-01+i*2.257e-03 | 2.415e-02-i*1.129e-03 | 2.415e-02-i*1.129e-03 |
| 6 | 4.567e-02-i*3.433e-02 | 1.612e-01-i*2.381e-02 | 2.724e-01+i*3.206e-02 | 5.664e-01-i*8.244e-03 |
| 6 | 2.792e-02-i*8.623e-04 | 2.907e-02-i*9.150e-04 | 2.865e-01-i*1.184e-03 | 6.844e-01+i*2.099e-03 |
| 6 | 1.772e-02+i*2.777e-03 | 2.642e-02+i*4.216e-03 | 1.220e-01-i*3.209e-03 | 8.515e-01-i*1.007e-03 |
| 6 | -4.947e-07+i*6.000e-08 | -2.427e-01+i*1.292e-01 | 2.131e-01-i*4.092e-02 | 1.030e+00-i*8.826e-02 |

$d = 14$, $n_p = 42$, type $[0, 6, 4]$, quality CC

| | | | | |
|---|---|---|---|---|
| 3 | 4.852e-02+i*1.075e-02 | 2.311e-01+i*1.624e-03 | 3.845e-01-i*8.118e-04 | 3.845e-01-i*8.118e-04 |
| 3 | 2.585e-02+i*3.392e-03 | 5.085e-01+i*6.321e-02 | 2.457e-01-i*3.161e-02 | 2.457e-01-i*3.161e-02 |
| 3 | 4.089e-02+i*1.677e-03 | 9.059e-02+i*3.642e-03 | 4.547e-01-i*1.821e-03 | 4.547e-01-i*1.821e-03 |
| 3 | 1.749e-02+i*9.395e-04 | 1.610e-02+i*1.398e-03 | 4.920e-01-i*6.988e-04 | 4.920e-01-i*6.988e-04 |
| 3 | 3.009e-02-i*1.469e-03 | 7.706e-01+i*1.622e-02 | 1.147e-01-i*8.108e-03 | 1.147e-01-i*8.108e-03 |
| 3 | 7.869e-03+i*2.653e-04 | 9.507e-01-i*8.704e-04 | 2.465e-02+i*4.352e-04 | 2.465e-02+i*4.352e-04 |
| 6 | 4.267e-02-i*4.020e-03 | 1.205e-01-i*1.343e-02 | 2.609e-01-i*6.494e-03 | 6.186e-01+i*1.993e-02 |
| 6 | 2.280e-02-i*2.242e-03 | 2.399e-02-i*2.216e-03 | 2.888e-01+i*2.230e-03 | 6.872e-01-i*1.465e-05 |
| 6 | 1.584e-02-i*1.515e-03 | 2.301e-02-i*2.673e-03 | 1.253e-01+i*2.077e-03 | 8.517e-01+i*5.968e-04 |
| 6 | 1.829e-09-i*5.690e-09 | -3.389e-01-i*4.138e-01 | 2.044e-01+i*3.997e-02 | 1.135e+00+i*3.738e-01 |

$d = 14$, $n_p = 42$, type $[0, 6, 4]$, quality CC

| | | | | |
|---|---|---|---|---|
| 3 | 4.852e-02-i*1.075e-02 | 2.311e-01-i*1.624e-03 | 3.845e-01+i*8.118e-04 | 3.845e-01+i*8.118e-04 |
| 3 | 2.585e-02-i*3.392e-03 | 5.085e-01-i*6.321e-02 | 2.457e-01+i*3.161e-02 | 2.457e-01+i*3.161e-02 |
| 3 | 4.089e-02-i*1.677e-03 | 9.059e-02-i*3.642e-03 | 4.547e-01+i*1.821e-03 | 4.547e-01+i*1.821e-03 |
| 3 | 1.749e-02-i*9.395e-04 | 1.610e-02-i*1.398e-03 | 4.920e-01+i*6.988e-04 | 4.920e-01+i*6.988e-04 |
| 3 | 3.009e-02+i*1.469e-03 | 7.706e-01-i*1.622e-02 | 1.147e-01+i*8.108e-03 | 1.147e-01+i*8.108e-03 |
| 3 | 7.869e-03-i*2.653e-04 | 9.507e-01+i*8.704e-04 | 2.465e-02-i*4.352e-04 | 2.465e-02-i*4.352e-04 |
| 6 | 4.267e-02+i*4.020e-03 | 1.205e-01+i*1.343e-02 | 2.609e-01+i*6.494e-03 | 6.186e-01-i*1.993e-02 |
| 6 | 2.280e-02+i*2.242e-03 | 2.399e-02+i*2.216e-03 | 2.888e-01-i*2.230e-03 | 6.872e-01+i*1.465e-05 |
| 6 | 1.584e-02+i*1.515e-03 | 2.301e-02+i*2.673e-03 | 1.253e-01-i*2.077e-03 | 8.517e-01-i*5.968e-04 |
| 6 | 1.829e-09+i*5.690e-09 | -3.389e-01+i*4.138e-01 | 2.044e-01-i*3.997e-02 | 1.135e+00-i*3.738e-01 |

$d = 14$, $n_p = 42$, type $[0, 6, 4]$, quality CC

| | | | | |
|---|---|---|---|---|
| 3 | 5.546e-02+i*1.056e-02 | 4.459e-01-i*1.077e-03 | 2.771e-01+i*5.383e-04 | 2.771e-01+i*5.383e-04 |
| 3 | 9.806e-03+i*2.276e-05 | 1.898e-01-i*8.129e-02 | 4.051e-01+i*4.064e-02 | 4.051e-01+i*4.064e-02 |
| 3 | 4.437e-02-i*3.088e-03 | 9.668e-02-i*1.149e-02 | 4.517e-01+i*5.745e-03 | 4.517e-01+i*5.745e-03 |
| 3 | 1.870e-02-i*2.443e-03 | 1.726e-02-i*2.283e-03 | 4.914e-01+i*1.142e-03 | 4.914e-01+i*1.142e-03 |
| 3 | 3.106e-02-i*2.308e-03 | 7.625e-01+i*1.694e-02 | 1.187e-01-i*8.471e-03 | 1.187e-01-i*8.471e-03 |
| 3 | 7.747e-03+i*2.448e-04 | 9.511e-01-i*8.359e-04 | 2.444e-02+i*4.179e-04 | 2.444e-02+i*4.179e-04 |
| 6 | 4.348e-02+i*5.841e-04 | 1.231e-01-i*3.028e-03 | 2.658e-01-i*8.758e-03 | 6.111e-01+i*1.179e-02 |
| 6 | 2.310e-02-i*6.856e-04 | 2.424e-02-i*6.460e-04 | 2.884e-01+i*1.345e-03 | 6.874e-01-i*6.986e-04 |
| 6 | 1.652e-02-i*1.391e-03 | 2.414e-02-i*2.326e-03 | 1.244e-01+i*1.630e-03 | 8.514e-01+i*6.958e-04 |
| 6 | 1.032e-09+i*7.315e-09 | -3.991e-01-i*2.727e-01 | 2.035e-01+i*3.555e-02 | 1.196e+00+i*2.372e-01 |

$d = 14$, $n_p = 42$, type $[0, 6, 4]$, quality CC

| | | | | |
|---|---|---|---|---|
| 3 | 5.546e-02-i*1.056e-02 | 4.459e-01+i*1.077e-03 | 2.771e-01-i*5.383e-04 | 2.771e-01-i*5.383e-04 |
| 3 | 9.806e-03-i*2.276e-05 | 1.898e-01+i*8.129e-02 | 4.051e-01-i*4.064e-02 | 4.051e-01-i*4.064e-02 |
| 3 | 4.437e-02+i*3.088e-03 | 9.668e-02+i*1.149e-02 | 4.517e-01-i*5.745e-03 | 4.517e-01-i*5.745e-03 |
| 3 | 1.870e-02+i*2.443e-03 | 1.726e-02+i*2.283e-03 | 4.914e-01-i*1.142e-03 | 4.914e-01-i*1.142e-03 |
| 3 | 3.106e-02+i*2.308e-03 | 7.625e-01-i*1.694e-02 | 1.187e-01+i*8.471e-03 | 1.187e-01+i*8.471e-03 |
| 3 | 7.747e-03-i*2.448e-04 | 9.511e-01+i*8.359e-04 | 2.444e-02-i*4.179e-04 | 2.444e-02-i*4.179e-04 |
| 6 | 4.348e-02-i*5.841e-04 | 1.231e-01+i*3.028e-03 | 2.658e-01+i*8.758e-03 | 6.111e-01-i*1.179e-02 |
| 6 | 2.310e-02+i*6.856e-04 | 2.424e-02+i*6.460e-04 | 2.884e-01-i*1.345e-03 | 6.874e-01+i*6.986e-04 |
| 6 | 1.652e-02+i*1.391e-03 | 2.414e-02+i*2.326e-03 | 1.244e-01-i*1.630e-03 | 8.514e-01-i*6.958e-04 |
| 6 | 1.032e-09-i*7.315e-09 | -3.991e-01+i*2.727e-01 | 2.035e-01-i*3.555e-02 | 1.196e+00-i*2.372e-01 |

$d = 14$, $n_p = 42$, type $[0, 6, 4]$, quality CC

| | | | | |
|---|---|---|---|---|
| 3 | 6.655538852659422e-02 | 4.632212961103579e-01 | 2.683893519448211e-01 | 2.683893519448211e-01 |
| 3 | 5.220617829545808e-02 | 1.202928757073425e-01 | 4.398535621463288e-01 | 4.398535621463288e-01 |
| 3 | 2.090720868338930e-02 | 7.057950590606794e-01 | 1.471024704696603e-01 | 1.471024704696603e-01 |
| 3 | 3.008648317632602e-12 | 2.121412000577328e+00 | -5.607060002886639e-01 | -5.607060002886639e-01 |
| 3 | -6.466e-02+i*5.313e-02 | 9.003e-01+i*1.975e-02 | 4.983e-02-i*9.874e-03 | 4.983e-02-i*9.874e-03 |
| 3 | -6.466e-02-i*5.313e-02 | 9.003e-01-i*1.975e-02 | 4.983e-02+i*9.874e-03 | 4.983e-02+i*9.874e-03 |
| 6 | 3.955565725463123e-02 | 1.044715815256602e-01 | 2.551721990573704e-01 | 6.403562194169694e-01 |
| 6 | 2.263673041332193e-02 | 2.278046433106534e-02 | 3.901123522697470e-01 | 5.871071833991876e-01 |
| 6 | 1.645059605373902e-02 | 1.897272301269352e-02 | 2.062276107651867e-01 | 7.747996662221198e-01 |
| 6 | 8.284452166532539e-02 | 3.667733257270650e-02 | 5.529956693367947e-02 | 9.080231004936140e-01 |

$d = 14$, $n_p = 42$, type $[0, 6, 4]$, quality CC

| | | | | |
|---|---|---|---|---|
| 3 | 4.478e-02-i*7.373e-04 | 2.252e-01-i*1.980e-04 | 3.874e-01+i*9.898e-05 | 3.874e-01+i*9.898e-05 |
| 3 | 3.608e-02+i*3.674e-04 | 5.091e-01-i*2.461e-03 | 2.454e-01+i*1.230e-03 | 2.454e-01+i*1.230e-03 |
| 3 | 3.929e-02+i*1.624e-03 | 9.061e-02+i*1.254e-03 | 4.547e-01-i*6.269e-04 | 4.547e-01-i*6.269e-04 |
| 3 | 1.792e-02+i*8.192e-05 | 1.663e-02+i*1.970e-04 | 4.917e-01-i*9.849e-05 | 4.917e-01-i*9.849e-05 |
| 3 | 3.155e-02-i*1.502e-03 | 7.630e-01+i*1.113e-02 | 1.185e-01-i*5.567e-03 | 1.185e-01-i*5.567e-03 |
| 3 | 7.779e-03+i*1.424e-04 | 9.510e-01-i*4.816e-04 | 2.449e-02+i*2.408e-04 | 2.449e-02+i*2.408e-04 |
| 6 | 3.999e-02+i*1.037e-03 | 1.139e-01+i*2.429e-04 | 2.677e-01-i*6.247e-03 | 6.184e-01+i*6.004e-03 |
| 6 | 2.163e-02-i*8.451e-05 | 2.273e-02-i*4.229e-05 | 2.890e-01+i*9.223e-04 | 6.882e-01-i*8.800e-04 |
| 6 | 1.636e-02-i*9.411e-04 | 2.380e-02-i*1.586e-03 | 1.248e-01+i*1.008e-03 | 8.514e-01+i*5.779e-04 |
| 6 | -1.884e-10+i*8.012e-10 | -5.289e-01-i*3.002e-01 | 2.000e-01+i*3.883e-02 | 1.329e+00+i*2.614e-01 |

$d = 14$, $n_p = 42$, type $[0, 6, 4]$, quality CC

| | | | | |
|---|---|---|---|---|
| 3 | 4.478e-02+i*7.373e-04 | 2.252e-01+i*1.980e-04 | 3.874e-01-i*9.898e-05 | 3.874e-01-i*9.898e-05 |
| 3 | 3.608e-02-i*3.674e-04 | 5.091e-01+i*2.461e-03 | 2.454e-01-i*1.230e-03 | 2.454e-01-i*1.230e-03 |
| 3 | 3.929e-02-i*1.624e-03 | 9.061e-02-i*1.254e-03 | 4.547e-01+i*6.269e-04 | 4.547e-01+i*6.269e-04 |
| 3 | 1.792e-02-i*8.192e-05 | 1.663e-02-i*1.970e-04 | 4.917e-01+i*9.849e-05 | 4.917e-01+i*9.849e-05 |
| 3 | 3.155e-02+i*1.502e-03 | 7.630e-01-i*1.113e-02 | 1.185e-01+i*5.567e-03 | 1.185e-01+i*5.567e-03 |
| 3 | 7.779e-03-i*1.424e-04 | 9.510e-01+i*4.816e-04 | 2.449e-02-i*2.408e-04 | 2.449e-02-i*2.408e-04 |
| 6 | 3.999e-02-i*1.037e-03 | 1.139e-01-i*2.429e-04 | 2.677e-01+i*6.247e-03 | 6.184e-01-i*6.004e-03 |
| 6 | 2.163e-02+i*8.451e-05 | 2.273e-02+i*4.229e-05 | 2.890e-01-i*9.223e-04 | 6.882e-01+i*8.800e-04 |
| 6 | 1.636e-02+i*9.411e-04 | 2.380e-02+i*1.586e-03 | 1.248e-01-i*1.008e-03 | 8.514e-01-i*5.779e-04 |
| 6 | -1.884e-10-i*8.012e-10 | -5.289e-01+i*3.002e-01 | 2.000e-01-i*3.883e-02 | 1.329e+00-i*2.614e-01 |

$d = 14$, $n_p = 42$, type $[0, 6, 4]$, quality CC

| | | | | |
|---|---|---|---|---|
| 3 | 6.464e-02+i*1.387e-04 | 4.602e-01+i*1.542e-04 | 2.699e-01-i*7.712e-05 | 2.699e-01-i*7.712e-05 |
| 3 | 5.350e-02-i*4.681e-04 | 1.188e-01-i*2.127e-04 | 4.406e-01+i*1.063e-04 | 4.406e-01+i*1.063e-04 |
| 3 | 2.264e-02+i*6.278e-03 | 2.347e-02+i*9.013e-04 | 4.883e-01-i*4.507e-04 | 4.883e-01-i*4.507e-04 |
| 3 | 2.487e-02-i*6.850e-04 | 8.059e-01-i*1.048e-02 | 9.703e-02+i*5.240e-03 | 9.703e-02+i*5.240e-03 |
| 3 | 7.089e-03-i*2.665e-03 | 9.527e-01+i*7.569e-03 | 2.367e-02-i*3.784e-03 | 2.367e-02-i*3.784e-03 |
| 3 | -5.437e-19+i*1.117e-18 | -2.750e+00-i*3.087e+00 | 1.875e+00+i*1.543e+00 | 1.875e+00+i*1.543e+00 |
| 6 | 4.460e-02-i*5.264e-04 | 1.130e-01+i*9.047e-06 | 2.440e-01+i*2.097e-03 | 6.430e-01-i*2.106e-03 |
| 6 | 2.253e-02+i*2.880e-03 | 2.257e-02-i*2.005e-03 | 2.982e-01-i*4.415e-02 | 6.793e-01+i*4.616e-02 |
| 6 | 7.006e-04-i*1.205e-03 | 1.574e-02-i*7.979e-03 | 2.085e-01-i*1.466e-01 | 7.758e-01+i*1.546e-01 |
| 6 | 1.246e-02-i*2.448e-03 | 1.841e-02+i*2.784e-03 | 1.181e-01-i*3.230e-02 | 8.634e-01+i*2.951e-02 |

$d = 14$, $n_p = 42$, type $[0, 6, 4]$, quality CC

| | | | | |
|---|---|---|---|---|
| 3 | 6.464e-02-i*1.387e-04 | 4.602e-01-i*1.542e-04 | 2.699e-01+i*7.712e-05 | 2.699e-01+i*7.712e-05 |
| 3 | 5.350e-02+i*4.681e-04 | 1.188e-01+i*2.127e-04 | 4.406e-01-i*1.063e-04 | 4.406e-01-i*1.063e-04 |
| 3 | 2.264e-02-i*6.278e-03 | 2.347e-02-i*9.013e-04 | 4.883e-01+i*4.507e-04 | 4.883e-01+i*4.507e-04 |
| 3 | 2.487e-02+i*6.850e-04 | 8.059e-01+i*1.048e-02 | 9.703e-02-i*5.240e-03 | 9.703e-02-i*5.240e-03 |
| 3 | 7.089e-03+i*2.665e-03 | 9.527e-01-i*7.569e-03 | 2.367e-02+i*3.784e-03 | 2.367e-02+i*3.784e-03 |
| 3 | -5.437e-19-i*1.117e-18 | -2.750e+00+i*3.087e+00 | 1.875e+00-i*1.543e+00 | 1.875e+00-i*1.543e+00 |
| 6 | 4.460e-02+i*5.264e-04 | 1.130e-01-i*9.047e-06 | 2.440e-01-i*2.097e-03 | 6.430e-01+i*2.106e-03 |
| 6 | 2.253e-02-i*2.880e-03 | 2.257e-02+i*2.005e-03 | 2.982e-01+i*4.415e-02 | 6.793e-01-i*4.616e-02 |
| 6 | 7.006e-04+i*1.205e-03 | 1.574e-02+i*7.979e-03 | 2.085e-01+i*1.466e-01 | 7.758e-01-i*1.546e-01 |
| 6 | 1.246e-02+i*2.448e-03 | 1.841e-02-i*2.784e-03 | 1.181e-01+i*3.230e-02 | 8.634e-01-i*2.951e-02 |

$d = 14$, $n_p = 42$, type $[0, 6, 4]$, quality CC

| | | | | |
|---|---|---|---|---|
| 3 | 9.202818815745786e-02 | 1.648332448820461e-01 | 4.175833775589770e-01 | 4.175833775589770e-01 |
| 3 | 4.973076851445317e-19 | 5.662636557538263e+00 | -2.331318278769132e+00 | -2.331318278769132e+00 |
| 3 | 5.949e-03+i*5.505e-03 | 2.866e-01+i*1.614e-01 | 3.567e-01-i*8.070e-02 | 3.567e-01-i*8.070e-02 |
| 3 | 5.949e-03-i*5.505e-03 | 2.866e-01-i*1.614e-01 | 3.567e-01+i*8.070e-02 | 3.567e-01+i*8.070e-02 |
| 3 | -1.738e-02+i*1.857e-02 | 8.965e-01+i*4.047e-02 | 5.177e-02-i*2.024e-02 | 5.177e-02-i*2.024e-02 |
| 3 | -1.738e-02-i*1.857e-02 | 8.965e-01-i*4.047e-02 | 5.177e-02+i*2.024e-02 | 5.177e-02+i*2.024e-02 |
| 6 | 5.070601245015494e-02 | 1.191281676399125e-01 | 2.356976159878156e-01 | 6.451742163722719e-01 |
| 6 | 2.743359747547832e-02 | 2.801967124752020e-02 | 3.901151587546584e-01 | 5.818651699978214e-01 |
| 6 | 1.661990754920317e-02 | 1.889478816839436e-02 | 2.109498070092868e-01 | 7.701554048223189e-01 |
| 6 | 3.732175682303503e-02 | 3.309025188215662e-02 | 6.279217230922883e-02 | 9.041175758086146e-01 |

$d = 15$, $n_p = 46$, type $[1, 7, 4]$, quality NC

| | | | | |
|---|---|---|---|---|
| 1 | 5.080005087265938e-02 | 3.333333333333333e-01 | 3.333333333333333e-01 | 3.333333333333333e-01 |
| 3 | 4.623922103057610e-02 | 1.743675289159769e-01 | 4.128162355420115e-01 | 4.128162355420115e-01 |
| 3 | 4.694672922622666e-02 | 5.412471104399061e-01 | 2.293764447800469e-01 | 2.293764447800469e-01 |
| 3 | 3.186211609251108e-02 | 6.688794735602234e-02 | 4.665560263219888e-01 | 4.665560263219888e-01 |
| 3 | 1.278608910154196e-02 | 1.167289534252281e-02 | 4.941635523287386e-01 | 4.941635523287386e-01 |
| 3 | 3.087881767476850e-02 | 7.731241067247773e-01 | 1.134379466376113e-01 | 1.134379466376113e-01 |
| 3 | 7.839172637427769e-03 | 9.508452007188952e-01 | 2.457739964055241e-02 | 2.457739964055241e-02 |
| 3 | -8.382678869002928e-12 | 1.561675665914419e+00 | -2.808378329572093e-01 | -2.808378329572093e-01 |
| 6 | 3.698630720311791e-02 | 9.551011774161495e-02 | 2.673844140840160e-01 | 6.371054681743691e-01 |
| 6 | 1.763435675193786e-02 | 1.833167917815711e-02 | 2.908598485915191e-01 | 6.908084722303238e-01 |
| 6 | 1.530325468923685e-02 | 2.196486096509650e-02 | 1.255652346728823e-01 | 8.524699043620212e-01 |
| 6 | -4.038783691225615e-13 | 5.844197595868141e-02 | 4.708e-01-i*1.591e+00 | 4.708e-01+i*1.591e+00 |
